# Supplementary material for: Learning Intrinsic Water-Quality Dynamics with Rainfall for Data-Driven Forecasting
Source: arXiv:2508.08279 source file (2026-09-10)
Supplement: Supplementary file 1 [file Appendix-final.tex]

%File: formatting-instruction.tex
\documentclass[letterpaper]{article}
\usepackage{aaai}
\usepackage{amsfonts}
\usepackage{times}
\usepackage{graphicx}
\usepackage{helvet}
\usepackage{courier}
\usepackage{bibentry}
\usepackage{amsmath}
\usepackage{booktabs} 
\usepackage{multirow}
\usepackage{comment}
\usepackage{subfigure}
\usepackage{algorithm}
\usepackage{algorithmic}
\frenchspacing
\setlength{\pdfpagewidth}{8.5in}
\setlength{\pdfpageheight}{11in}
\pdfinfo{
/Title (XXX) %Multidimensional
/Author (Put All Your Authors Here, Separated by Commas)}
\setcounter{secnumdepth}{0}  
 \begin{document}
% The file aaai.sty is the style file for AAAI Press 
% proceedings, working notes, and technical reports.
%
\nocopyright
\title{Supplementary Material for XFMNet: Decoding Cross-Site and Nonstationary Water Patterns via Stepwise Multimodal Fusion for Long-Term Water Quality Forecasting}
% \author{AAAI Press\\
% Association for the Advancement of Artificial Intelligence\\
% 2275 East Bayshore Road, Suite 160\\
% Palo Alto, California 94303\\
% }
\author{Anonymous submission}
\maketitle

This document provides more analysis, implementation details, and experimental results for comparative studies.

\section{Data Analysis}
\subsection{Cross-site Periodic Coupling Analysis} %换成一天一画 线细一点，两个图差异大一点
This section gives a detailed analysis on observed water quality data. We first compute periodograms at one-day resolution over the range of 0 to 30 days for two monitoring stations. It is shown in Fig. \ref{period} that each spectrum is displayed as a power versus period bar chart and overlaid with a LOESS \cite{loess} trend line. Station A exhibits two dominant peaks at one day and around thirty days, indicating highly pure diurnal and monthly oscillations. Station B also shows a strong one-day peak but displays additional, lower-amplitude peaks throughout the 10 to 20 day range, revealing substantial mid-term periodic variability. These pronounced differences in peak magnitude and spectral complexity provide clear evidence of heterogeneous cross-site coupling. Station A’s spectrum peaks sharply at one day and again around thirty days, yielding a clean diurnal and monthly signature with minimal intermediate bumps. Station B also shows a clear one-day rhythm but differs markedly in the ten–twenty-day band, where it displays a series of lower-amplitude peaks that are absent or much weaker in Station A’s profile. This contrast in mid-term periodic content underscores the heterogeneous nature of cross-site coupling and indicates that Station B incorporates more multi-day variability, whereas Station A remains dominated by pure daily and monthly cycles.

We further extract the full time series from both stations, applying two fourth-order Butterworth band-pass filters: one isolating the 0.8–1.2 cycles/day band (daily cycle) and the other isolating the 1/20–1/10 cycles/day band (10–20 day mid-term cycle). Each filtered signal is transformed via the Hilbert analytic signal to compute its instantaneous amplitude envelope. Finally, we plot both envelopes on a common time-index axis at high resolution, using distinct line widths and the colors to differentiate stations. In the daily-cycle envelope plot, two curves overlap perfectly, indicating that the two stations share the same diurnal frequency and exhibit similar phase behavior. In contrast, the 10–20 day envelope reveals pronounced differences. This contrast demonstrates that while daily oscillations are regionally homogeneous, the multiday component varies significantly between sites, providing compelling evidence that cross-site periodic coupling is characterized by strong diurnal synchrony alongside heterogeneous mid-term variability.

\begin{figure}[ht!]
\centering
\includegraphics[width=0.99\columnwidth]{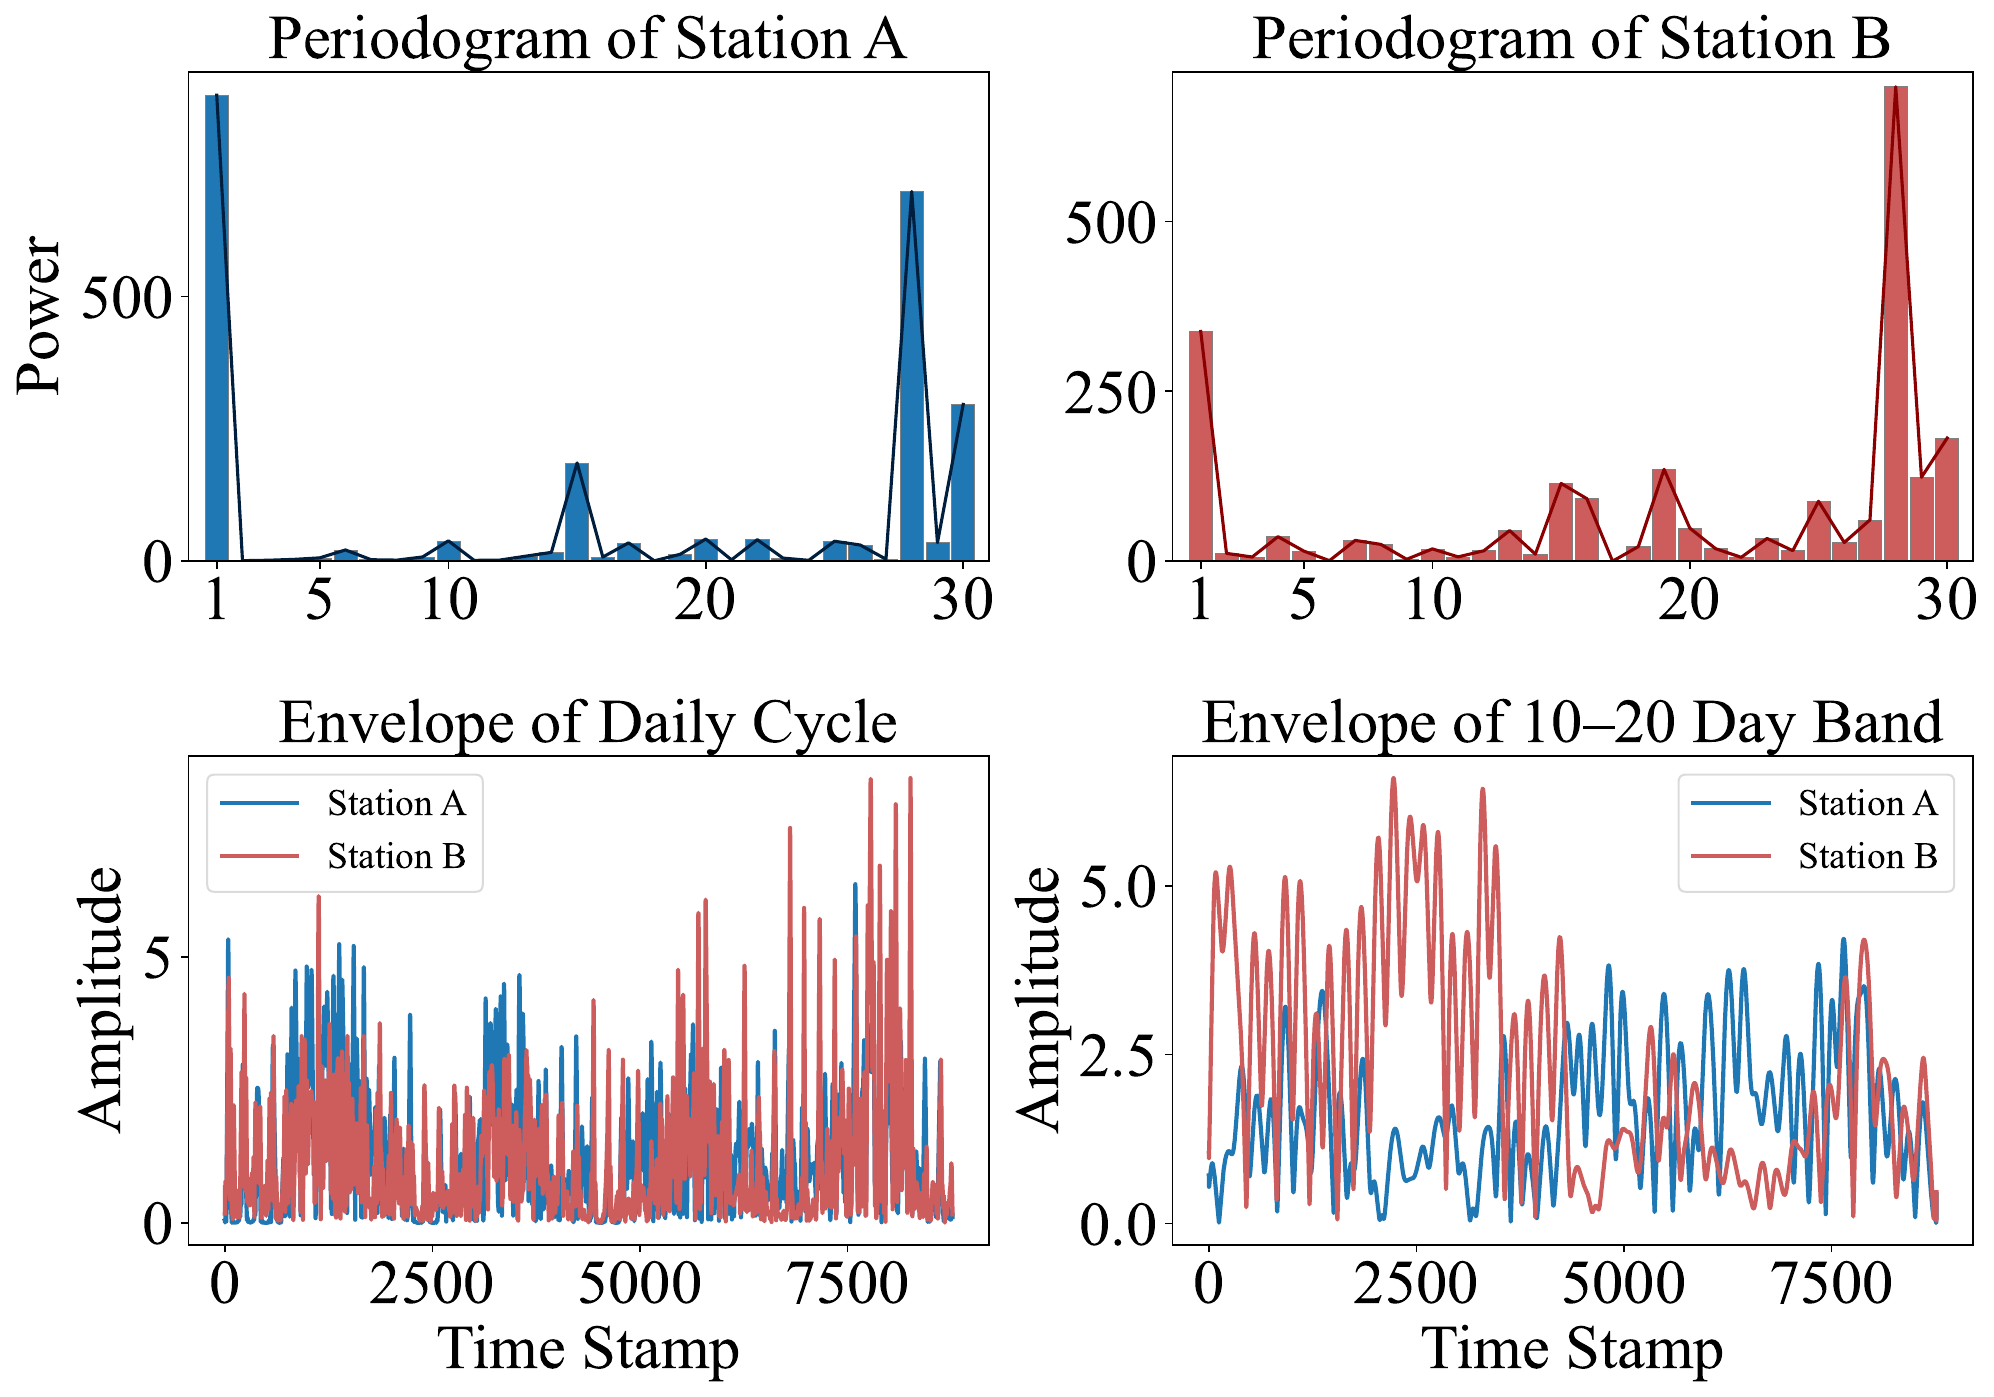} % Reduce the figure size so that it is slightly narrower than the column. Don't use precise values for figure width.This setup will avoid overfull boxes.
\caption{Two-site periodicity analysis: Periodograms show dominant daily and monthly peaks at Station A, while Station B exhibits additional 10–20 day components. Amplitude envelopes indicate similar diurnal dynamics across stations but reveal heterogeneous multi-day variability.}
\label{period}
\end{figure}

\subsection{Stationary and Fluctuation Analysis}
Fig. \ref{station} characterizes long-range dependence and time-varying volatility with environmental factors. First, autocorrelation function (ACF) plots are generated for lags 1-25 with 95\% confidence bounds, allowing quantification of memory effects: a rapid decay implies predominantly short-range dependence, whereas a slow decay reveals significant long-term trend or periodic components. Second, a fixed 48-point rolling window is applied to compute the local standard deviation at each time step, and the distribution of these rolling standard deviations is presented as a histogram. Points that exceed $\pm 3$ rolling standard deviations from the local mean are counted as anomalies. This dual-axis layout simultaneously conveys the baseline fluctuation distribution and the frequency of extreme deviations across different volatility regimes.

\begin{figure}[ht!]
\centering
\includegraphics[width=0.99\columnwidth]{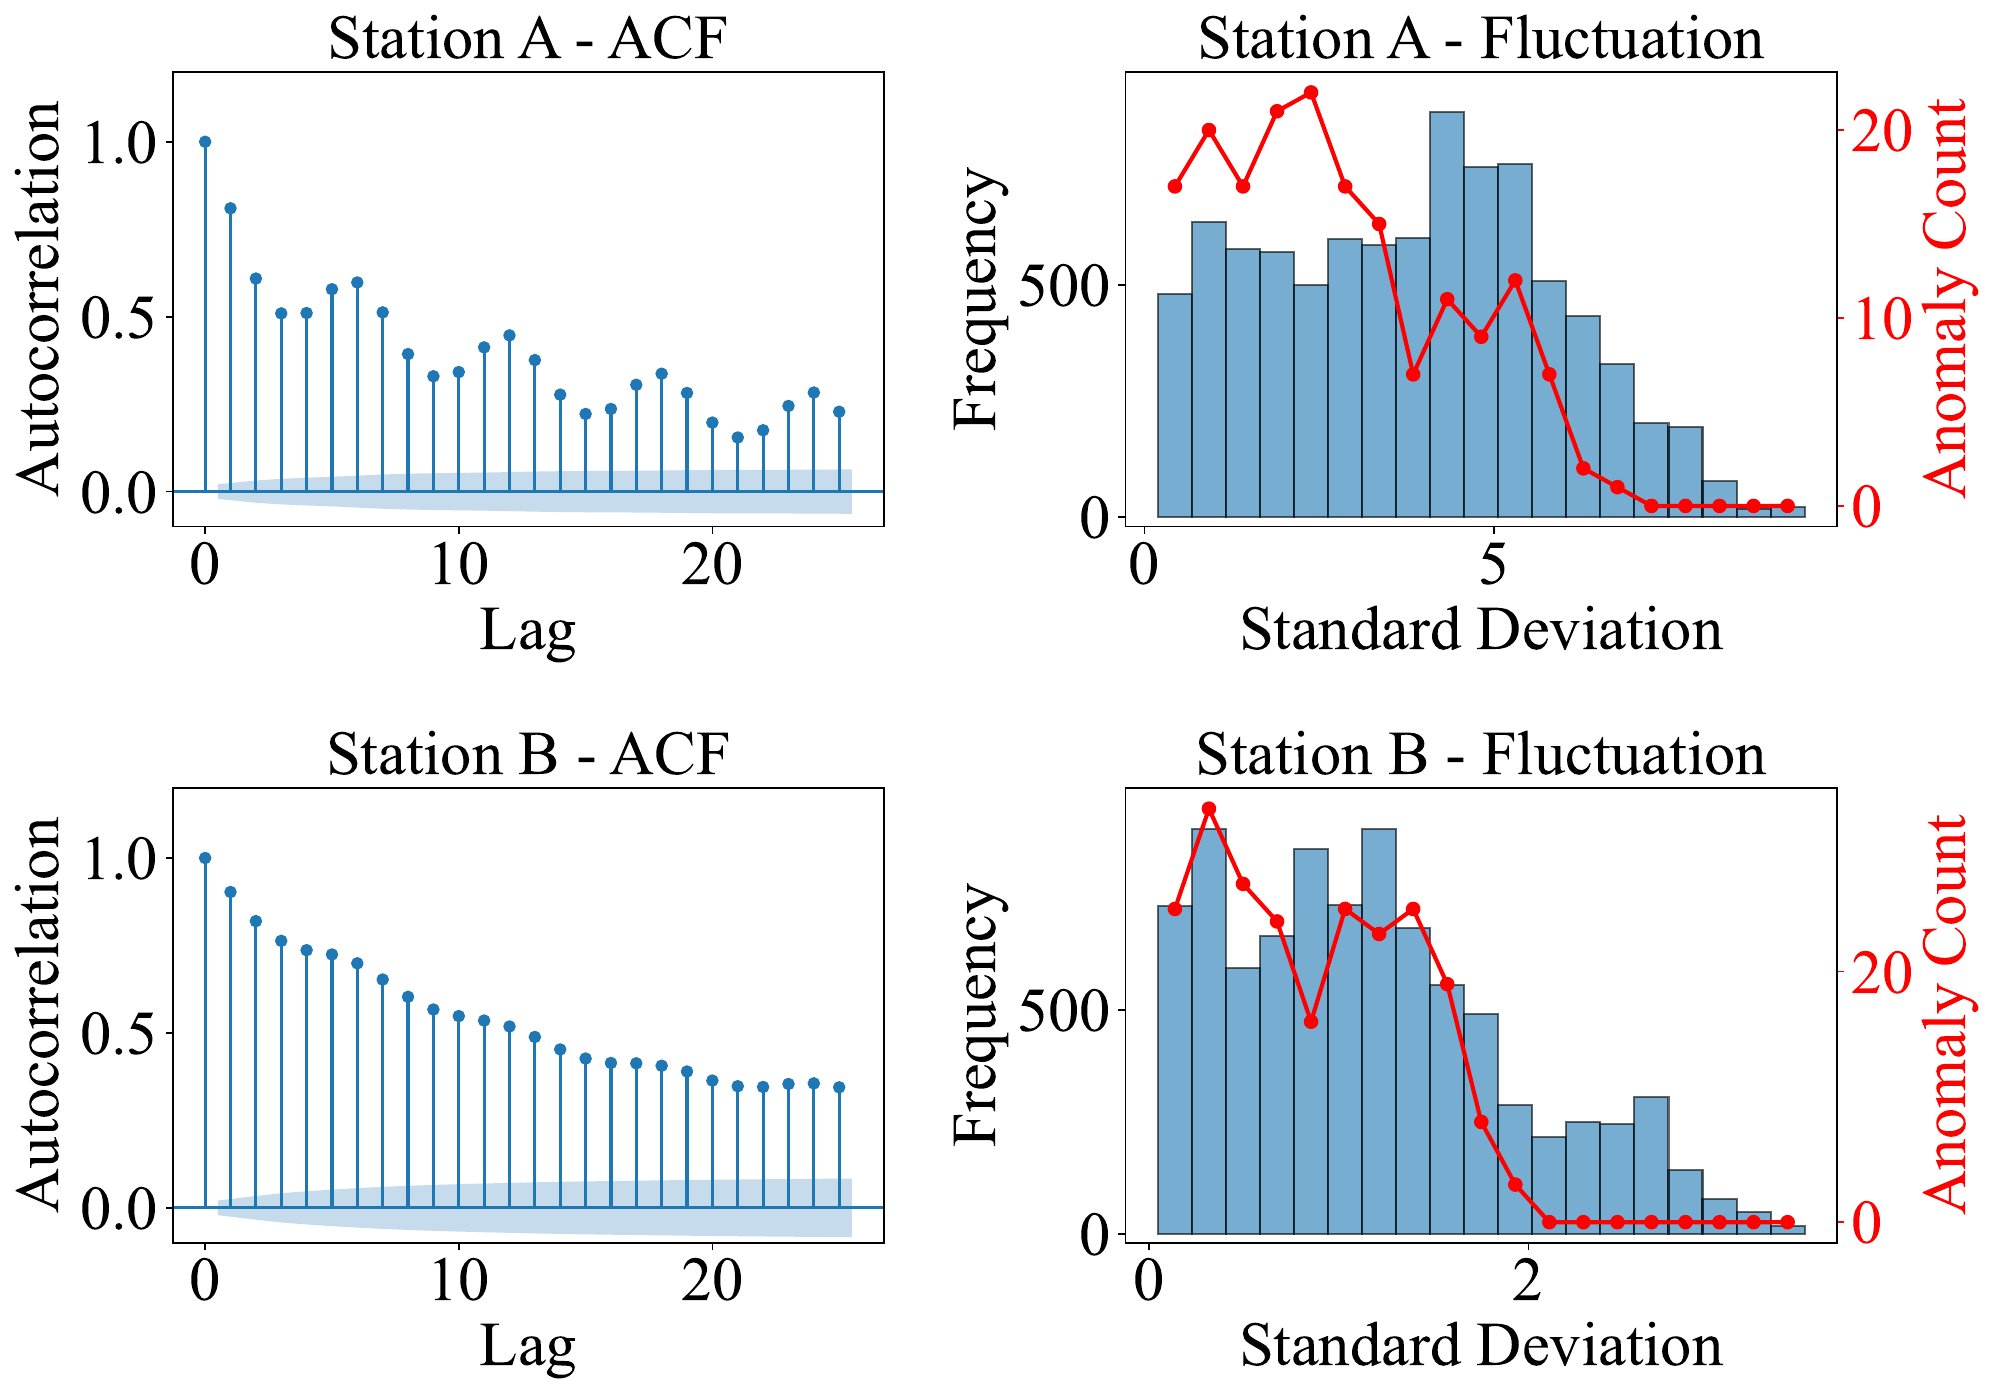} 
\caption{Two-site stationary analysis: ACF shows that Station A decays moderately, indicating short- to mid-range dependence, whereas Station B retains stronger long-memory effects. Rolling standard deviation histograms with anomaly counts reveal Station A’s fluctuations concentrated in moderate volatility episodes, while Station B exhibits a broader volatility distribution and anomalies even under low- and mid-level fluctuations.}
\label{station}
\end{figure}

Station A’s ACF declines from approximately one at lag one to around 0.5 by lag five and remains near 0.2–0.3 through lag 25, indicating moderate mid-term dependence but relatively mild long-term drift. Its rolling standard deviation is concentrated in moderate volatility bins, with anomaly counts peaking in the standard deviation range of approximately 1-3, showing that fluctuations occur primarily during episodes of elevated local volatility. In contrast, Station B exhibits a markedly slower ACF decay, retaining positive correlation above 0.3 even at lag 25, signifying pronounced long-memory effects. Its rolling standard deviation distribution is broader with a heavy right tail, and anomalies appear both at low and mid volatility levels, reflecting both pronounced trend- or cycle-driven disturbances.

\section{Implementation Details}

\subsection{Embedding Construction}
To obtain temporally enriched representations from both modalities, we employ a unified embedding strategy consisting of value, positional, and periodic components. The value embedding encodes the raw magnitude of observations, the positional embedding preserves temporal order for sequence modeling, and the periodic embedding highlights recurrent seasonal patterns. Their combination ensures that both instantaneous signals and long-term temporal structures are jointly represented, providing a robust foundation for downstream multimodal fusion.

For the water quality sequence at resolution level $l$, each time step $t$ contains an input $\mathbf{x}_t^{(l)} {\in} \mathbb{R}^{M}$. This is projected into a latent space using a multi-layer perception (MLP):
\begin{equation}
\mathbf{e}_{t}^{\text{val}} = \mathrm{MLP}(\mathbf{x}_t^{(l)}) \in \mathbb{R}^d.
\end{equation}
The MLP consists of two linear layers with ReLU activation and dropout, and the final layer projects to a dimension of $d$, transforming low-dimensional inputs into expressive representations. To encode temporal position, we add fixed sinusoidal positional embeddings to preserve the temporal order of the input sequence:
\begin{equation}
\mathbf{e}_{t}^{\mathrm{pos}} = \mathrm{PE}[t] \in \mathbb{R}^d,
\end{equation}
where $\mathrm{PE}[t]$ denotes the $t$-th row of a deterministic matrix constructed using sine and cosine functions at different frequencies:
\begin{equation}
\begin{aligned}
\mathrm{PE}[t, 2i]   &= \sin\!\left(\frac{t}{10000^{2i/d}}\right), \\
\mathrm{PE}[t, 2i+1] &= \cos\!\left(\frac{t}{10000^{2i/d}}\right),
\end{aligned}
\end{equation}
for $i=0,\ldots,d/2-1$. 
This encoding provides unique representations for each timestamp while enabling smooth interpolation of temporal relationships. 

%we add fixed sinusoidal positional embeddings:
%\begin{equation}
%\mathbf{e}_{t}^{\text{pos}} = \mathrm{PE}[t] \in \mathbb{R}^d,
%\end{equation}
%where $\mathrm{PE}[t]$ is the $t$-th row of a deterministic positional encoding matrix. 
We further incorporate learnable periodic embeddings based on discrete time attributes:
\begin{equation}
\mathbf{e}_{t}^{\text{per}} = \mathrm{TE}_\text{h}(h_t) + \mathrm{TE}_\text{w}(w_t) + \mathrm{TE}_\text{m}(m_t) \in \mathbb{R}^d,
\end{equation}
where $h_t$, $w_t$, and $m_t$ represent the hour of day, weekday, and month of time step $t$, respectively, and each $\mathrm{TE}_*$ is a trainable embedding lookup table. The final temporal embedding sequence is the element-wise sum of them:
\begin{equation}
F_{\text{temp}}^{(l)} = [\mathbf{e}_t^{\text{val}} + \mathbf{e}_t^{\text{pos}} + \mathbf{e}_t^{\text{per}}]_{t=1}^{T_l} \in \mathbb{R}^{T_l \times d}.
\end{equation}

For the image stream, the input at level $l$ is denoted by $\tilde{F}_{\text{img}}^{(l)} = [\tilde{\mathbf{f}}_1^{(l)}, \dots, \tilde{\mathbf{f}}_{T_l}^{(l)}] \in \mathbb{R}^{T_l \times d}$, where each $\tilde{\mathbf{f}}_t^{(l)}$ is the flattened and projected feature of the $t$-th downsampled image. To explicitly capture temporal dependencies among image frames, we construct a graph where each frame is treated as a node and temporal correlations between frames are encoded as edges, based on adjacency defined by temporal proximity. A graph attention network (GAT) is then applied to dynamically learn attention weights for each edge, enabling the model to focus on the most informative temporal relationships. This results in value embeddings that incorporate both spatial features and temporal interaction patterns across frames, i.e.,
\begin{equation}
\overline{\mathbf{e}}_{t}^{\text{val}} = \mathrm{GAT}(\tilde{F}_{\text{img}}^{(l)})\in \mathbb{R}^d.
\end{equation}
Positional and periodic embeddings are added in the same way as sensor data:
\begin{equation}
F_{\text{img}}^{(l)} = [\overline{\mathbf{e}}_t^{\text{val}} + \overline{\mathbf{e}}_t^{\text{pos}} + \overline{\mathbf{e}}_t^{\text{per}}]_{t=1}^{T_l} \in \mathbb{R}^{T_l \times d}.
\end{equation}

This embedding process enables the model to simultaneously encode modality-specific content, temporal order, and periodicity, ensuring aligned and informative inputs for downstream fusion and modeling.

\subsection{Construction of \texttt{XFMNet}}
Algorithm 1 outlines the workflow of \texttt{XFMNet}.
Lines 2–8 conduct aligned downsampling and multimodal feature embedding.
Lines 10–12 perform sequence decomposition followed by information enhancement.
Lines 13–18 implement progressive multimodal fusion, while line 19 executes recursive fusion.
Finally, lines 20–22 carry out regression and projection to produce the prediction results.

\begin{algorithm}[!ht]
\renewcommand\arraystretch{{2}}
\caption{{Training process of \texttt{XFMNet}}}
\label{train}
\small
{\bf Input:} Sensor time series ($X$), Remote sensing-based precipitation imagery sequence ($I$)\\
{\bf Output:} Prediction result $\hat{Y}$ 
\begin{algorithmic}[1]%{\Statex}
\FOR{each epoch}
\STATE \textit{Preprocessing and Multiscale Aligned Sampling}
\STATE Downsampling $X$ by fixed-stride 1D pooling to obtain $X^{(l)}$.
\STATE Embedding $X^{(l)}$ to obtain $F_{\text{temp}}^{(l)}$
\STATE Extracting features from $I$ by EfficientNet, obtaining $F_{\text{raw}}$.
\STATE Downsampling and projecting $F_{\text{raw}}$ to obtain $\tilde{F}_{\text{img}}^{(l)}$.
\STATE Embedding $\tilde{F}_{\text{img}}^{(l)}$ to obtain $F_{\text{img}}^{(l)}$
\STATE Concatenating $F_{\text{img}}^{(l)}$ and $F_{\text{temp}}^{(l)}$ and fusing by a 2D convolution to obtain $F^{(l)}_{con}$.
\STATE \textit{Sequence Decomposition and Multimodal Fusion}
\STATE Decomposing $F_{\mathrm{mod}}^{(l)} {\in}[F_{\mathrm{temp}}^{(l)}, F_{\mathrm{img}}^{(l)}, F^{(l)}_{con}]$ by \texttt{LocTrend} into seasonal part ${S_{\text{mod}}^{(l)}}$ and trend part ${R_{\text{mod}}^{(l)}}$.
\STATE Enhancing ${S_{\text{mod}}^{(l)}}$ in bottom-up direction by stacked linear layers and a multi-kernel convolutional block.
\STATE Enhancing ${R_{\text{mod}}^{(l)}}$ in top-down direction by transposed convolution block and stacked linear layers.
\STATE Taking seasonal part as an example, performing bidirectional interaction to obtain $A_{t\leftarrow i}^{(l)}$ and $A_{i\leftarrow t}^{(l)}$.
\STATE Performing interpolated fusion to obtain $\hat{S}_{\mathrm{temp}}^{(l)}$ and $\hat{S}_{\mathrm{img}}^{(l)}$.
\STATE Performing gated fusion to obtain $S_{\mathrm{f}}^{(l)}$.
\STATE Adding the early fusion $S_{\mathrm{con}}^{(l)}$ to obtain $\bar{S}^{(l)}$.
\STATE Adaptively integrating seasonal part $\bar{S}^{(l)}$ and trend part $\bar{R}^{(l)}$ to obtain $Z^{(l)}$.
\STATE Passing a shared feed-forward block to obtain $\hat{Z}^{(l)}$.
\STATE Performing recursive fusion to obtain $\hat{Z}^{(l,n)}$
\STATE \textit{Long-term Cross-site Prediction}
\STATE Performing scale-specific regression to obtain $Y_{\text{reg}}^{(l)}$
\STATE Projecting and averaging all scales to obtain the final prediction $\hat{Y}$.
\ENDFOR
\end{algorithmic}
\end{algorithm}

\subsection{Parameter Sensitivity} %表格
The predictive performance of \texttt{XFMNet} depends on several essential hyperparameters, including the number of recursive fusion iterations ($n$), the depth of downsampling levels ($l$), the embedding size ($d$), the dimensionality of the feedforward network ($d_f$), and the order of multi-scale information enhancement. These settings are selected through systematic experimentation to achieve optimal results. Table~\ref{tab:recursive_fusion} presents the performance under different numbers of recursive fusion iterations ($n$). Compared to $n=1$, introducing an additional fusion step ($n=2$) consistently reduces both MSE and MAE across all datasets, demonstrating that moderate recursive refinement effectively mitigates the information loss from one-shot fusion. However, further increasing $n$ beyond 2 results in clear performance degradation. This is because repeated fusion introduces redundant representations and excessive aggregation of similar signals, ultimately diminishing generalization and bringing additional computational cost. Based on these observations, $n=2$ is selected as the optimal configuration, striking the best balance between information retention and model simplicity.

\begin{table*}[ht]
\centering
\caption{Effect of recursive fusion iterations ($n$) on forecasting accuracy.} %Optimal performance is observed at $n=2$.}
\begin{tabular}{c|cc|cc|cc|cc|cc}
\toprule
\multirow{2}{*}{Dataset} & \multicolumn{2}{|c|}{$n=1$} & \multicolumn{2}{c|}{$n=2$} & \multicolumn{2}{c|}{$n=3$} & \multicolumn{2}{c|}{$n=4$} & \multicolumn{2}{c}{$n=5$} \\
\cmidrule(lr){2-3}\cmidrule(lr){4-5}\cmidrule(lr){6-7}\cmidrule(lr){8-9}\cmidrule(lr){10-11}
& MSE & MAE & MSE & MAE & MSE & MAE & MSE & MAE & MSE & MAE \\
\midrule
BJ & 0.877 & 0.726 & 0.867 & 0.721 & 0.879 & 0.726 & 0.893 & 0.734 & 0.881 & 0.728 \\
BTH     & 0.781 & 0.611 & 0.726 & 0.585 & 0.726 & 0.585 & 0.728 & 0.586 & 0.726 & 0.585 \\
Ala & 1.148 & 0.660 & 0.854 & 0.578 & 1.415 & 0.716 & 2.256 & 0.823 & 1.092 & 0.626 \\
\bottomrule
\end{tabular}
\label{tab:recursive_fusion}
\end{table*}

Table~\ref{tab:downsampling_levels} shows the forecasting performance under different numbers of downsampling levels ($l$). The results reveal that introducing a moderate degree of multiscale downsampling substantially improves predictive accuracy compared to no downsampling ($l=0$). Specifically, setting $l=3$ consistently achieves the lowest MSE and MAE on all datasets, highlighting its effectiveness in capturing salient temporal patterns while reducing redundancy. However, further increasing $l$ to 4 degrades performance, because excessive resolution reduction discards fine-grained temporal signals critical for modeling localized dynamics. These results suggest that a balanced downsampling configuration is essential for maximizing the benefits of multiscale feature extraction.

\begin{table*}[t]
\centering
\caption{Forecasting performance with varying numbers of downsampling levels ($l$).}
\begin{tabular}{c|cc|cc|cc|cc|cc}
\toprule
\multirow{2}{*}{Dataset} & \multicolumn{2}{c|}{$l=0$} & \multicolumn{2}{c|}{$l=1$} & \multicolumn{2}{c|}{$l=2$} & \multicolumn{2}{c|}{$l=3$} & \multicolumn{2}{c}{$l=4$} \\
\cmidrule(lr){2-3} \cmidrule(lr){4-5} \cmidrule(lr){6-7} \cmidrule(lr){8-9} \cmidrule(lr){10-11}
& MSE & MAE & MSE & MAE & MSE & MAE & MSE & MAE & MSE & MAE \\
\midrule
BJ & 0.872 & 0.724 & 0.913 & 0.742 & 0.908 & 0.740 & 0.867 & 0.721 & 0.881 & 0.727 \\
BTH     & 0.743 & 0.594 & 0.743 & 0.594 & 0.735 & 0.590 & 0.726 & 0.585 & 0.735 & 0.589 \\
Ala & 1.428 & 0.734 & 0.880 & 0.582 & 1.208 & 0.674 & 0.854 & 0.578 & 1.624 & 0.772 \\
\bottomrule
\end{tabular}
\label{tab:downsampling_levels}
\end{table*}

Table~\ref{tab:embedding_dimension} shows the impact of varying the embedding dimension $d$ on predictive performance. As $d$ increases from 8 to 16, all datasets consistently exhibit improved MSE and MAE, highlighting that richer embeddings help capture more informative temporal and spatial patterns. However, further increasing $d$ beyond 16 does not lead to consistent improvements. While BTH benefits slightly when $d=32$, the Alabama dataset shows clear performance degradation, primarily due to overfitting and increased variance in smaller datasets. Overall, $d=16$ provides the most stable and competitive results across different scenarios, striking a balance between expressiveness and generalization.

\begin{table*}[htbp]
\centering
\caption{Effect of embedding dimension $d$ on forecasting performance.}
\renewcommand{\arraystretch}{1.1}
\begin{tabular}{c|cc|cc|cc|cc|cc}
\toprule
\multirow{2}{*}{Dataset} & 
\multicolumn{2}{|c|}{$d=8$} &
\multicolumn{2}{c|}{$d=16$} &
\multicolumn{2}{c|}{$d=24$} &
\multicolumn{2}{c|}{$d=32$} &
\multicolumn{2}{c}{$d=40$} \\
\cmidrule(lr){2-3}
\cmidrule(lr){4-5}
\cmidrule(lr){6-7}
\cmidrule(lr){8-9}
\cmidrule(lr){10-11}
& MSE & MAE & MSE & MAE & MSE & MAE & MSE & MAE & MSE & MAE \\
\midrule
BJ & 0.915 & 0.740 & 0.867 & 0.721 & 0.906 & 0.737 & 0.889 & 0.731 & 0.876 & 0.725 \\
BTH     & 0.735 & 0.593 & 0.726 & 0.585 & 0.720 & 0.583 & 0.709 & 0.581 & 0.717 & 0.583 \\
Ala & 0.895 & 0.591 & 0.854 & 0.578 & 1.396 & 0.623 & 1.433 & 0.736 & 0.875 & 0.587 \\
\bottomrule
\end{tabular}
\label{tab:embedding_dimension}
\end{table*}

We further examine the impact of varying the hidden dimension $d_f$ in the feedforward layers (Table~\ref{tab:ffd_dim}). The results reveal that moderate hidden sizes (e.g., $d_f=8$ or $d_f=16$) deliver more consistent performance across datasets. In particular, increasing $d_f$ beyond 24 tends to degrade the MSE and MAE in Alabama, primarily due to overparameterization and limited data coverage in this region, which leads to overfitting. On BJ and BTH, the results remain relatively stable across different hidden dimensions, suggesting that these datasets are less sensitive to the capacity of the feedforward layers. Consequently, we set $d_f=16$ to maintain a trade-off between representation capacity and robust generalization.

\begin{table*}[t]
\centering
\caption{Impact of hidden dimension $d_f$ in feedforward layers on MSE and MAE across datasets.}
\begin{tabular}{c|cc|cc|cc|cc|cc}
\toprule
\multirow{2}{*}{Dataset} & \multicolumn{2}{c|}{$d_f=8$} & \multicolumn{2}{c|}{$d_f=16$} & \multicolumn{2}{c|}{$d_f=24$} & \multicolumn{2}{c|}{$d_f=32$} & \multicolumn{2}{c}{$d_f=40$} \\
\cmidrule(lr){2-3}
\cmidrule(lr){4-5}
\cmidrule(lr){6-7}
\cmidrule(lr){8-9}
\cmidrule(lr){10-11}
 & MSE & MAE & MSE & MAE & MSE & MAE & MSE & MAE & MSE & MAE \\
\midrule
Beijing & 0.867 & 0.720 & 0.860 & 0.716 & 0.900 & 0.732 & 0.867 & 0.721 & 0.860 & 0.717 \\
BTH     & 0.707 & 0.579 & 0.725 & 0.585 & 0.719 & 0.583 & 0.726 & 0.585 & 0.712 & 0.582 \\
Alabama & 0.823 & 0.560 & 1.016 & 0.614 & 1.545 & 0.747 & 0.854 & 0.578 & 1.398 & 0.713 \\
\bottomrule
\end{tabular}
\label{tab:ffd_dim}
\end{table*}

%We set the sliding-window length $w$ to control the granularity of local temporal segments in \texttt{LocTrend}. It is shown in Table \ref{window} that a larger window size could smooth over fine-grained dynamics, while a smaller window may introduce noise in trend estimation. We find that $w = 27$ offers stable performance across datasets with different temporal characteristics. Notably, since \texttt{LocTrend} employs fixed kernel projections without parameter learning, this setting also ensures fast execution during both training and inference.

We set the sliding-window length $w$ to control the granularity of local temporal segments in \texttt{LocTrend}. As illustrated in Table~\ref{window}, the choice of $w$ balances sensitivity to short-term fluctuations and the ability to capture longer-range trends. A small window size tends to increase the influence of high-frequency variations and may introduce noise in the extracted trend components. Conversely, a huge window can over-smooth the sequence, potentially masking abrupt changes or fine-grained dynamics. We find that a moderate setting of $w = 27$ consistently yields robust performance across datasets exhibiting diverse temporal characteristics, including periodicity, abrupt transitions, and non-stationary behaviors. Furthermore, since \texttt{LocTrend} operates with fixed kernel projections and avoids costly parameter learning or matrix decomposition, this configuration ensures both computational efficiency and ease of deployment during training and inference.

\begin{table*}[htbp]
\centering
\caption{Performance of \texttt{XFMNet} under Different window size $w$}
\label{window}
\begin{tabular}{c|cc|cc|cc|cc|cc}
\toprule
\multirow{2}{*}{Dataset} & 
\multicolumn{2}{c|}{$w=9$} & 
\multicolumn{2}{c|}{$w=18$} & 
\multicolumn{2}{c|}{$w=27$} & 
\multicolumn{2}{c|}{$w=36$} & 
\multicolumn{2}{c}{$w=45$} \\
\cmidrule(r){2-3} \cmidrule(r){4-5} \cmidrule(r){6-7} \cmidrule(r){8-9} \cmidrule(r){10-11}
 & MSE & MAE & MSE & MAE & MSE & MAE & MSE & MAE & MSE & MAE \\
\midrule
BJ  & 0.868 & 0.721 & 0.867 & 0.721 & 0.867 & 0.721 & 0.867 & 0.721 & 0.867 & 0.721 \\
BTH      & 0.725 & 0.585 & 0.727 & 0.585 & 0.727 & 0.585 & 0.727 & 0.585 & 0.727 & 0.586 \\
Ala  & 0.995 & 0.628 & 0.958 & 0.620 & 0.929 & 0.609 & 0.973 & 0.621 & 0.946 & 0.613 \\
\bottomrule
\end{tabular}
\end{table*}

To further amplify decomposed components and facilitate cross-resolution representation alignment, we introduce a hierarchical dual-path enhancement mechanism. Table \ref{tab:trend-season-order} show that for the seasonal component, a bottom-up refinement achieves better performance. Given that high-frequency seasonal variations are typically rooted in local fluctuations, the model progressively aggregates fine-grained representations into coarser ones. Conversely, for the trend component, the top-down enhancement strategy achieves better performance. This design is motivated by the observation that trend dynamics often manifest over long horizons, and global structure should guide the shaping of local trends. Coarse-resolution trend signals are gradually upsampled to reconstruct higher-resolution features. Overall, this bidirectional refinement paradigm provides a principled way to separately optimize seasonality and trend components, while also aligning multi-resolution features. It strengthens both local sensitivity and global awareness, forming a key part of our architecture’s effectiveness in complex temporal environments.

\begin{table*}[htbp]
\centering
\caption{Performance under different season-trend enhancement orders.}
\label{tab:trend-season-order}
\begin{tabular}{c|cc|cc|cc|cc}
\toprule
\multirow{2}{*}{Dataset} & \multicolumn{2}{c|}{season↓-trend↑} & \multicolumn{2}{c|}{season↑-trend↑} & \multicolumn{2}{c|}{season↑-trend↓} & \multicolumn{2}{c}{season↓-trend↓} \\
\cmidrule(r){2-3} \cmidrule(r){4-5} \cmidrule(r){6-7} \cmidrule(r){8-9}
& MSE & MAE & MSE & MAE & MSE & MAE & MSE & MAE \\
\midrule
BJ & 0.867 & 0.721 & 0.868 & 0.721 & 0.867 & 0.721 & 0.864 & 0.720 \\
BTH     & 0.727 & 0.585 & 0.727 & 0.586 & 0.726 & 0.585 & 0.726 & 0.585 \\
Ala & 1.063 & 0.640 & 1.254 & 0.675 & 0.854 & 0.578 & 0.969 & 0.621 \\
\bottomrule
\end{tabular}
\end{table*}

\section{Dataset Description}
The details of the three real-world water quality datasets are provided in Table \ref{sum}. The BJ and BTH datasets cover the period from January 2019 to December 2022, with measurements recorded every four hours. The BJ dataset contains dissolved oxygen (DO) data from six monitoring stations distributed across the Chaobai River basin in the Beijing area, covering approximately 120 km. The BTH data set includes total nitrogen (TN) measurements from nine stations located throughout the broader region of three cities, within the Beiyan Canal, covering a spatial range of about 300 km. The Ala dataset comprises hourly DO observations from five stations in Alabama, collected between January 2021 and December 2022. These stations are situated within the Cahaba River watershed and span approximately 190 km. All datasets are supplemented with remote sensing-based precipitation imagery, temporally aligned with the water quality sampling frequency (four-hourly for BJ and BTH; hourly for Ala) and featuring a spatial resolution of 0.1 {$\times$} 0.1°. An example of remote sensing-based precipitation imagery is shown in Fig. \ref{rain}. It captures the spatio-temporal environmental dynamics, including spatial context and rainfall variability that influence water quality. We release a publicly available multimodal water quality prediction dataset BJ to support further research in multimodal environmental forecasting. The sample data is presented in Table \ref{tab:data-sample}. %还有遥感图

\begin{comment}
\begin{table}[!ht]
\centering
\caption{Dataset Description}
\label{sum}
\begin{tabular}{cccc}
\hline
\multirow{2}{*}{Parameter} & \multicolumn{3}{c}{Datasets}  \\ \cline{2-4}
& BTH & BJ & Ala \\ \hline
Number of station   & 9  & 6       & 5       \\ \hline
% Time Span        & \multicolumn{2}{c|}{Jan. 1, 2019–Dec. 31, 2022}  & Jan. 1, 2021–Dec. 31, 2022 \\ \hline
Sampling frequency        & 4 hours & 4 hours & 1 hour \\ \hline
Data length      & 8,766   & 8,766   & 17,520   \\ \hline
Water quality indicator  & TN     & DO     & DO      \\ \hline
\end{tabular}
\end{table}
\end{comment}

\begin{table}[!ht]
\centering
\caption{Dataset Description}
\label{sum}
\begin{tabular}{lccc}
\toprule
\textbf{Dataset} & \textbf{BTH} & \textbf{BJ} & \textbf{Ala} \\
\midrule
Number of stations      & 9     & 6     & 5     \\
Sampling frequency      & 4 h   & 4 h   & 1 h   \\
Data length             & 8,766 & 8,766 & 17,520 \\
Water quality indicator & TN    & DO    & DO    \\
\bottomrule
\end{tabular}
\end{table}

\begin{figure}[!ht]
\centering
\includegraphics[width=0.6\columnwidth]{figure/rainfall.jpg} 
\caption{Remote sensing-based precipitation imagery.}
\label{rain}
\end{figure}

%样例数据
\begin{table*}[htbp]
\centering
\caption{Example of DO Index in BJ Dataset with Station Coordinates}
\label{tab:data-sample}
\renewcommand{\arraystretch}{1.2}
\begin{tabular}{c|cccccc}
\toprule
\textbf{Station} & \textbf{Dahongqiao} & \textbf{Shawo} & \textbf{Xinbaliqiao} & \textbf{Wangjiabai} & \textbf{Wucun} & \textbf{Huairoushuiku} \\
\midrule
\textbf{Latitude}  & 40.010°N & 39.850°N & 39.920°N & 39.970°N & 39.880°N & 40.350°N \\
\textbf{Longitude} & 116.320°E & 116.240°E & 116.500°E & 116.700°E & 116.600°E & 116.630°E \\
\midrule
2022/1/1 0:00  & 11.17 Mg/L & 11.06 Mg/L & 6.39 Mg/L & 6.04 Mg/L & 10.71 Mg/L & 13.92 Mg/L\\
2022/1/1 4:00  & 11.13 Mg/L& 11.08 Mg/L& 5.68 Mg/L & 5.80 Mg/L & 10.38 Mg/L & 13.98 Mg/L\\
2022/1/1 8:00  & 11.09 Mg/L & 10.95 Mg/L & 5.91 Mg/L & 5.92 Mg/L & 10.00 Mg/L & 13.97 Mg/L \\
2022/1/1 12:00 & 11.05 Mg/L & 10.92 Mg/L& 10.11 Mg/L& 5.78 Mg/L & 9.96 Mg/L & 13.94 Mg/L\\
2022/1/1 16:00 & 11.01 Mg/L& 11.48 Mg/L& 11.99 Mg/L & 5.84 Mg/L & 10.27 Mg/L & 13.96 Mg/L\\
2022/1/1 20:00 & 10.97 Mg/L & 11.58 Mg/L & 8.45 Mg/L & 5.87 Mg/L & 10.63 Mg/L & 13.89 Mg/L \\
2022/1/2 0:00  & 10.93 Mg/L & 9.20 Mg/L  & 5.82 Mg/L & 13.16 Mg/L& 14.23 Mg/L& 14.80 Mg/L\\
2022/1/2 4:00  & 10.89 Mg/L & 9.28 Mg/L & 4.75 Mg/L & 13.08 Mg/L & 13.39 Mg/L & 14.47 Mg/L\\
2022/1/2 8:00  & 10.86 Mg/L & 9.40 Mg/L & 4.70 Mg/L & 12.62 Mg/L & 13.21 Mg/L & 14.64 Mg/L\\
2022/1/2 12:00 & 10.82 Mg/L & 10.22 Mg/L& 10.00 Mg/L& 13.27 Mg/L& 13.55 Mg/L& 14.66 Mg/L\\
\bottomrule
\end{tabular}
\end{table*}

\section{Compared Models and Evaluation Metrics}
We compare our method with several state-of-the-art time series forecasting models. TimeKAN \cite{TimeKAN} introduces a KAN-based architecture that decomposes time series into multiple frequency bands and learns multi-order representations for each. FilterTS \cite{FilterTS} employs learnable frequency-domain filters to extract salient patterns and suppress high-frequency noise. TimePFN \cite{TimePFN} leverages synthetic data priors and permutation-invariant transformers to achieve robust forecasting in few-shot and zero-shot settings. MSGNet \cite{MSGNet} models multi-scale inter-series dependencies via frequency decomposition and adaptive graph convolution. TimeMixer \cite{TimeMixer} proposes a fully MLP-based framework that integrates seasonal and trend components across multiple resolutions through parallel decomposition and multi-predictor fusion. iTransformer \cite{iTransformer} inverts the attention mechanism over variate tokens to better capture multivariate dependencies. TimesNet \cite{TimesNet} converts 1D time series into 2D period-based tensors and applies 2D convolutions to model intra- and inter-period variations. FEDformer \cite{FEDformer} combines seasonal-trend decomposition with frequency-domain modeling for efficient long-term forecasting.

In addition, we evaluate different fusion methods, including CDA \cite{CDA}, MBT \cite{MBT}, LMF \cite{LMF}, and TFN \cite{TFN}, which are directly integrated into our framework by replacing \texttt{XGateFusion} while keeping all other settings unchanged. Specifically, CDA adopts a cross-modal attention mechanism to align temporal and spatial features. MBT introduces a shared bottleneck token for efficient cross-modal interaction while preserving modality-specific representations. LMF employs tensor factorization to reduce fusion complexity and emphasize complementary information across modalities. TFN performs outer product-based tensor fusion to capture high-order feature interactions. Large models including TimeVLM \cite{TimeVLM}, Timer \cite{Timer}, AutoTimes \cite{AutoTimes}, and aLLM4TS \cite{aLLM4TS}. TimeVLM incorporates vision-language pretraining for temporal forecasting with multimodal inputs. Timer leverages large-scale pretraining on diverse temporal datasets to enhance cross-domain generalization. AutoTimes employs neural architecture search and automated hyperparameter tuning to adapt to varying data characteristics. aLLM4TS extends large language models for time-series forecasting by integrating prompt-driven temporal encoding. In all these models, imagery is encoded as additional input following a consistent multimodal setup.

MSE emphasizes large deviations and is more sensitive to abrupt fluctuations, while MAE reflects overall average error with greater robustness to outliers. Lower MSE and MAE values indicate higher forecasting accuracy and better model performance. They are calculated as:
\begin{equation}
\text{MAE}{=}\frac{1}{a} \sum_{j=1}^a\left|\hat{h}_j{-}h_j\right|
\end{equation}
\begin{equation}
\text{MSE}{=}\frac{1}{a} \sum_{j=1}^a\left|\hat{h}_j{-}h_j\right|^2
\end{equation}
where $a$ denotes the number of samples. $h_j$ and $\hat{h}_j$ denote the ground truth and predicted values of data point $j$.

\section{Full Results}
\subsection{Comparitive Results} %可以画图

Tables~\ref{tab:main_results} and \ref{multimodallarge} comprehensively summarize the forecasting performance of all baseline models and the proposed \texttt{XFMNet} across three representative real-world datasets, each evaluated under a wide range of prediction horizons. These datasets differ in sampling frequency, spatial layout, and environmental variability, providing a robust benchmark for model generalization. The detailed trend comparisons of MSE and MAE metrics over different forecasting steps are visualized in Figs.~\ref{BJ}–\ref{Ala}. These figures show how prediction errors evolve as the horizon length increases, offering insight into model stability under both short-term and long-term scenarios. Fig.~\ref{ladarall} further presents the averaged performance across all horizons, highlighting overall model behavior. Compared with state-of-the-art approaches, \texttt{XFMNet} consistently achieves superior performance on nearly all horizons and datasets, attributed to its stepwise multimodal fusion design, which effectively incorporates remote sensing imagery and captures evolving spatiotemporal patterns without losing localized temporal dynamics.

%The BJ dataset, primarily composed of water quality records from urban monitoring stations, exhibits relatively smooth temporal patterns with localized fluctuations driven by rainfall. This dataset serves as a relatively regular benchmark. As shown in Fig.~\ref{BJ}, \texttt{XFMNet} nearly outperforms all competing models across all horizons, with particularly significant gains in MSE. Since MSE is more sensitive to large deviations, this suggests that \texttt{XFMNet} is especially effective in detecting sharp changes or localized anomalies. The model's ability to leverage visual cues offers an advantage in anticipating such events. MAE results, which reflect general accuracy, also remain consistently favorable, indicating reliable modeling of baseline trends and normal variation ranges.
The BJ dataset, primarily composed of water quality records from dense urban monitoring stations, exhibits relatively smooth long-term temporal patterns interspersed with localized fluctuations induced by rainfall and anthropogenic activities. This makes BJ an ideal benchmark for evaluating a model’s capability to capture stable trends while remaining sensitive to transient anomalies. As reported in Tables~\ref{tab:main_results} and \ref{multimodallarge} and visualized in Fig.~\ref{BJ}, \texttt{XFMNet} demonstrates strong and stable forecasting performance across all prediction horizons. The improvements are especially evident in MSE, which is inherently more sensitive to large deviations, indicating that \texttt{XFMNet} effectively handles sharp concentration changes and localized anomalies. Meanwhile, the MAE, which captures overall prediction accuracy, remains consistently favorable, demonstrating the model’s ability to reliably represent baseline temporal dynamics. These results confirm that integrating visual cues and recursive multimodal fusion provides robust and accurate modeling for complex tasks in predicting urban water quality.

%The BTH dataset introduces increased modeling complexity. It covers a broad spatial region encompassing three metropolitan areas, with a dense network of monitoring sites affected by both natural hydrological processes and anthropogenic factors. The spatial heterogeneity leads to frequent inter-site correlations, phase shifts across locations, and a higher degree of non-stationarity. These characteristics typically challenge traditional models that treat series independently or rely solely on self-attention. However, \texttt{XFMNet} still demonstrates strong performance on this dataset, achieving the lowest or near-lowest MAE and lowest MSE under every time horizon, as shown in Fig.~\ref{BTH}. This suggests that its recursive cross-modal fusion enables better extraction of inter-series dependencies and dynamic relationships, particularly through its alignment mechanism that adapts at each step. Notably, its margin of superiority widens at longer horizons, indicating resilience against error accumulation during recursive inference.

The BTH dataset presents a substantially higher level of modeling complexity compared to BJ. It spans a broad geographic region covering three metropolitan areas, where diverse hydrological processes and anthropogenic influences jointly shape water quality dynamics. Such conditions produce strong spatial heterogeneity, characterized by frequent inter-site correlations, asynchronous phase shifts, and pronounced nonstationarity. These factors pose significant challenges to conventional forecasting models. Despite these challenges, \texttt{XFMNet} exhibits consistently strong performance across all prediction horizons, as reported in Tables~\ref{tab:main_results} and \ref{multimodallarge} and visualized in Fig.~\ref{BTH}. Its MSE remains the lowest among all compared approaches, and its MAE ranks at or near the best under every forecast step, highlighting the model’s robustness under highly variable spatial-temporal conditions. The advantage of \texttt{XFMNet} is particularly pronounced at longer horizons. This robustness can be attributed to its recursive cross-modal fusion and alignment mechanism, which iteratively refines shared representations while retaining local temporal features and spatial context. These design choices enable \texttt{XFMNet} to capture both site-specific variability and cross-site interactions, resulting in reliable forecasting performance in scenarios characterized by complex spatial coupling and dynamic environmental disturbances.

%The Ala dataset, representing a natural watershed system, features substantial seasonal variation driven by precipitation events, runoff cycles, and land-cover transitions. Unlike urban datasets, Ala exhibits strong periodicity and abrupt changes due to exogenous drivers. As reflected in Table~\ref{tab:main_results} and Fig.~\ref{Ala}, most baselines suffer performance degradation on this dataset, especially under long-horizon settings, due to limited ability to model such exogenous and nonlinear behaviors. In contrast, \texttt{XFMNet} maintains a consistently low error across all forecasting steps, with the lowest MSE and MAE throughout. Fig.~\ref{ladar} provides a compact visual summary of these performance comparisons across all datasets and prediction lengths. It clearly shows that \texttt{XFMNet} excels in short-term prediction (96–192 steps) and maintains reliable long-range forecasting ability beyond 480 steps, a regime where most baselines deteriorate significantly. This consistent advantage underscores the benefits of step-wise multimodal alignment and fine-grained feature interaction, particularly in modeling multi-source environmental data where spatial, temporal, and contextual information are deeply intertwined.

The Ala dataset, representing a natural watershed system, poses forecasting challenges distinct from those of urban river networks. Its water quality dynamics are heavily influenced by seasonal precipitation events, runoff cycles, and land cover transitions, resulting in strong periodicity interspersed with abrupt changes driven by exogenous factors such as storms. Unlike urban datasets, where variations are often moderated by engineered infrastructure, Ala exhibits pronounced nonlinear behaviors and sudden regime shifts. As shown in Fig.\ref{Ala}, most baseline models experience noticeable performance degradation on this dataset, particularly at long prediction horizons where capturing such complex exogenous signals becomes critical. In contrast, \texttt{XFMNet} consistently achieves the lowest or second-lowest MSE and MAE across all horizons, demonstrating resilience to both seasonal oscillations and abrupt environmental disturbances. This persistent advantage reflects the benefits of its stepwise multimodal alignment and fine-grained feature interaction, which jointly leverage remote sensing imagery and temporal series to capture the coupled spatial and temporal drivers of water quality. This capability is crucial for modeling natural watersheds, where ecological processes are deeply intertwined and subject to rapid external perturbations.

%BJ
\begin{figure}[htbp]
    \centering
    \subfigure[MSE comparison on the first group of baseline models.]{%
        \includegraphics[width=0.95\columnwidth]{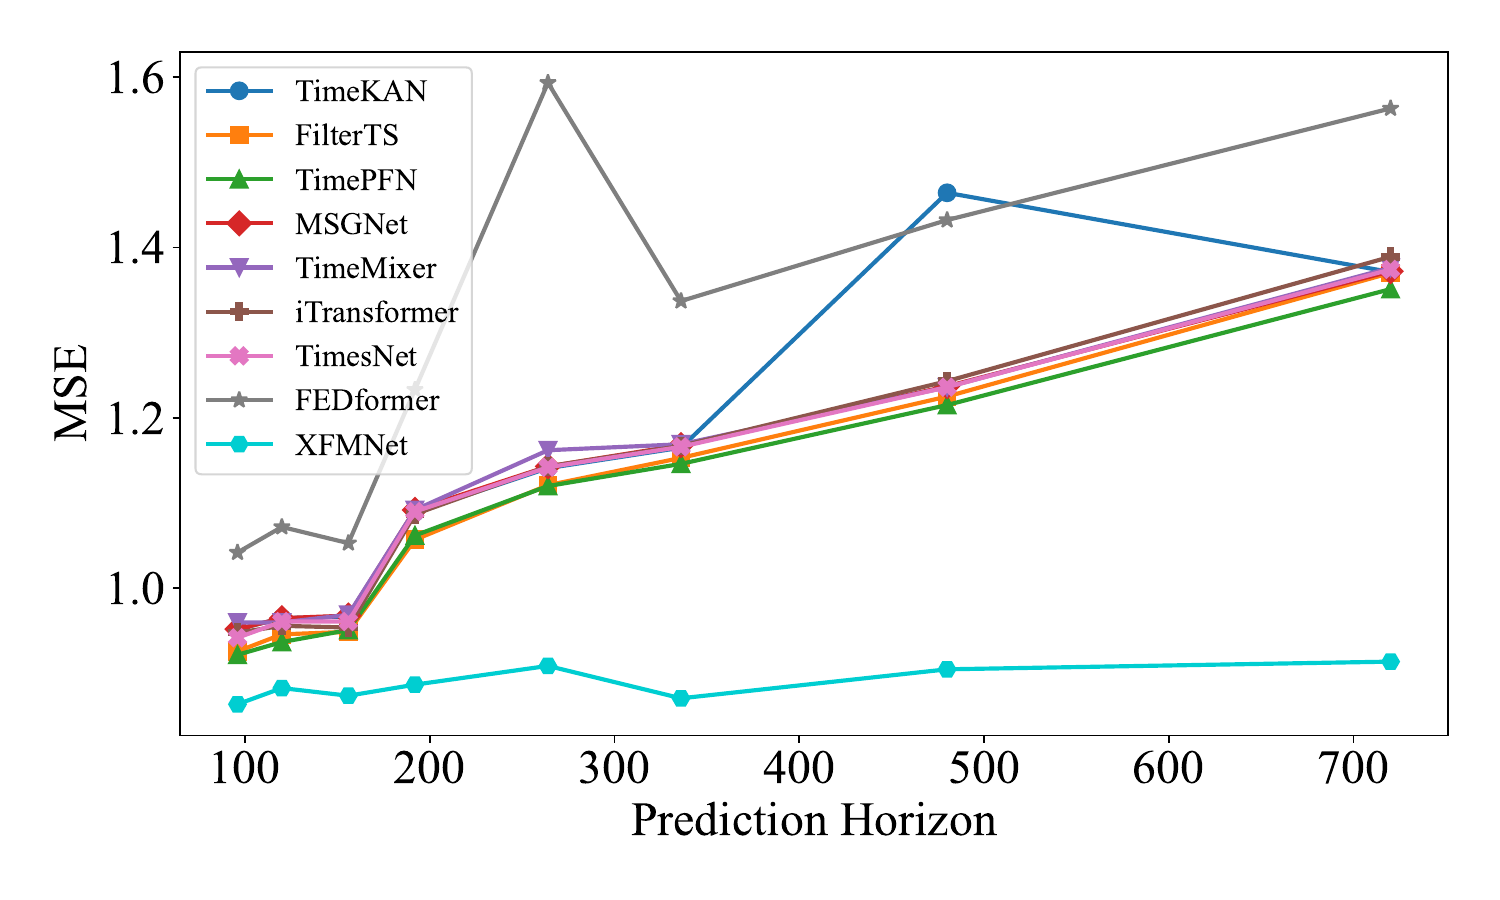}%
        \label{BJ1}
    }
    \quad
    \subfigure[MAE comparison on the first group of baseline models.]{%
        \includegraphics[width=0.95\columnwidth]{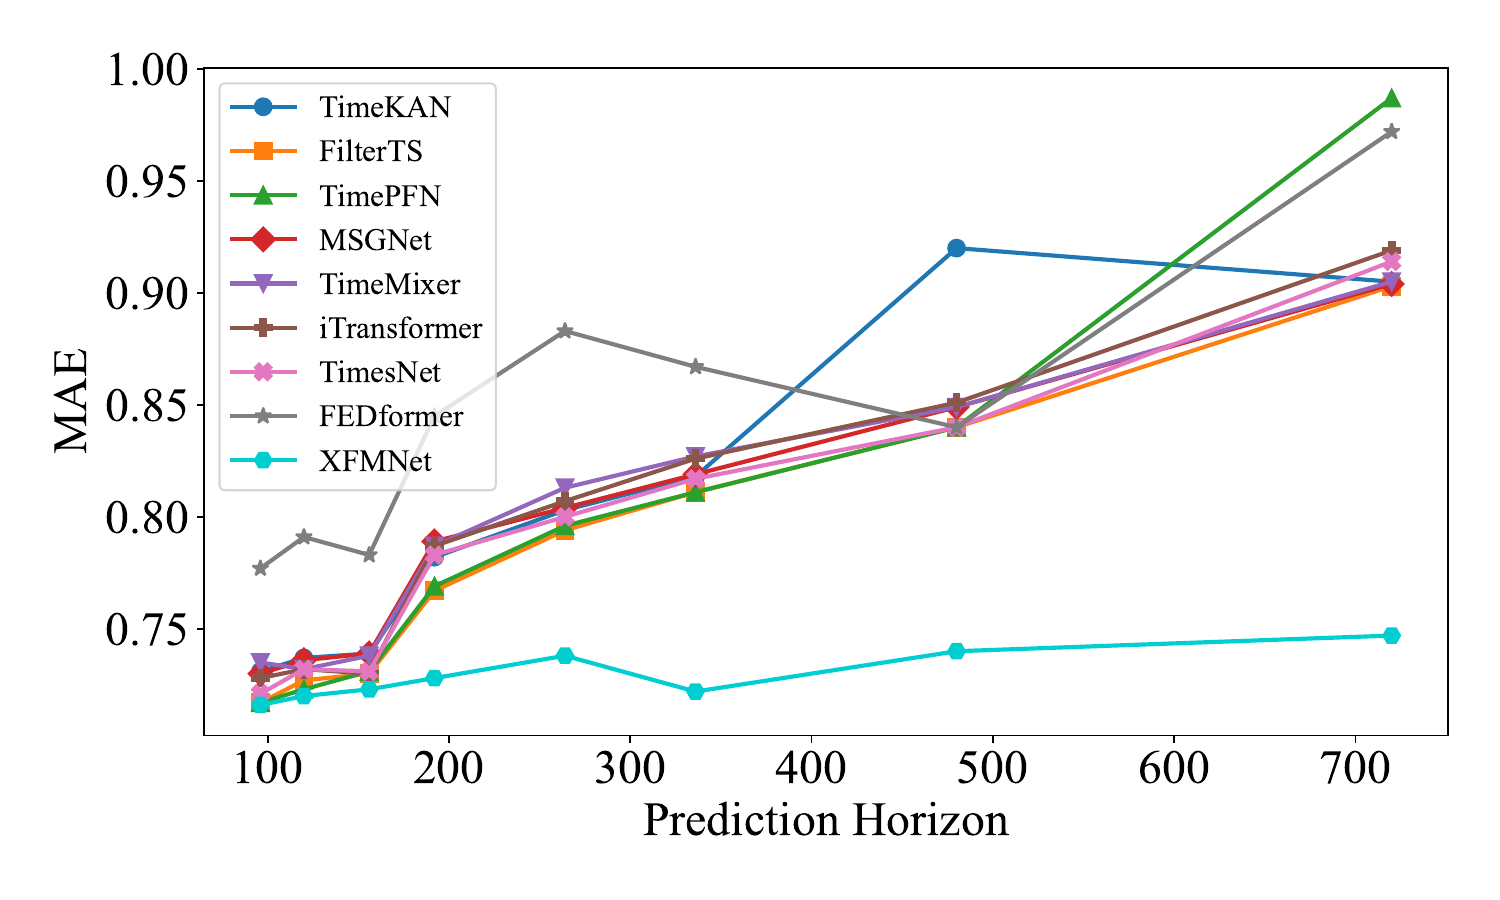}%
        \label{BJ2}
    }
    \quad
    \subfigure[MSE comparison on the second group of baseline models.]{%
        \includegraphics[width=0.95\columnwidth]{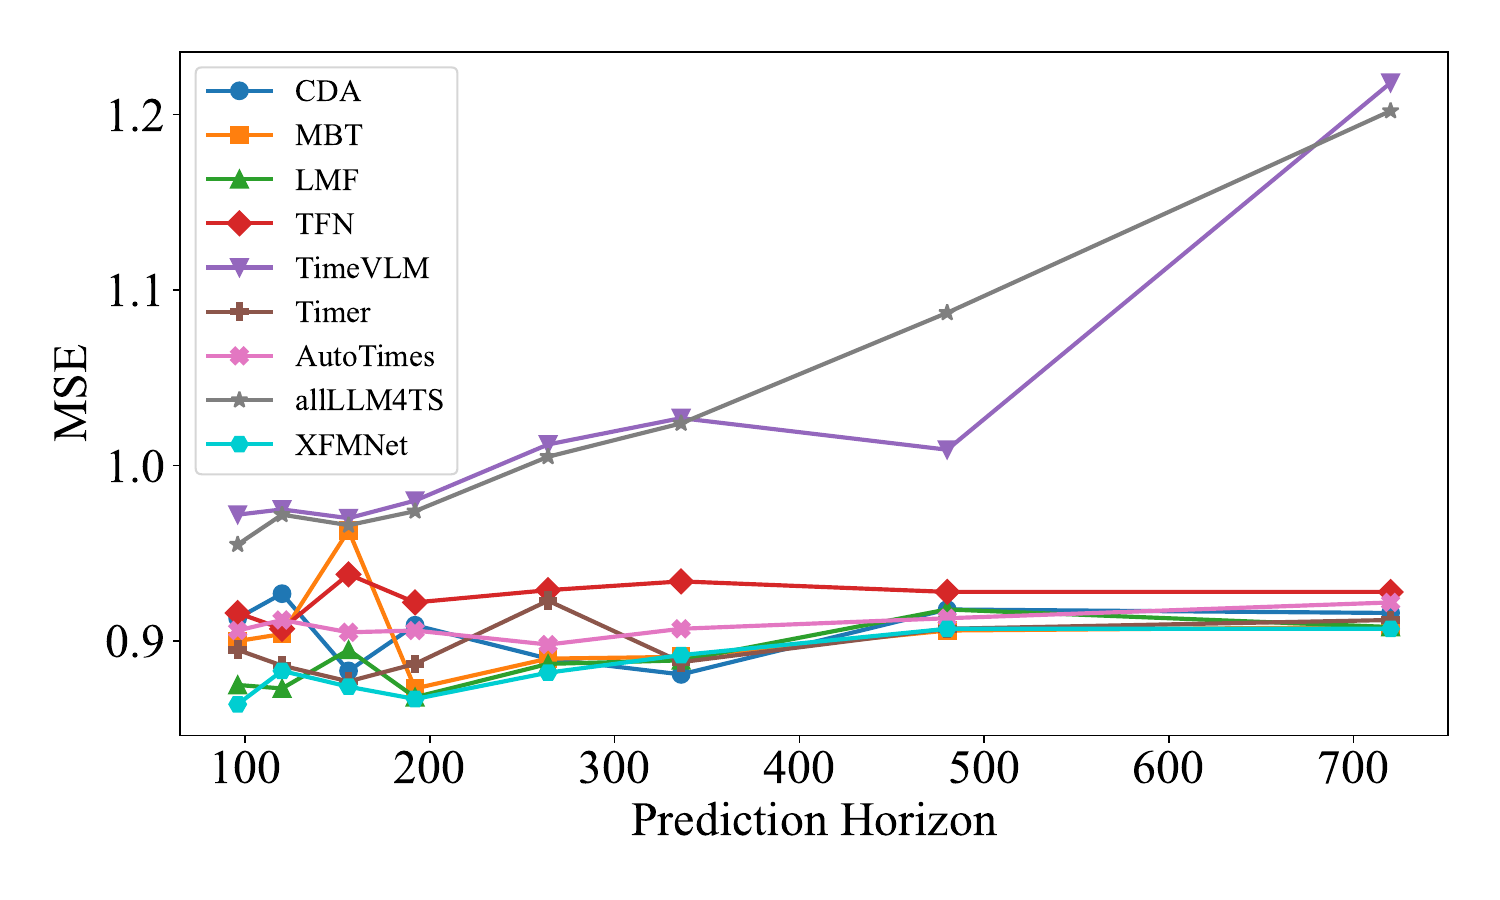}%
        \label{BJ3}
    }
    \quad
    \subfigure[MAE comparison on the second group of baseline models.]{%
        \includegraphics[width=0.95\columnwidth]{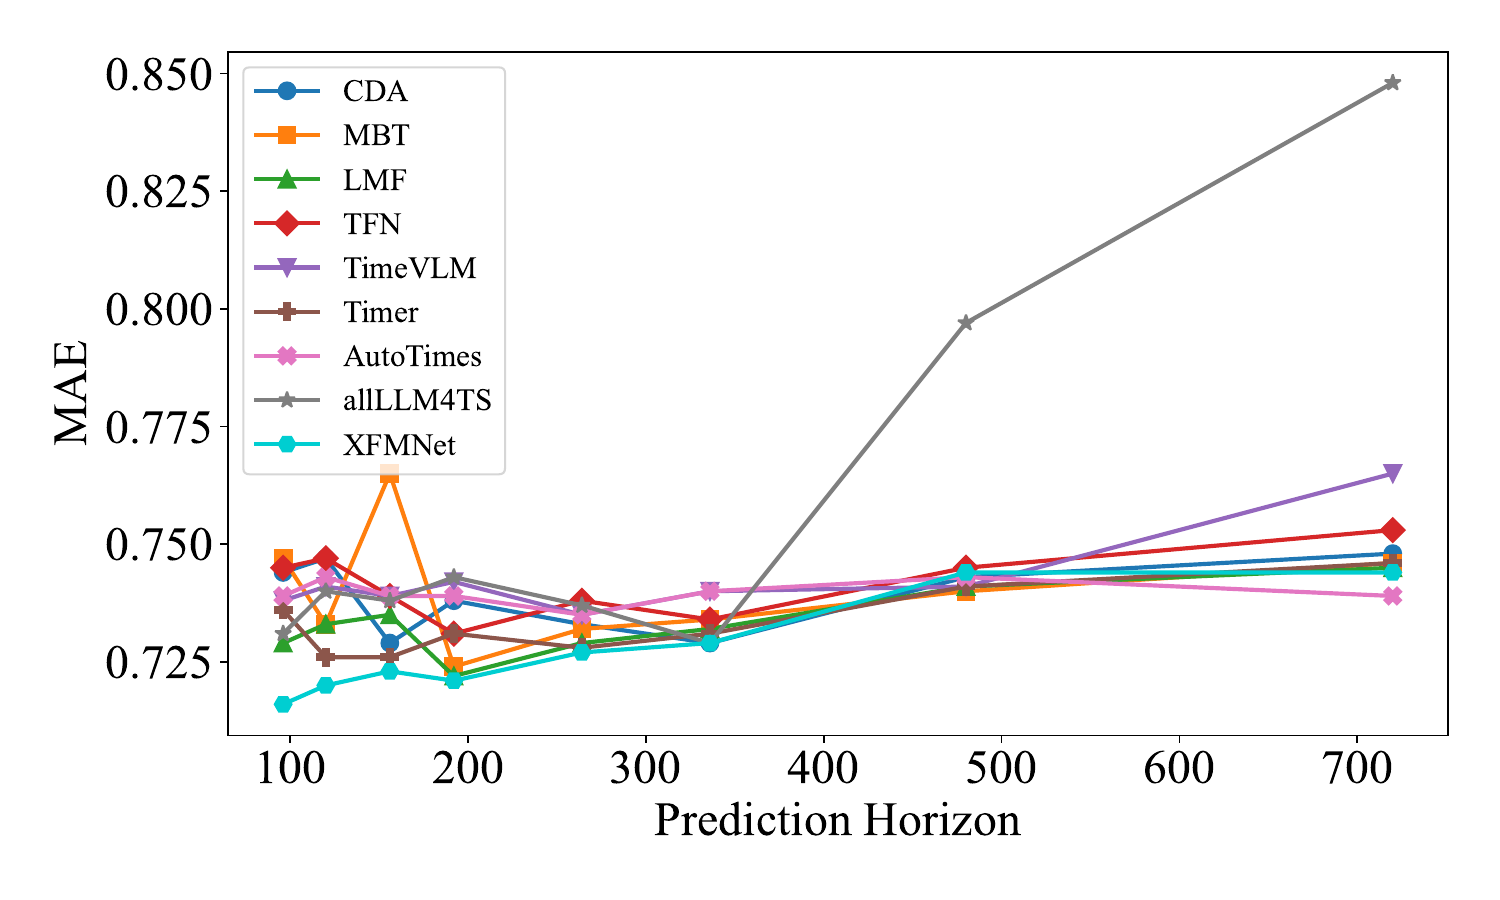}%
        \label{BJ4}
    }
    \caption{Performance comparison across different prediction horizons on the BJ dataset.}
    \label{BJ}
\end{figure}

%BTH
\begin{figure}[htbp]
    \centering
    \subfigure[MSE comparison on the first group of baseline models.]{%
        \includegraphics[width=0.95\columnwidth]{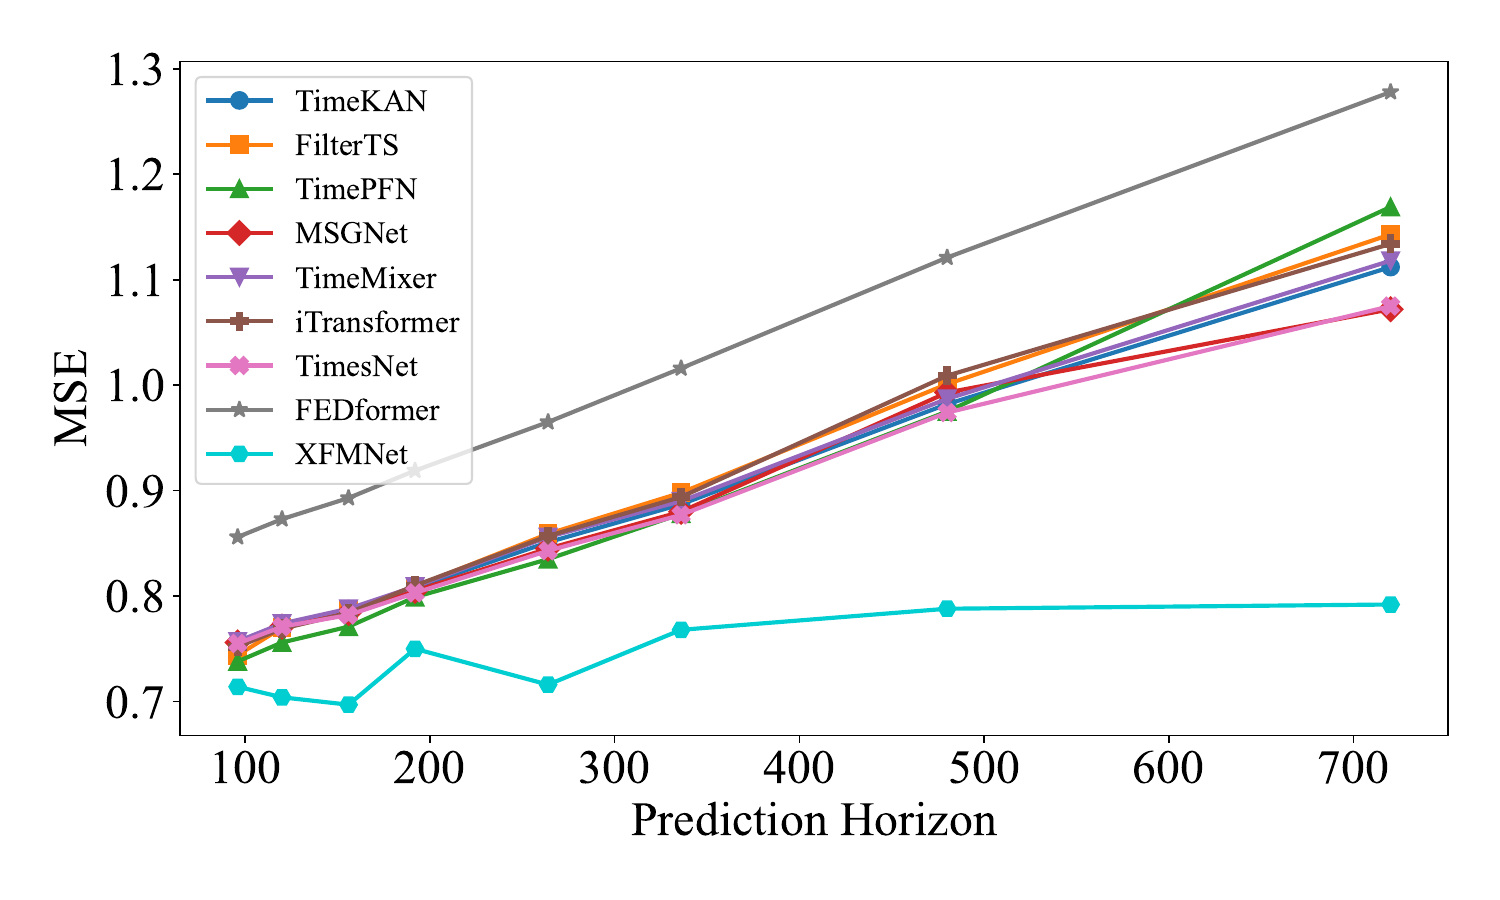}%
        \label{BTH1}
    }
    \quad
    \subfigure[MAE comparison on the first group of baseline models.]{%
        \includegraphics[width=0.95\columnwidth]{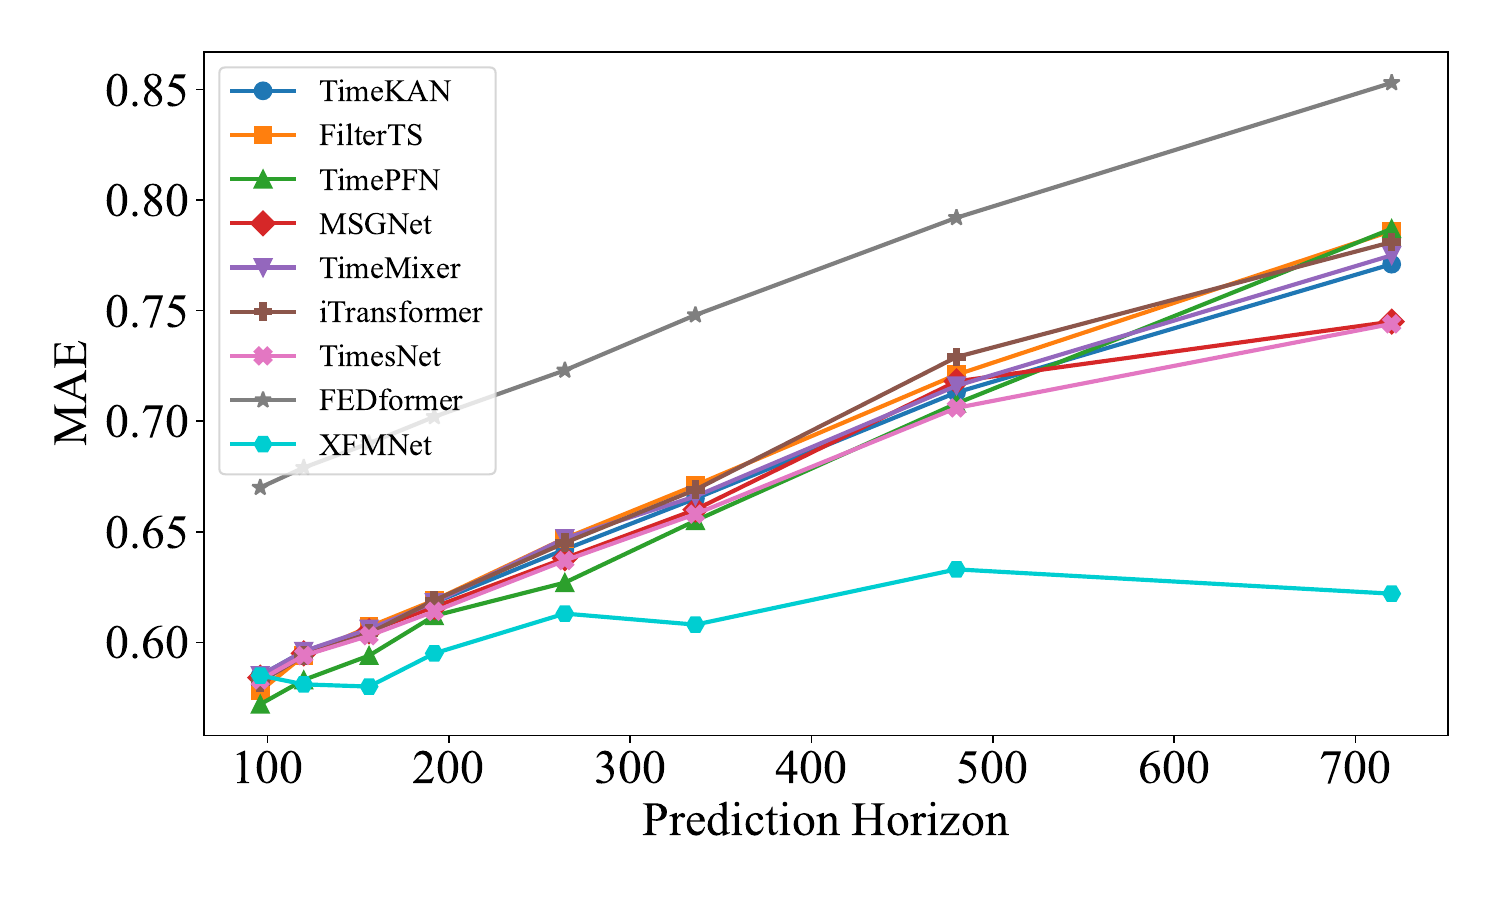}%
        \label{BTH2}
    }
    \quad
    \subfigure[MSE comparison on the second group of baseline models.]{%
        \includegraphics[width=0.95\columnwidth]{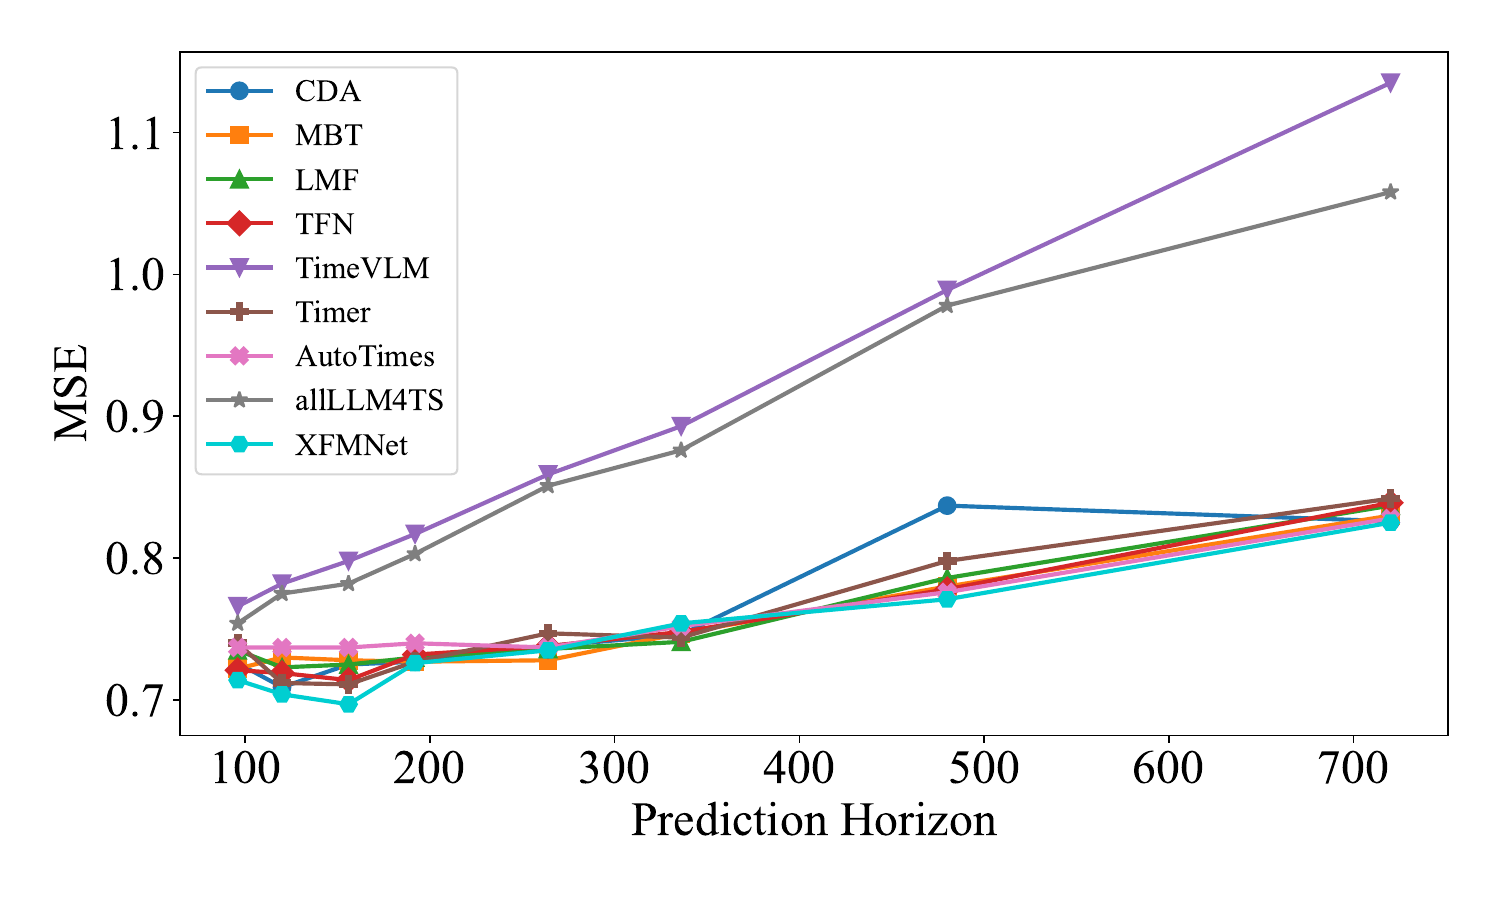}%
        \label{BTH3}
    }
    \quad
    \subfigure[MAE comparison on the second group of baseline models.]{%
        \includegraphics[width=0.95\columnwidth]{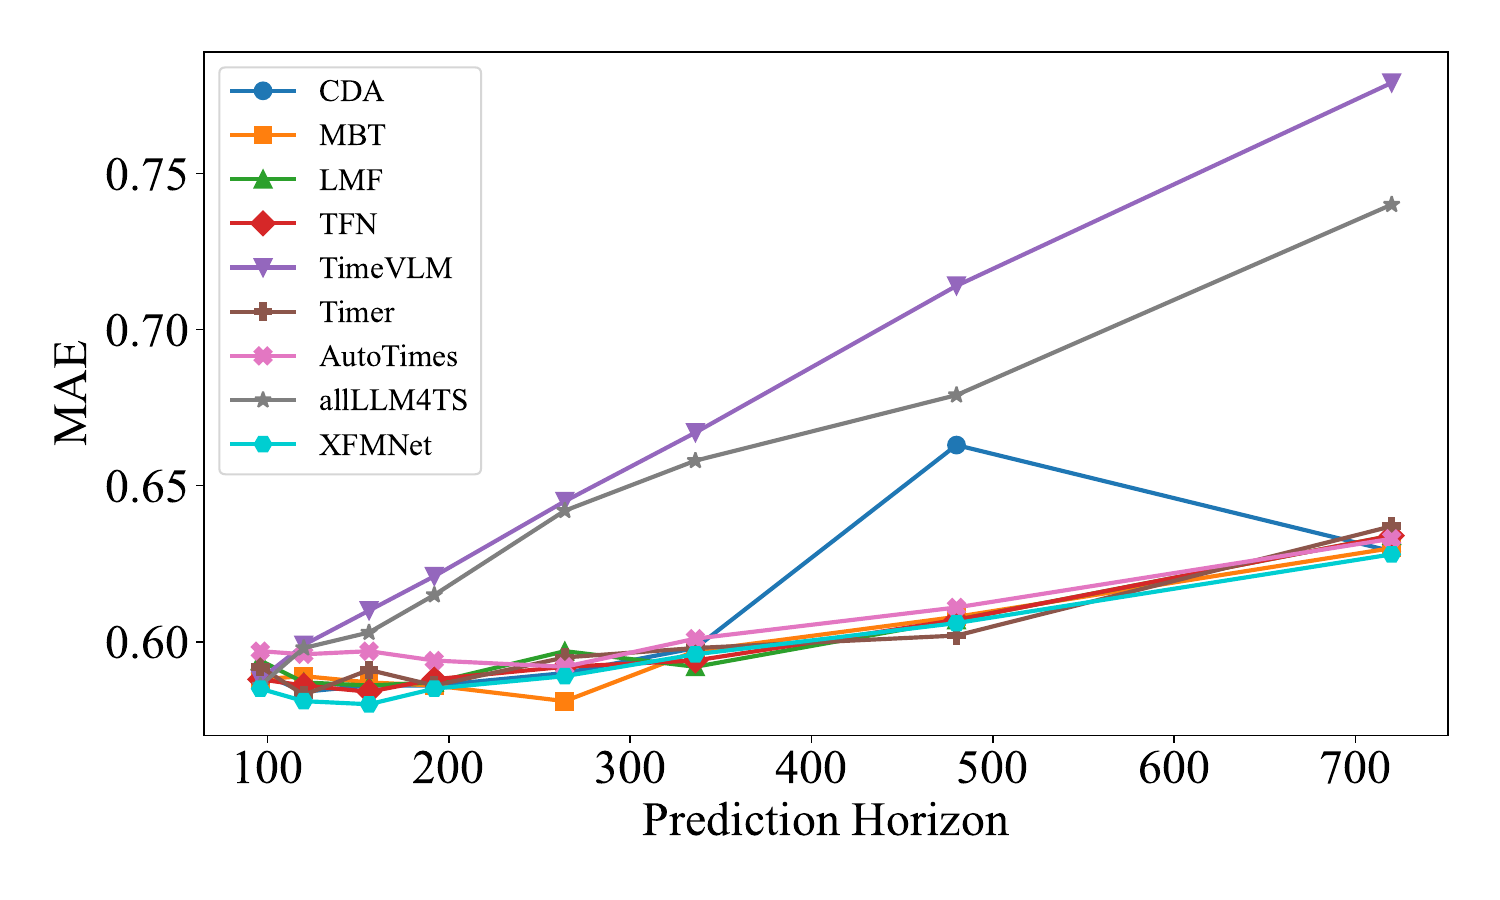}%
        \label{BTH4}
    }
    \caption{Performance comparison across different prediction horizons on the BTH dataset.}
    \label{BTH}
\end{figure}

%Ala
\begin{figure}[htbp]
    \centering
    \subfigure[MSE comparison on the first group of baseline models.]{%
        \includegraphics[width=0.95\columnwidth]{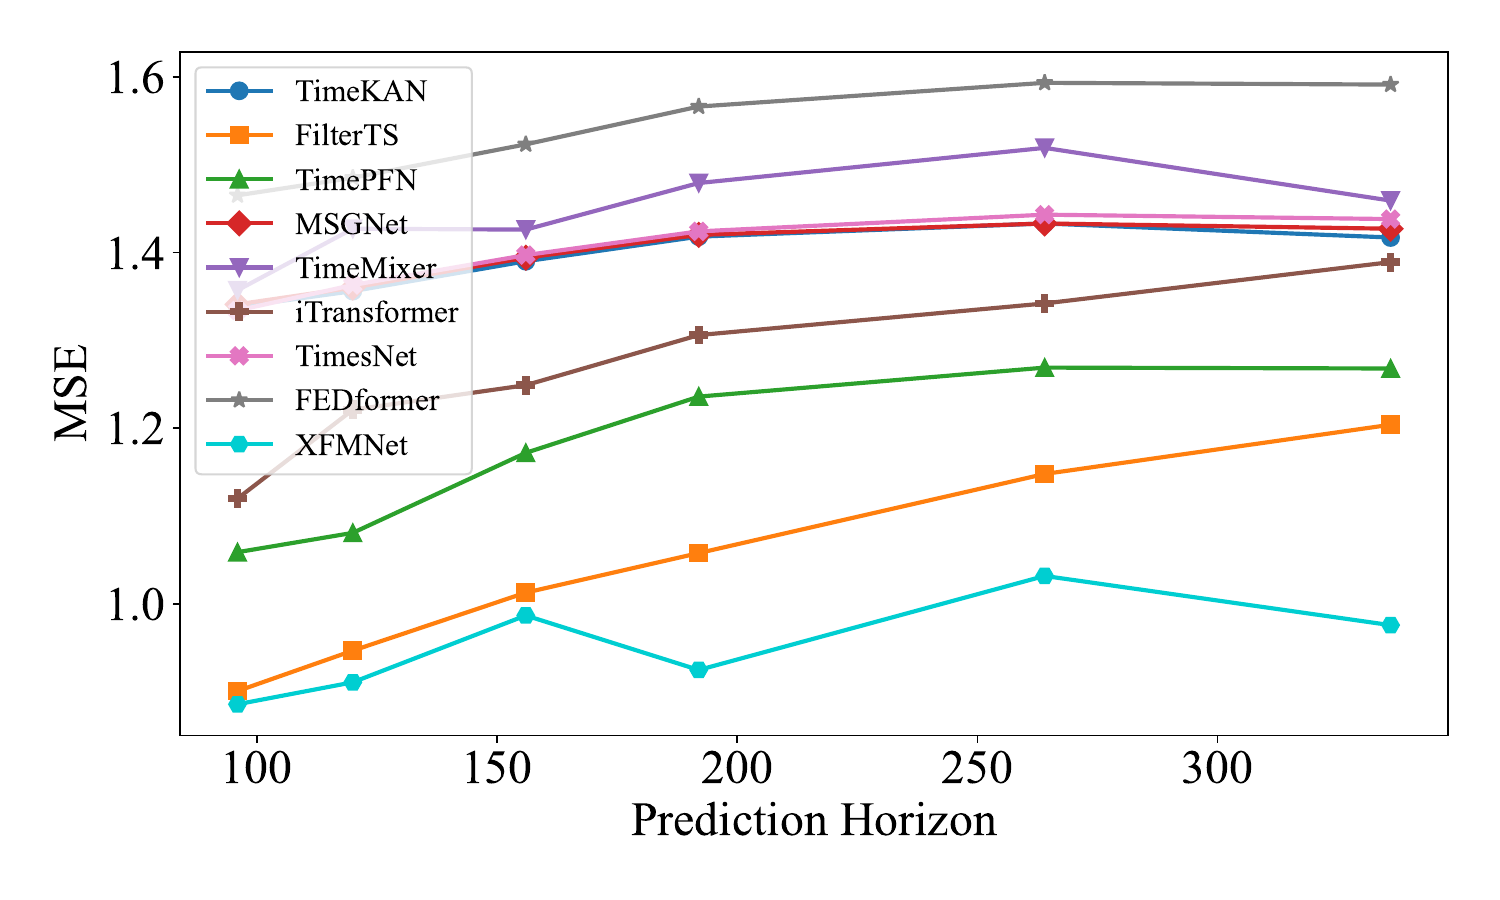}%
        \label{Ala1}
    }
    \quad
    \subfigure[MAE comparison on the first group of baseline models.]{%
        \includegraphics[width=0.95\columnwidth]{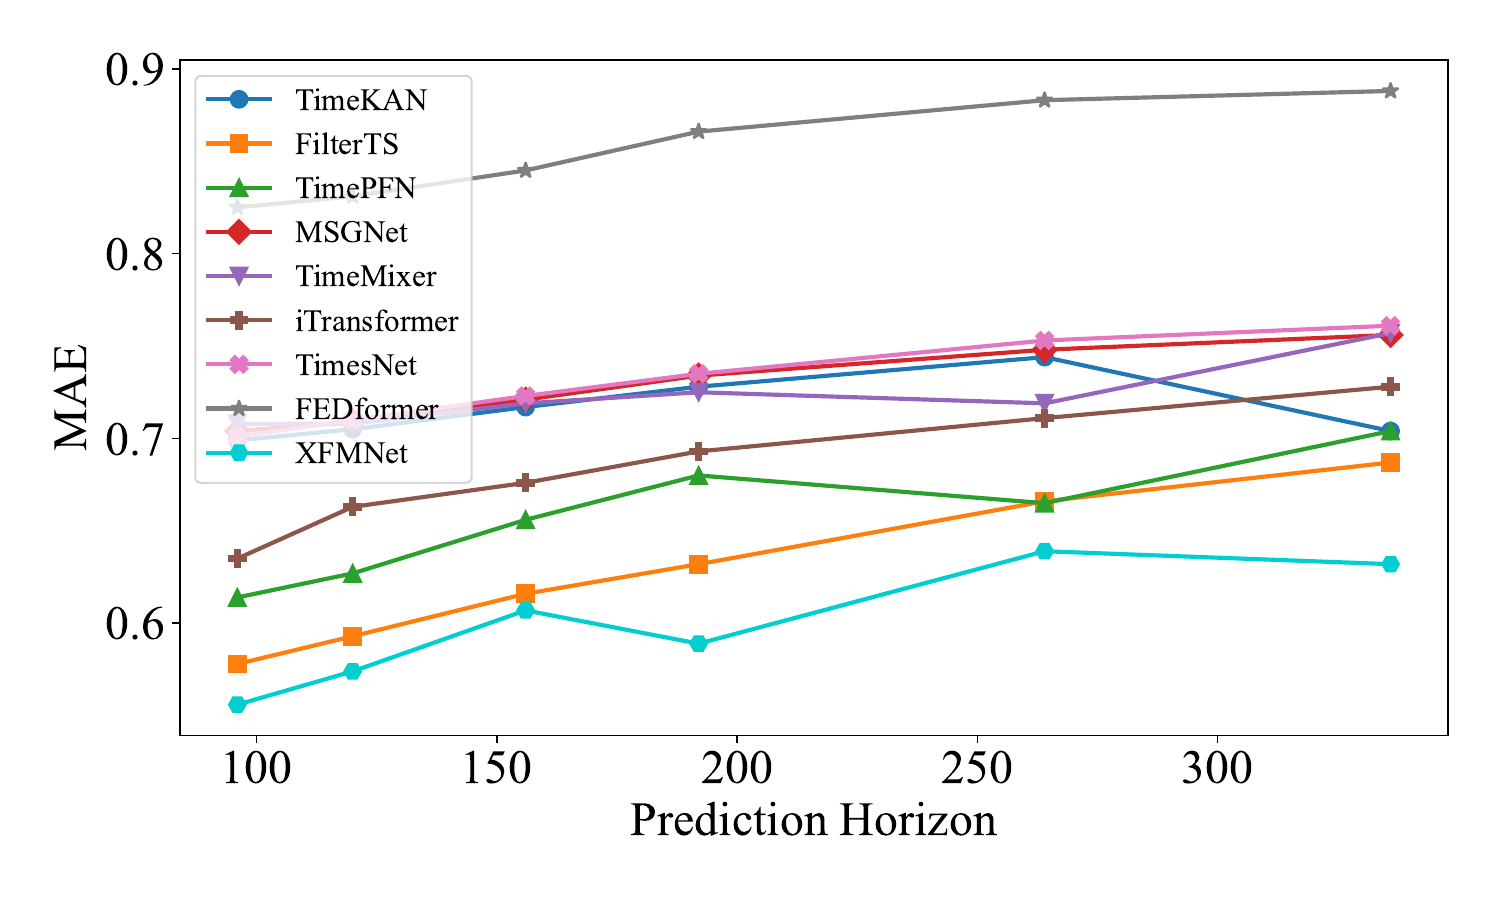}%
        \label{Ala2}
    }
    \quad
    \subfigure[MSE comparison on the second group of baseline models.]{%
        \includegraphics[width=0.95\columnwidth]{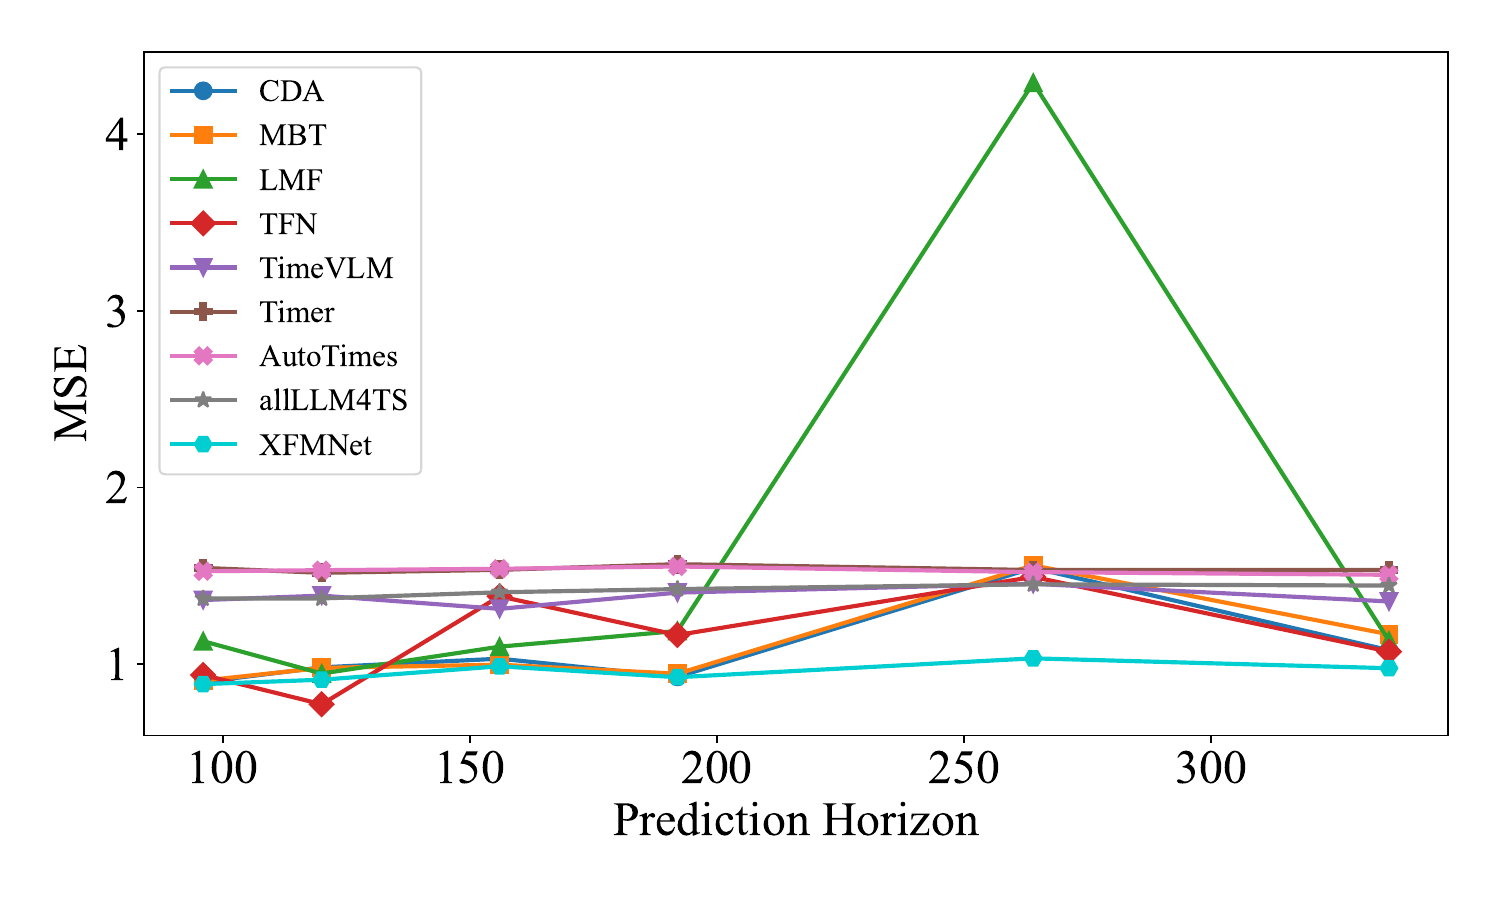}%
        \label{Ala3}
    }
    \quad
    \subfigure[MAE comparison on the second group of baseline models.]{%
        \includegraphics[width=0.95\columnwidth]{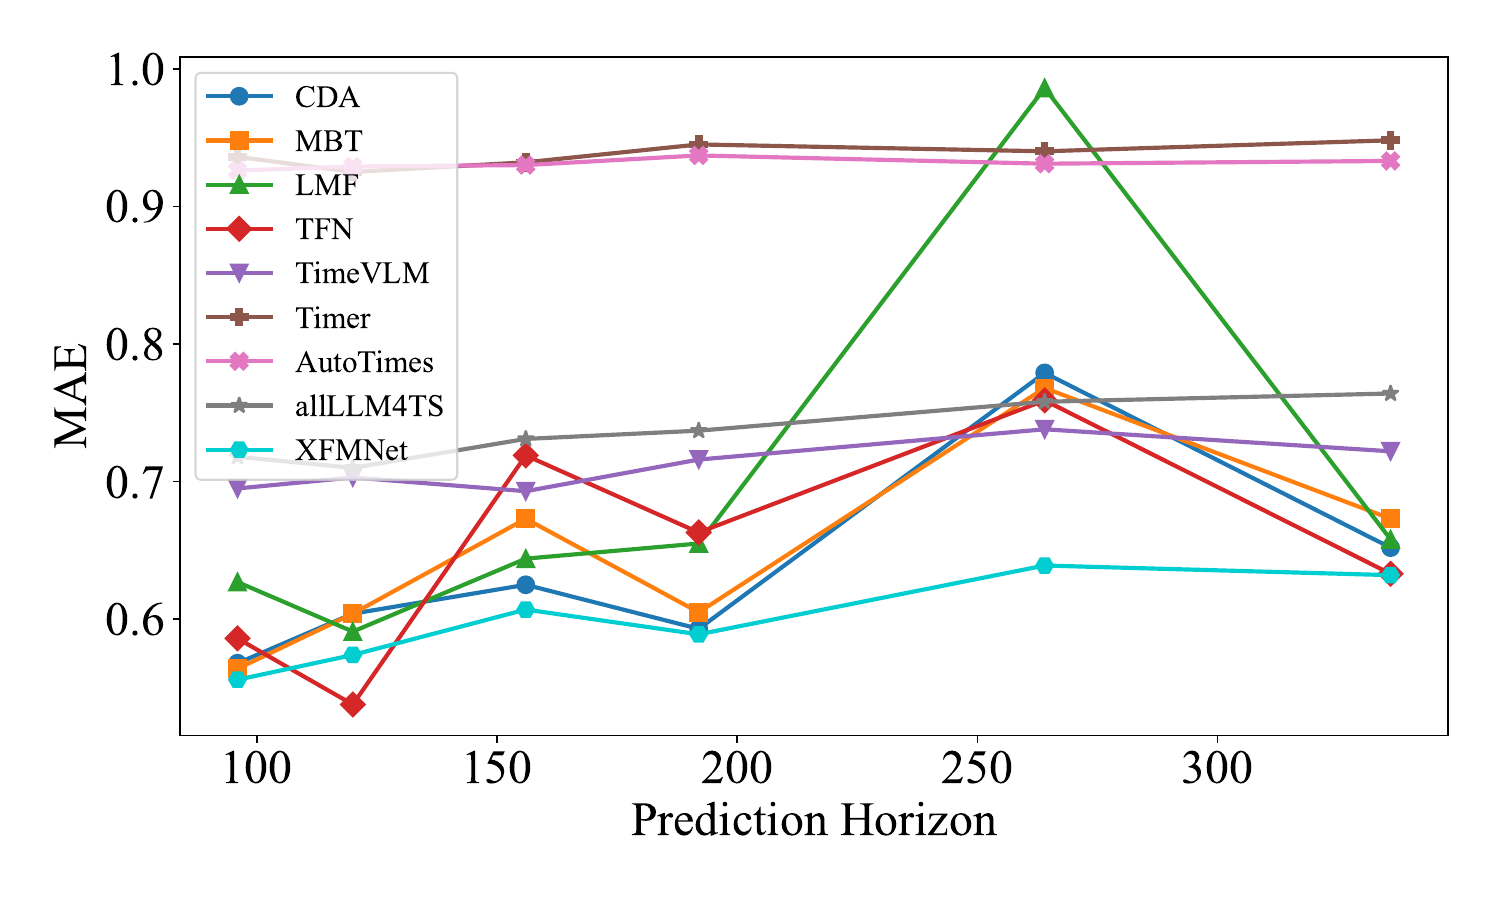}%
        \label{Ala4}
    }
    \caption{Performance comparison across different prediction horizons on the Ala dataset.}
    \label{Ala}
\end{figure}

\begin{comment}
\begin{figure}[t]
\centering  %图片全局居中
\subfigure[MSE]{
\label{pennu}
\includegraphics[width=0.5\columnwidth]{figure/radar_plot_final_mse.pdf}}\subfigure[MAE]{
\label{pendis}
\includegraphics[width=0.5\columnwidth]{figure/radar_plot_final_mae.pdf}}
\caption{Radar chart of average MSE and MAE across three datasets on the first group of baseline models.}
\label{ladar}
\end{figure}

\begin{figure}[t]
\centering  %图片全局居中
\subfigure[MSE]{
\label{pennu2}
\includegraphics[width=0.5\columnwidth]{figure/radar_plot_clean_mse2.pdf}}\subfigure[MAE]{
\label{pendis2}
\includegraphics[width=0.5\columnwidth]{figure/radar_plot_clean_mae2.pdf}}
\caption{Radar chart of average MSE and MAE across three datasets on the second group of baseline models.}
\label{ladar1}
\end{figure}
\end{comment}

\begin{figure}[t]
    \centering
    \subfigure[MSE (Group 1)]{
        \includegraphics[width=0.48\columnwidth]{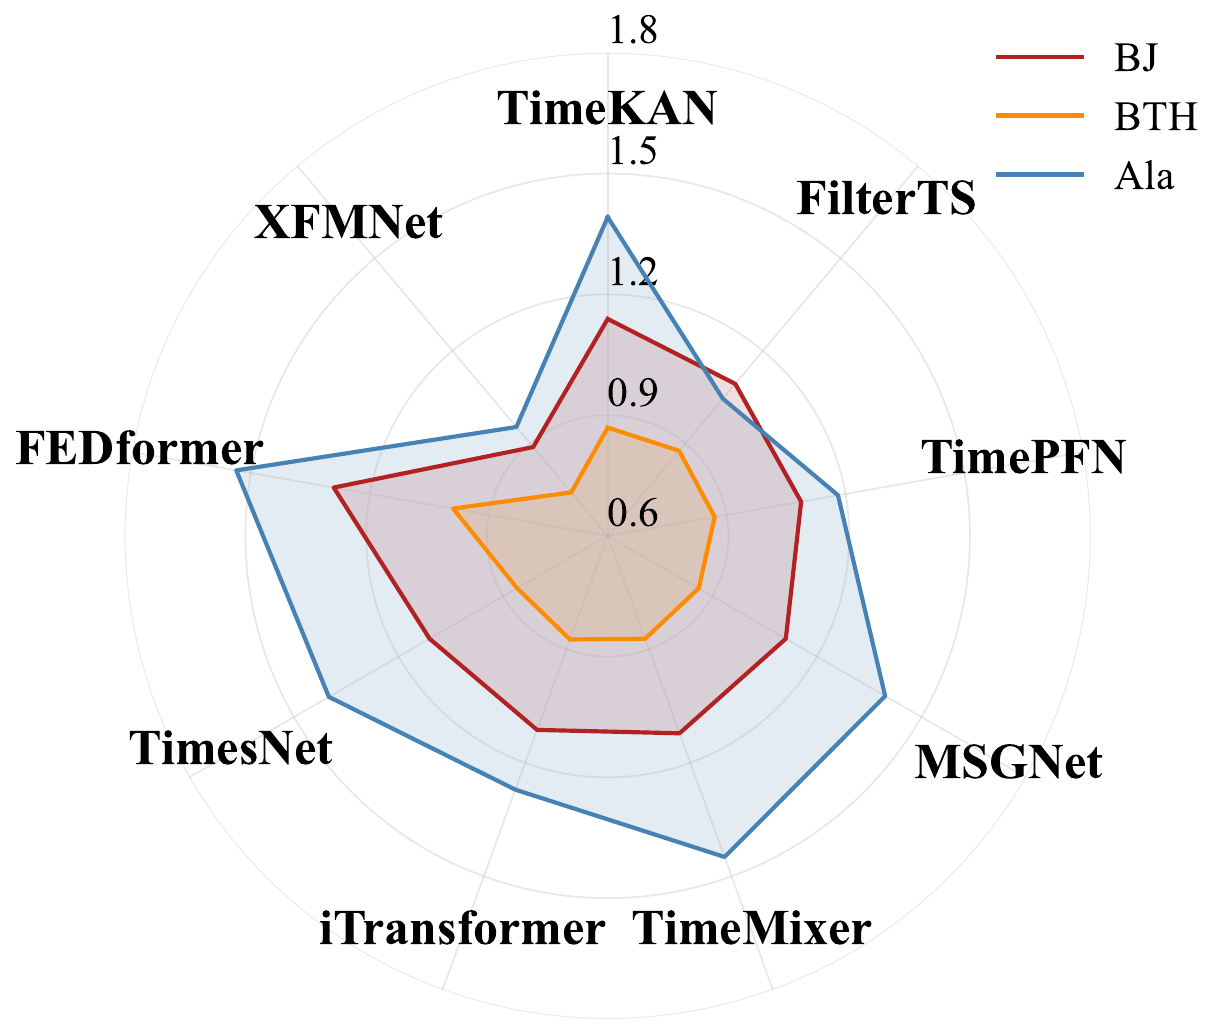}}
    \subfigure[MAE (Group 1)]{
        \includegraphics[width=0.48\columnwidth]{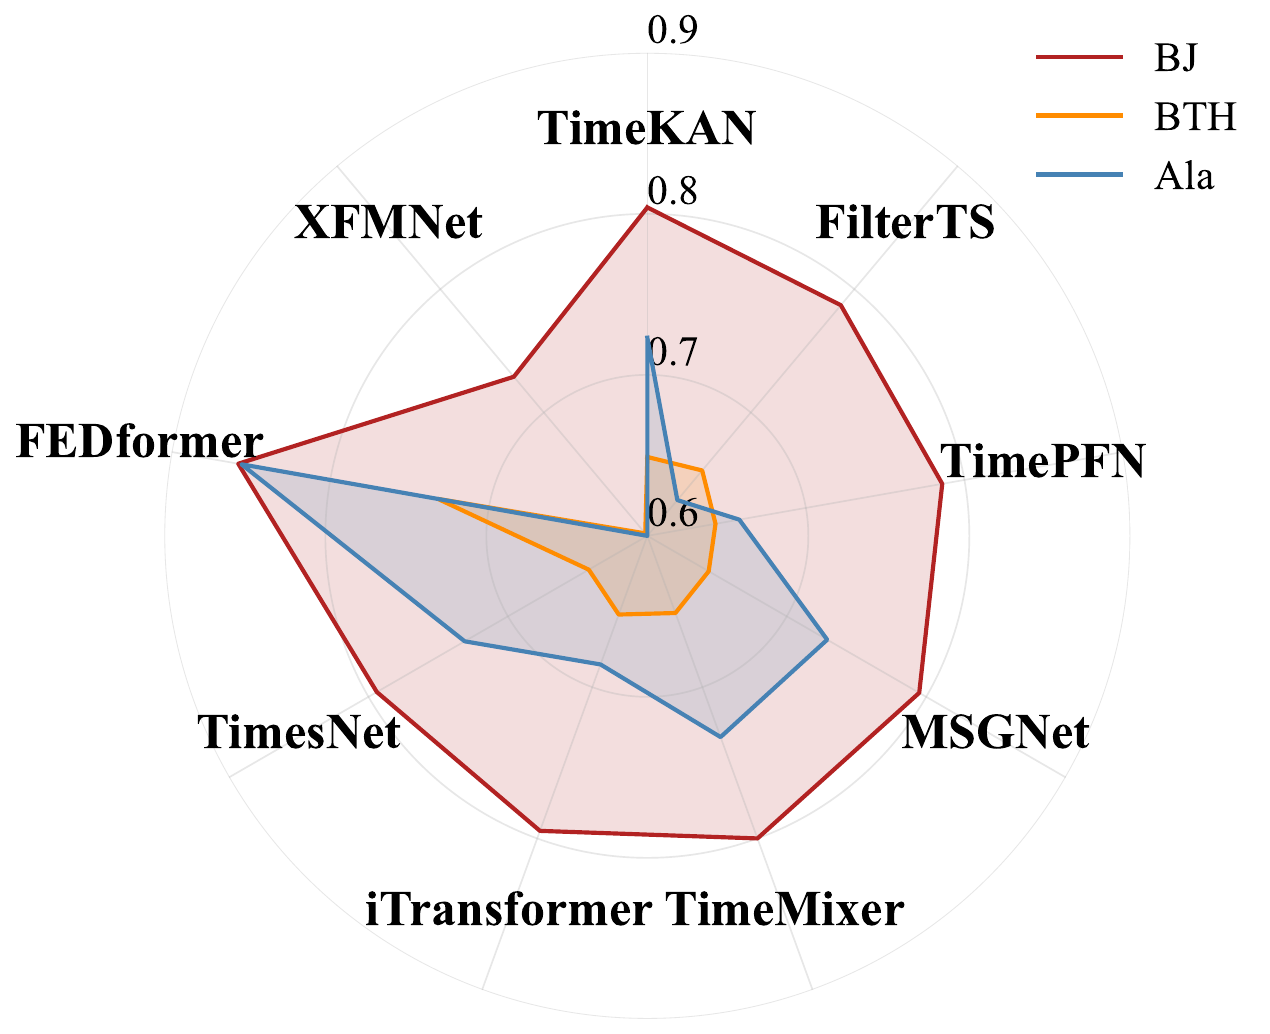}}\\
    \subfigure[MSE (Group 2)]{
        \includegraphics[width=0.48\columnwidth]{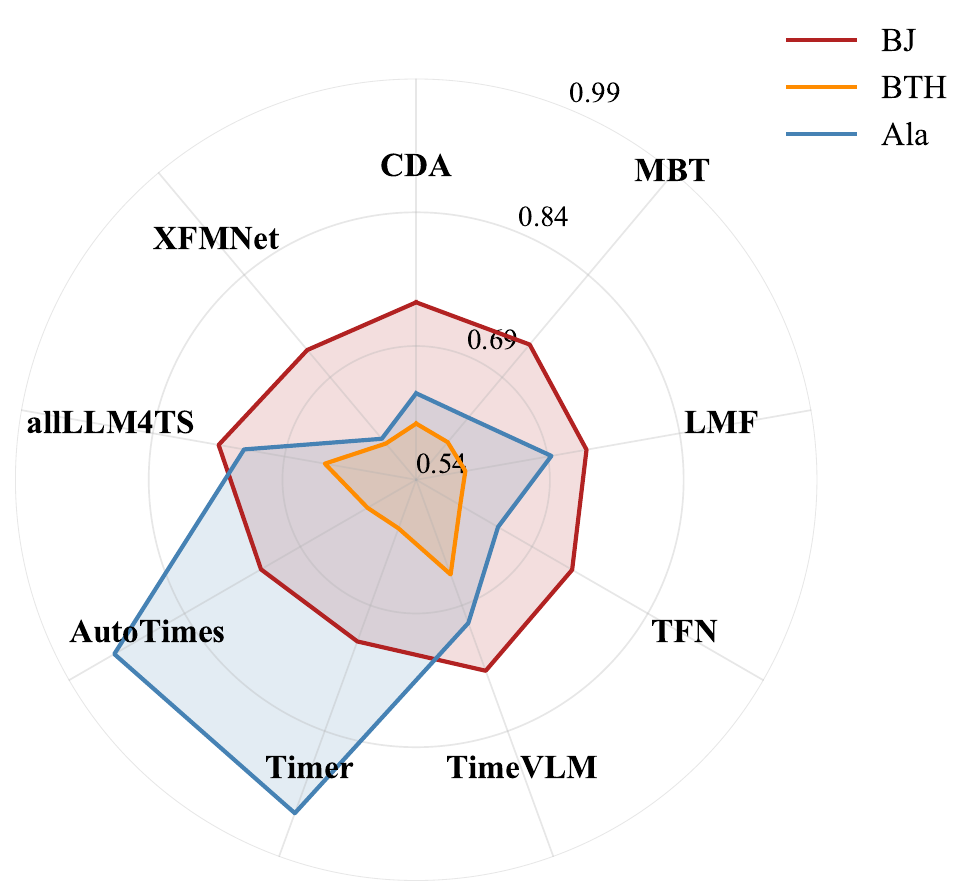}}
    \subfigure[MAE (Group 2)]{
        \includegraphics[width=0.48\columnwidth]{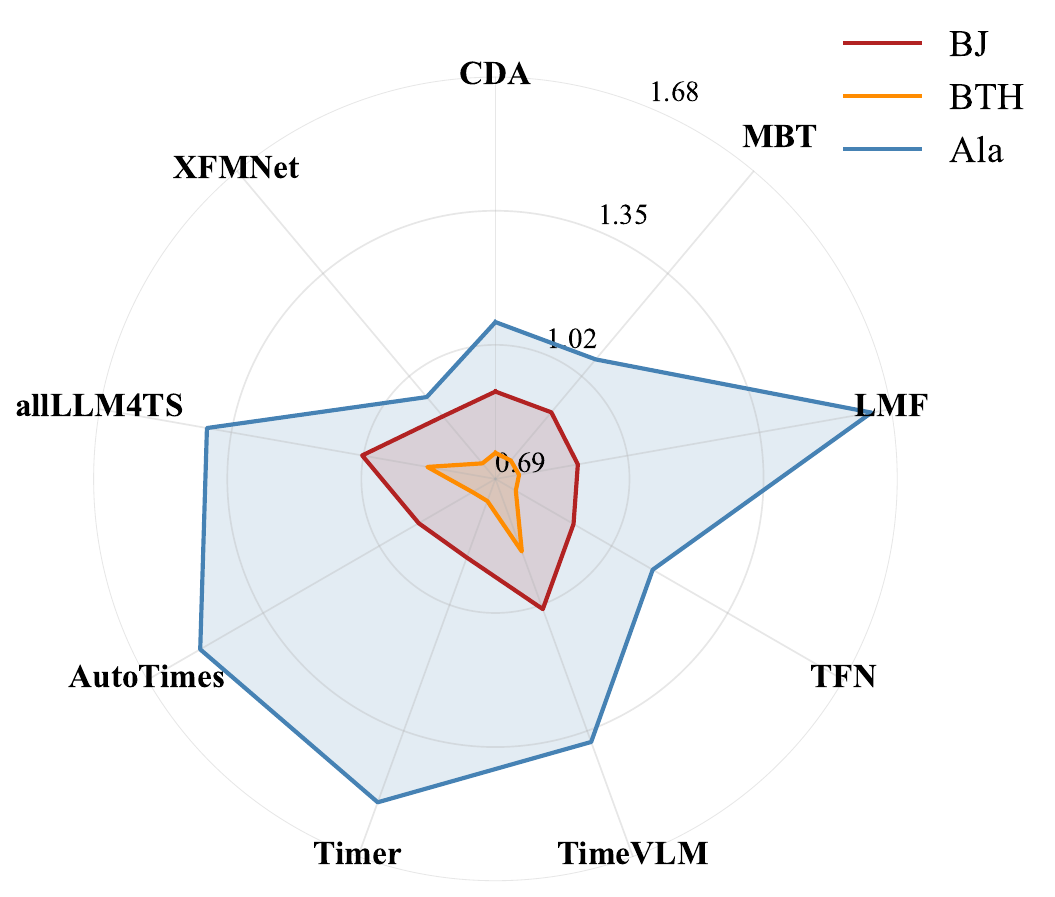}}
    \caption{Radar charts of average MSE and MAE across three datasets on two groups of baseline models.}
    \label{ladarall}
\end{figure}

\begin{table*}[t!]
\centering
\small
\setlength{\tabcolsep}{2.6pt}
\renewcommand{\arraystretch}{1.3}
\caption{Long-term prediction results on three real-world datasets under varying prediction horizons. We highlight the best and the second-best results in \textbf{bold} and \underline{underline}, respectively.}
\begin{tabular}{c@{\hskip 10pt}c
@{\hskip 6pt}|c@{\hskip 2.5pt}c
@{\hskip 6pt}|c@{\hskip 2.5pt}c
@{\hskip 6pt}|c@{\hskip 2.5pt}c
@{\hskip 6pt}|c@{\hskip 2.5pt}c
@{\hskip 6pt}|c@{\hskip 2.5pt}c
@{\hskip 6pt}|c@{\hskip 2.5pt}c
@{\hskip 6pt}|c@{\hskip 2.5pt}c
@{\hskip 6pt}|c@{\hskip 2.5pt}c
@{\hskip 6pt}|c@{\hskip 2.5pt}c}
\toprule
%\multirow{3.5}{*}{Data} & \multirow{3.5}{*}{Horizon} 
%\multirow{3}{*}{Metric}
\multicolumn{2}{c|}{\multirow{2}{*}{Model}} & \multicolumn{2}{c}{TimeKAN} & \multicolumn{2}{c}{FilterTS} & \multicolumn{2}{c}{TimePFN} 
& \multicolumn{2}{c}{MSGNet} & \multicolumn{2}{c}{TimeMixer} &  \multicolumn{2}{c}{iTransformer} & \multicolumn{2}{c}{TimesNet} & \multicolumn{2}{c}{FEDformer} & \multicolumn{2}{c}{XFMNet} \\
& & \multicolumn{2}{c}{(2025)} & \multicolumn{2}{c}{(2025)} & \multicolumn{2}{c}{(2025)} & \multicolumn{2}{c}{(2024)} & \multicolumn{2}{c}{(2024)} & \multicolumn{2}{c}{(2024)} & \multicolumn{2}{c}{(2023)} & \multicolumn{2}{c}{(2022)} & \multicolumn{2}{c}{(ours)}\\
\cmidrule(lr){1-2} \cmidrule(lr){3-4} \cmidrule(lr){5-6} \cmidrule(lr){7-8} \cmidrule(lr){9-10} \cmidrule(lr){11-12} \cmidrule(lr){13-14} \cmidrule(lr){15-16} \cmidrule(lr){17-18}  \cmidrule(lr){19-20} 
\multicolumn{2}{c|}{Metric} & MSE & MAE & MSE & MAE & MSE & MAE & MSE & MAE & MSE & MAE & MSE & MAE & MSE & MAE & MSE & MAE & MSE & MAE\\
\midrule
\multirow{9}{*}{\rotatebox{90}{BJ}} 
& 96  & 0.952 & 0.731 & 0.926 & \underline{0.717} & \underline{0.922} & \underline{0.717} & 0.952 & 0.730 & 0.960 & 0.735 & 0.948 & 0.728 & 0.951 & 0.730 & 1.042 & 0.777 & \textbf{0.864} & \textbf{0.716} \\
& 120 & 0.965 & 0.737 & 0.946 & 0.727 & \underline{0.937} & \underline{0.723} & 0.965 & 0.736 & 0.968 & 0.738 & 0.956 & 0.732 & 0.969 & 0.737 & 1.072 & 0.791 & \textbf{0.883} & \textbf{0.720} \\
& 156 & 0.967 & 0.739 & \underline{0.949} & \underline{0.730} & 0.951 & 0.731 & 0.963 & 0.737 & 0.969 & 0.738 & 0.954 & 0.732 & 0.961 & 0.735 & 1.053 & 0.783 & \textbf{0.874} & \textbf{0.723} \\
& 192 & 1.089 & 0.782 & \underline{1.057} & \underline{0.767} & 1.064 & 0.772 & 1.091 & 0.782 & 1.092 & 0.783 & 1.089 & 0.780 & 1.090 & 0.781 & 1.233 & 0.845 & \textbf{0.867} & \textbf{0.721} \\
& 264 & 1.141 & 0.803 & \underline{1.121} & \underline{0.794} & \underline{1.121} & 0.796 & 1.143 & 0.804 & 1.162 & 0.813 & 1.148 & 0.804 & 1.142 & 0.802 & 1.593 & 0.883 & \textbf{0.882} & \textbf{0.727} \\
& 336 & 1.165 & 0.818 & 1.153 & 0.812 & \underline{1.146} & \underline{0.811} & 1.168 & 0.819 & 1.214 & 0.837 & 1.176 & 0.822 & 1.166 & 0.817 & 1.337 & 0.887 & \textbf{0.929} & \textbf{0.746} \\
& 480 & 1.464 & 0.920 & 1.225 & 0.844 & \underline{1.215} & \underline{0.840} & 1.237 & 0.849 & 1.237 & 0.850 & 1.243 & 0.850 & 1.236 & 0.847 & 1.432 & 0.924 & \textbf{0.924} & \textbf{0.747} \\
& 720 & 1.371 & 0.905 & 1.370 & 0.903 & \underline{1.351} & \underline{0.897} & 1.372 & 0.904 & 1.376 & 0.905 & 1.389 & 0.909 & 1.374 & 0.904 & 1.563 & 0.972 & \textbf{0.907} & \textbf{0.744} \\
& Avg & 1.139 & 0.804 & 1.093 & 0.787 &  \underline{1.088} &  \underline{0.786} & 1.111 & 0.795 & 1.122 & 0.800 & 1.113 & 0.795 & 1.111 & 0.794 & 1.291 & 0.858 & \textbf{0.891} & \textbf{0.730}\\
\midrule
\multirow{9}{*}{\rotatebox{90}{BTH}} 
& 96  & 0.757 & 0.585 & 0.744 & \underline{0.578} & \underline{0.738} & \textbf{0.572} & 0.756 & 0.584 & 0.757 & 0.585 & 0.752 & 0.582 & 0.755 & 0.583 & 0.856 & 0.670 & \textbf{0.714} & 0.585 \\
& 120 & 0.773 & 0.596 & 0.770 & 0.594 & \underline{0.756} & \underline{0.583} & 0.771 & 0.595 & 0.774 & 0.596 & 0.769 & 0.594 & 0.771 & 0.594 & 0.873 & 0.679 & \textbf{0.704} & \textbf{0.581} \\
& 156 & 0.785 & 0.605 & 0.787 & 0.607 & \underline{0.771} & \underline{0.594} & 0.784 & 0.605 & 0.788 & 0.606 & 0.784 & 0.604 & 0.782 & 0.603 & 0.893 & 0.690 & \textbf{0.697} & \textbf{0.580} \\
& 192 & 0.808 & 0.618 & 0.809 & 0.619 & \underline{0.799} & \underline{0.612} & 0.805 & 0.616 & 0.809 & 0.618 & 0.810 & 0.619 & 0.803 & 0.614 & 0.919 & 0.702 & \textbf{0.726} & \textbf{0.585} \\
& 264 & 0.851 & 0.642 & 0.859 & 0.647 & \underline{0.835} & \underline{0.627} & 0.845 & 0.638 & 0.856 & 0.647 & 0.857 & 0.645 & 0.843 & 0.637 & 0.965 & 0.723 & \textbf{0.735} & \textbf{0.589} \\
& 336 & 0.887 & 0.665 & 0.898 & 0.671 & 0.878 & \underline{0.655} & 0.880 & 0.660 & 0.890 & 0.666 & 0.894 & 0.669 & \underline{0.877} & 0.658 & 1.016 & 0.748 & \textbf{0.754} & \textbf{0.596} \\
& 480 & 0.982 & 0.713 & 1.001 & 0.721 & 1.015 & 0.713 & 0.975 & 0.708 & 0.987 & 0.716 & 0.993 & 0.718 & \underline{0.974} & \underline{0.706} & 1.121 & 0.792 & \textbf{0.771} & \textbf{0.606} \\
& 720 & 1.112 & 0.771 & 1.143 & 0.786 & 1.169 & 0.787 & \underline{1.072} & 0.745 & 1.118 & 0.775 & 1.134 & 0.781 & 1.075 & \underline{0.744} & 1.278 & 0.853 & \textbf{0.825} & \textbf{0.628} \\
& Avg & 0.869 & 0.649 & 0.876 & 0.653 & 0.870 & 0.643 & 0.861 & 0.644 & 0.872 & 0.651 & 0.874 & 0.652 & \underline{0.860} & \underline{0.642} & 0.990 & 0.732 & \textbf{0.740} & \textbf{0.593}\\
\midrule

\multirow{7}{*}{\rotatebox{90}{Ala}} 
& 96 & 1.338 & 0.699 & \underline{0.901} & \underline{0.578} & 1.059 & 0.614 & 1.341 & 0.704 & 1.357 & 0.708 & 1.120 & 0.635 & 1.334 & 0.701 & 1.465 & 0.825 & \textbf{0.886} & \textbf{0.556} \\
& 120 & 1.356 & 0.705 & \underline{0.947} & \underline{0.593} & 1.081 & 0.627 & 1.360 & 0.709 & 1.427 & 0.708 & 1.221 & 0.663 & 1.363 & 0.710 & 1.485 & 0.831 & \textbf{0.911} & \textbf{0.574} \\
& 156 & 1.390 & 0.717 & \underline{1.013} & \underline{0.616} & 1.172 & 0.656 & 1.394 & 0.721 & 1.436 & 0.719 & 1.249 & 0.676 & 1.397 & 0.723 & 1.523 & 0.845 & \textbf{0.987} & \textbf{0.607} \\
& 192 & 1.418 & 0.728 & \underline{1.058} & \underline{0.632} & 1.236 & 0.680 & 1.421 & 0.734 & 1.479 & 0.725 & 1.306 & 0.693 & 1.424 & 0.735 & 1.566 & 0.866 & \textbf{0.925} & \textbf{0.589} \\
& 264 & 1.433 & 0.744 & \underline{1.148} & 0.666 & 1.269 & \underline{0.665} & 1.433 & 0.748 & 1.519 & 0.778 & 1.342 & 0.712 & 1.443 & 0.753 & 1.593 & 0.883 & \textbf{1.032} & \textbf{0.639} \\
& 336 & 1.417 & 0.747 & \underline{1.204} & \underline{0.687} & 1.268 & 0.704 & 1.427 & 0.756 & 1.475 & 0.757 & 1.389 & 0.728 & 1.438 & 0.761 & 1.591 & 0.888 & \textbf{0.976} & \textbf{0.632} \\
& Avg & 1.392 & 0.723 & \underline{1.045} & \underline{0.629} & 1.181 & 0.658 & 1.396 & 0.729 & 1.449 & 0.733 & 1.271 & 0.685 & 1.400 & 0.731 & 1.537 & 0.856 & \textbf{0.953} & \textbf{0.600}\\

\bottomrule
\end{tabular}
\label{tab:main_results}
\end{table*}

%In addition, we compare \texttt{XFMnet} with other multimodal fusion strategies and large multimodal model. The results are shown in Table \ref{multimodallarge} and Figs. \ref{} to \ref{}. It is shown that

\begin{table*}[t!]
\centering
\small
\setlength{\tabcolsep}{2.6pt}
\renewcommand{\arraystretch}{1.3}
\caption{Comparison of different fusion strategies and multimodal models. We highlight the best and the second-best results in \textbf{bold} and \underline{underline}, respectively.}
\begin{tabular}{c@{\hskip 10pt}c
@{\hskip 6pt}|c@{\hskip 2.5pt}c
@{\hskip 6pt}|c@{\hskip 2.5pt}c
@{\hskip 6pt}|c@{\hskip 2.5pt}c
@{\hskip 6pt}|c@{\hskip 2.5pt}c
@{\hskip 6pt}|c@{\hskip 2.5pt}c
@{\hskip 6pt}|c@{\hskip 2.5pt}c
@{\hskip 6pt}|c@{\hskip 2.5pt}c
@{\hskip 6pt}|c@{\hskip 2.5pt}c
@{\hskip 6pt}|c@{\hskip 2.5pt}c}
\toprule
%\multirow{3.5}{*}{Data} & \multirow{3.5}{*}{Horizon} 
%\multirow{3}{*}{Metric}
\multicolumn{2}{c|}{\multirow{2}{*}{Model}} & \multicolumn{2}{c}{CDA} & \multicolumn{2}{c}{MBT} & \multicolumn{2}{c}{LMF} 
& \multicolumn{2}{c}{TFN} & \multicolumn{2}{c}{TimeVLM} &  \multicolumn{2}{c}{Timer} & \multicolumn{2}{c}{AutoTimes} & \multicolumn{2}{c}{allLLM4TS} & \multicolumn{2}{c}{XFMNet} \\
& & \multicolumn{2}{c}{(2024)} & \multicolumn{2}{c}{(2025)} & \multicolumn{2}{c}{(2025)} & \multicolumn{2}{c}{(2024)} & \multicolumn{2}{c}{(2025)} & \multicolumn{2}{c}{(2024)} & \multicolumn{2}{c}{(2024)} & \multicolumn{2}{c}{(2024)} & \multicolumn{2}{c}{(ours)}\\
\cmidrule(lr){1-2} \cmidrule(lr){3-4} \cmidrule(lr){5-6} \cmidrule(lr){7-8} \cmidrule(lr){9-10} \cmidrule(lr){11-12} \cmidrule(lr){13-14} \cmidrule(lr){15-16} \cmidrule(lr){17-18}  \cmidrule(lr){19-20} 
\multicolumn{2}{c|}{Metric} & MSE & MAE & MSE & MAE & MSE & MAE & MSE & MAE & MSE & MAE & MSE & MAE & MSE & MAE & MSE & MAE & MSE & MAE\\
\midrule
\multirow{9}{*}{\rotatebox{90}{BJ}} 
& 96  & 0.913 & 0.744 & 0.900 & 0.738 & \underline{0.875} & \underline{0.725} & 0.916 & 0.745 & 0.972 & 0.738 & 0.895 & 0.736 & 0.906 & 0.739 & 0.955 & 0.731 & \textbf{0.864} & \textbf{0.716} \\
& 120 & 0.927 & 0.747 & 0.904 & 0.733 & 0.904 & 0.737 & 0.907 & 0.741 & 0.975 & 0.741 & \underline{0.886} & \underline{0.726} & 0.912 & 0.743 & 0.972 & 0.740 & \textbf{0.883} & \textbf{0.720} \\
& 156 & \underline{0.883} & 0.729 & 0.963 & 0.765 & 0.895 & 0.735 & 0.898 & 0.736 & 0.970 & 0.739 & 0.877 & \underline{0.726} & 0.905 & 0.739 & 0.966 & 0.738 & \textbf{0.874} & \textbf{0.723} \\
& 192 & 0.909 & 0.738 & 0.873 & 0.724 & 0.899 & 0.736 & \underline{0.868} & \underline{0.722} & 0.980 & 0.744 & 0.887 & 0.731 & 0.906 & 0.739 & 0.974 & 0.743 & \textbf{0.867} & \textbf{0.721} \\
& 264 & 0.890 & 0.733 & 0.890 & 0.732 & \underline{0.887} & \underline{0.729} & 0.920 & 0.741 & 1.012 & 0.758 & 0.923 & 0.728 & 0.898 & 0.735 & 1.005 & 0.754 & \textbf{0.882} & \textbf{0.727} \\
& 336 & \textbf{0.881} & \textbf{0.729} & 0.891 & 0.734 & \underline{0.889} & \underline{0.732} & 0.894 & 0.734 & 1.027 & 0.769 & 0.882 & \textbf{0.729} & 0.902 & 0.737 & 1.024 & 0.767 & 0.929 & 0.746 \\
& 480 & 0.918 & 0.743 & \textbf{0.906} & \textbf{0.740} & 0.918 & \underline{0.741} & 0.967 & 0.764 & 1.097 & 0.801 & \underline{0.907} & \underline{0.741} & 0.913 & 0.743 & 1.087 & 0.797 & 0.924 & 0.747 \\
& 720 & 0.916 & 0.748 & \underline{0.908} & 0.746 & \underline{0.908} & \underline{0.745} & 0.928 & 0.753 & 1.218 & 0.853 & 0.912 & 0.746 & 0.922 & 0.750 & 1.202 & 0.848 & \textbf{0.907} & \textbf{0.744} \\
& Avg & 0.905 & 0.739 & 0.904 & 0.738 & \underline{0.896} & 0.734 & 0.912 & 0.742 & 1.031 & 0.768 & 0.896 & \underline{0.733} & 0.908 & 0.741 & 1.023 & 0.765 & \textbf{0.891} & \textbf{0.730}\\

\midrule
\multirow{9}{*}{\rotatebox{90}{BTH}} 
& 96  & 0.726 & 0.590 & 0.722 & 0.588 & 0.735 & 0.594 & \underline{0.721} & 0.588 & 0.766 & 0.588 & 0.740 & 0.592 & 0.737 & 0.597 & 0.754 & \underline{0.586} & \textbf{0.714} & \textbf{0.585} \\
& 120 & \underline{0.709} & 0.584 & 0.730 & 0.589 & 0.723 & 0.587 & 0.719 & 0.586 & 0.782 & 0.599 & 0.712 & \underline{0.583} & 0.737 & 0.596 & 0.775 & 0.598 & \textbf{0.704} & \textbf{0.581} \\
& 156 & 0.725 & 0.586 & 0.728 & 0.587 & 0.725 & 0.586 & 0.714 & \underline{0.584} & 0.798 & 0.610 & \underline{0.711} & 0.591 & 0.737 & 0.597 & 0.782 & 0.603 & \textbf{0.697} & \textbf{0.580} \\
& 192 & 0.727 & \underline{0.586} & \underline{0.727} & 0.586 & 0.730 & 0.587 & 0.732 & 0.588 & 0.817 & 0.621 & 0.727 & \underline{0.586} & 0.740 & 0.594 & 0.803 & 0.615 & \textbf{0.726} & \textbf{0.585} \\
& 264 & 0.738 & 0.590 & \textbf{0.728} & \textbf{0.581} & 0.736 & 0.597 & 0.738 & 0.592 & 0.859 & 0.645 & 0.747 & 0.595 & 0.737 & 0.592 & 0.851 & 0.642 & \underline{0.735} & \underline{0.589} \\
& 336 & 0.746 & 0.598 & 0.747 & 0.597 & \textbf{0.741} & \textbf{0.592} & 0.748 & 0.594 & 0.893 & 0.667 & \underline{0.744} & 0.598 & 0.752 & 0.601 & 0.876 & 0.658 & 0.754 & \underline{0.596} \\
& 480 & 0.837 & 0.663 & 0.780 & 0.608 & 0.786 & 0.607 & \underline{0.778} & \underline{0.607} & 0.989 & 0.714 & 0.798 & 0.602 & 0.776 & 0.611 & 0.978 & 0.709 & \textbf{0.771} & \textbf{0.606} \\
& 720 & \underline{0.826} & \underline{0.629} & 0.830 & 0.630 & 0.837 & 0.634 & 0.839 & 0.634 & 1.135 & 0.779 & 0.842 & 0.637 & 0.828 & 0.633 & 1.058 & 0.740 & \textbf{0.825} & \textbf{0.628} \\
& Avg & 0.754 & 0.603 & 0.749 & \underline{0.595} & 0.749 & 0.596 & \underline{0.748} & 0.597 & 0.880 & 0.653 & \underline{0.748} & 0.598 & 0.755 & 0.603 & 0.860 & 0.644 & \textbf{0.740} & \textbf{0.593}\\
\midrule

\multirow{7}{*}{\rotatebox{90}{Ala}} 
& 96  & \underline{0.898} & 0.568 & 0.906 & \underline{0.564} & 1.129 & 0.627 & 0.938 & 0.586 & 1.362 & 0.695 & 1.544 & 0.936 & 1.525 & 0.926 & 1.371 & 0.718 & \textbf{0.886} & \textbf{0.556} \\
& 120 & 0.981 & 0.604 & 0.978 & 0.604 & 0.946 & 0.591 & \textbf{0.772} & \textbf{0.538} & 1.387 & 0.703 & 1.516 & 0.925 & 1.531 & 0.929 & 1.371 & 0.710 & \underline{0.911} & \underline{0.574} \\
& 156 & 1.030 & \underline{0.625} & \underline{0.996} & 0.673 & 1.098 & 0.644 & 1.383 & 0.719 & 1.312 & 0.693 & 1.533 & 0.932 & 1.539 & 0.930 & 1.406 & 0.731 & \textbf{0.987} & \textbf{0.607} \\
& 192 & \underline{0.927} & \underline{0.593} & 0.945 & 0.605 & 1.187 & 0.655 & 1.164 & 0.663 & 1.404 & 0.716 & 1.565 & 0.945 & 1.552 & 0.937 & 1.424 & 0.737 & \textbf{0.925} & \textbf{0.589} \\
& 264 & 1.544 & 0.779 & 1.558 & 0.768 & 4.290 & 0.986 & 1.493 & 0.759 & \underline{1.454} & \underline{0.738} & 1.532 & 0.940 & 1.520 & 0.931 & 1.451 & 0.758 & \textbf{1.032} & \textbf{0.639} \\
& 336 & 1.078 & 0.652 & 1.168 & 0.673 & 1.132 & 0.658 & \underline{1.070} & \underline{0.633} & 1.354 & 0.722 & 1.532 & 0.948 & 1.505 & 0.933 & 1.444 & 0.764 & \textbf{0.976} & \textbf{0.632} \\
& Avg & 1.076 & 0.637 & \underline{1.074} & \underline{0.631} & 1.630 & 0.694 & 1.137 & 0.646 & 1.379 & 0.711 & 1.537 & 0.938 & 1.529 & 0.931 & 1.411 & 0.736 & 
\textbf{0.953} & \textbf{0.600}\\

\bottomrule
\end{tabular}
\label{multimodallarge}
\end{table*}

\begin{comment}
\subsection{Computational Cost}
Table \ref{computing} shows the computational cost of all compared models.

\begin{table*}[t!]
\centering
\small
\setlength{\tabcolsep}{2.6pt}
\renewcommand{\arraystretch}{1.3}
\caption{Comparison of model parameters (Par) and memory consumption (MC) on each dataset.}
\begin{tabular}{c|cc|cc|cc|cc|cc|cc|cc|cc|cc}
\toprule
\multicolumn{1}{c|}{Datasets} 
& \multicolumn{2}{c}{TimeKAN} 
& \multicolumn{2}{c}{FilterTS} 
& \multicolumn{2}{c}{TimePFN} 
& \multicolumn{2}{c}{MSGNet} 
& \multicolumn{2}{c}{TimeMixer} 
& \multicolumn{2}{c}{iTransformer} 
& \multicolumn{2}{c}{TimesNet} 
& \multicolumn{2}{c}{FEDformer} 
& \multicolumn{2}{c}{XFMNet} \\
\cmidrule(lr){2-3}
\cmidrule(lr){4-5}
\cmidrule(lr){6-7}
\cmidrule(lr){8-9}
\cmidrule(lr){10-11}
\cmidrule(lr){12-13}
\cmidrule(lr){14-15}
\cmidrule(lr){16-17}
\cmidrule(lr){18-19}
Metrics & Par & MC & Par & MC & Par & MC & Par & MC & Par & MC & Par & MC & Par & MC & Par & MC & Par & MC \\
\midrule
BJ  & xxx & xxx & xxx & xxx & xxx & xxx & xxx & xxx & xxx & xxx & xxx & xxx & xxx & xxx & xxx & xxx & xxx & xxx \\
BTH & xxx & xxx & xxx & xxx & xxx & xxx & xxx & xxx & xxx & xxx & xxx & xxx & xxx & xxx & xxx & xxx & xxx & xxx \\
Ala & xxx & xxx & xxx & xxx & xxx & xxx & xxx & xxx & xxx & xxx & xxx & xxx & xxx & xxx & xxx & xxx & xxx & xxx \\
\bottomrule
\end{tabular}
\label{computing}
\end{table*}
\end{comment}

\subsection{Effectiveness of \texttt{XGateFusion}} %与别的方法比较 三个数据集都画融合图
%Fig.~\ref{aba_mae} presents the mean MAE results of multiple model variants. Removing the recursive fusion module (w/o-RF) leads to noticeable performance drops, particularly on the Ala and BTH datasets, where complex non-stationary dynamics are more prominent. This highlights the importance of iterative refinement in capturing evolving spatiotemporal signals. More critically, replacing \texttt{XGateFusion} with a simple MLP (re-XGF-MLP) results in the most substantial degradation across all datasets. These results underscore the necessity of a learnable, modality-aware fusion strategy for effective cross-modal integration. The second worst performance is observed when both \texttt{XGateFusion} and LocTrend are replaced (re-MLP-MA), confirming the synergy between adaptive fusion and signal decomposition. The worst performance is entirely removing \texttt{XGateFusion}, demonstrating its importance in integrating visual cues.

Fig.~\ref{aba_mae} reports the mean MAE performance for a series of ablation variants, providing insights into the contribution of each module within \texttt{XFMNet}. Removing the recursive fusion component (w/o-RF) causes clear performance drops, particularly on the Ala and BTH datasets, where nonstationary and site-specific dynamics are more complex. This result underscores the importance of recursive refinement, which enables the model to capture evolving spatiotemporal dependencies across multiple fusion rounds, rather than relying on a single-step integration. Even more critical is the role of the proposed \texttt{XGateFusion}. Substituting it with a simple MLP-based fusion (re-XGF-MLP) leads to the largest performance degradation across all datasets. In addition, the comparative experiments in replacing \texttt{XGateFusion} with different fusion strategies also confirm that progressive fusion is crucial for effectively aligning heterogeneous features. A large performance gap is observed when both the decomposition module and the fusion strategy are replaced (re-MLP-MA), emphasizing the synergy between adaptive trend decomposition and cross-modal fusion. The worst-case scenario occurs when \texttt{XGateFusion} is entirely removed (w/o-XGF), demonstrating that robust visual–temporal integration is indispensable for achieving reliable water quality prediction.

To gain deeper insights into how \texttt{XGateFusion} contributes to effective cross-modal integration, we visualize the internal feature evolution at three representative fusion stages on the BTH dataset, as illustrated in Fig. \ref{fusionfinBTH}. Specifically, we track: (1) the output of the initial cross-attention operation ($A_{\mathrm{t} \leftrightarrow \mathrm{i}}$), (2) the result after gated fusion ($S_{\mathrm{f}}^{(l)}$), and (3) the final recursive representation ($\hat{Z}^{(l,n)}$). 

The top rows of each figure display channel-wise Pearson correlation matrices, which reveal how modality interactions evolve across stages. At the early stage ($A_{\mathrm{t} \leftrightarrow \mathrm{i}}$), the features exhibit high redundancy and modality-specific entanglement, reflected in dense off-diagonal correlation patterns. This indicates that the features still carry mixed modality information and lack distinct semantic separation. After passing through the gating mechanism ($S_{\mathrm{f}}^{(l)}$), the correlations become sparser and more structured, suggesting that irrelevant cross-modal noise has been suppressed and salient modality-specific cues are selectively emphasized. At the final recursive stage ($\hat{Z}^{(l,n)}$), well-organized block structures emerge, indicating that the model has successfully learned hierarchically structured, modality-enhanced representations. The bottom rows present the corresponding local activation heatmaps for a representative input. Initially, activations in $A_{\mathrm{t} \leftrightarrow \mathrm{i}}$ are scattered and spatially diffuse, reflecting the model’s early-stage uncertainty and lack of semantic focus. After gated fusion, $S_{\mathrm{f}}^{(l)}$ demonstrates localized activation patterns, showing stronger alignment with relevant spatial regions and temporal events. In the final representation $\hat{Z}^{(l,n)}$, the activations become sharply concentrated around critical spatial–temporal regions, revealing that recursive refinement further sharpens feature selectivity and enhances semantic focus.

%These observations suggest that \texttt{XGateFusion} progressively transforms raw cross-modal inputs into decorrelated, semantically meaningful, and spatially localized representations. This channel-wise decorrelation and spatial localization, coupled with semantic filtering, are key to improving model robustness and predictive accuracy, especially in datasets with high variability and complex environmental dynamics such as BTH and Ala. In summary, \texttt{XGateFusion} plays a central role in guiding effective and adaptive cross-modal integration. Its design supports progressive signal disentanglement, semantic enhancement, and recursive refinement, which together contribute to the superior performance observed in the main experiments.

%In summary, these results confirm that \texttt{XGateFusion} is pivotal in enabling effective and adaptive cross-modal integration. By coupling cross-attention with a learnable gating mechanism, it progressively disentangles intertwined modality signals, suppresses irrelevant noise, and emphasizes salient spatial–temporal cues. Moreover, its recursive refinement design allows the fused representation to be iteratively aligned with the original inputs, ensuring that evolving dependencies are accurately captured without sacrificing core information. Together, these capabilities enhance semantic richness and structural clarity in the learned features, directly translating to the superior forecasting performance consistently observed in our main experiments.  

These observations suggest that \texttt{XGateFusion} progressively transforms raw cross-modal inputs into decorrelated and semantically meaningful representations. Through channel-wise decorrelation, it effectively suppresses redundant or conflicting interactions between modalities. The semantic filtering further enhances the discriminative quality of the fused features, allowing the model to focus on task-relevant dynamics rather than noise or background variability. This capabilities are particularly beneficial in datasets with high variability and complex environmental dynamics. In summary, \texttt{XGateFusion} serves as the core driver of adaptive cross-modal integration. Its design supports progressive signal disentanglement, semantic enhancement, and recursive refinement, enabling the construction of robust representations that generalize well across diverse forecasting scenarios. This highlights its potential as a general framework for multimodal forecasting across diverse industrial domains, including energy, transportation, healthcare, and environmental monitoring.

\begin{figure}[!ht]
\centering
\includegraphics[width=0.99\columnwidth]{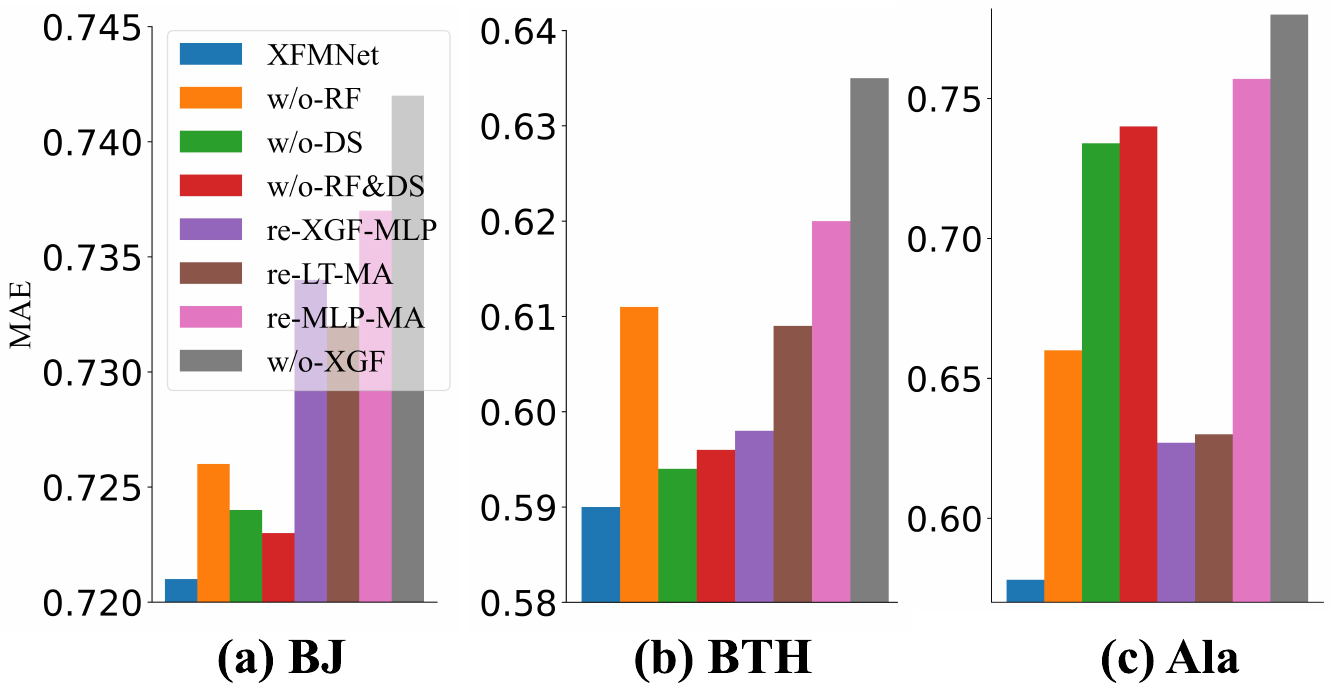} 
\caption{Ablation study on three datasets. Each bar represents the mean MAE obtained by different model variants.}
\label{aba_mae}
\end{figure}

\begin{figure}[!ht]
\centering
\includegraphics[width=0.99\columnwidth]{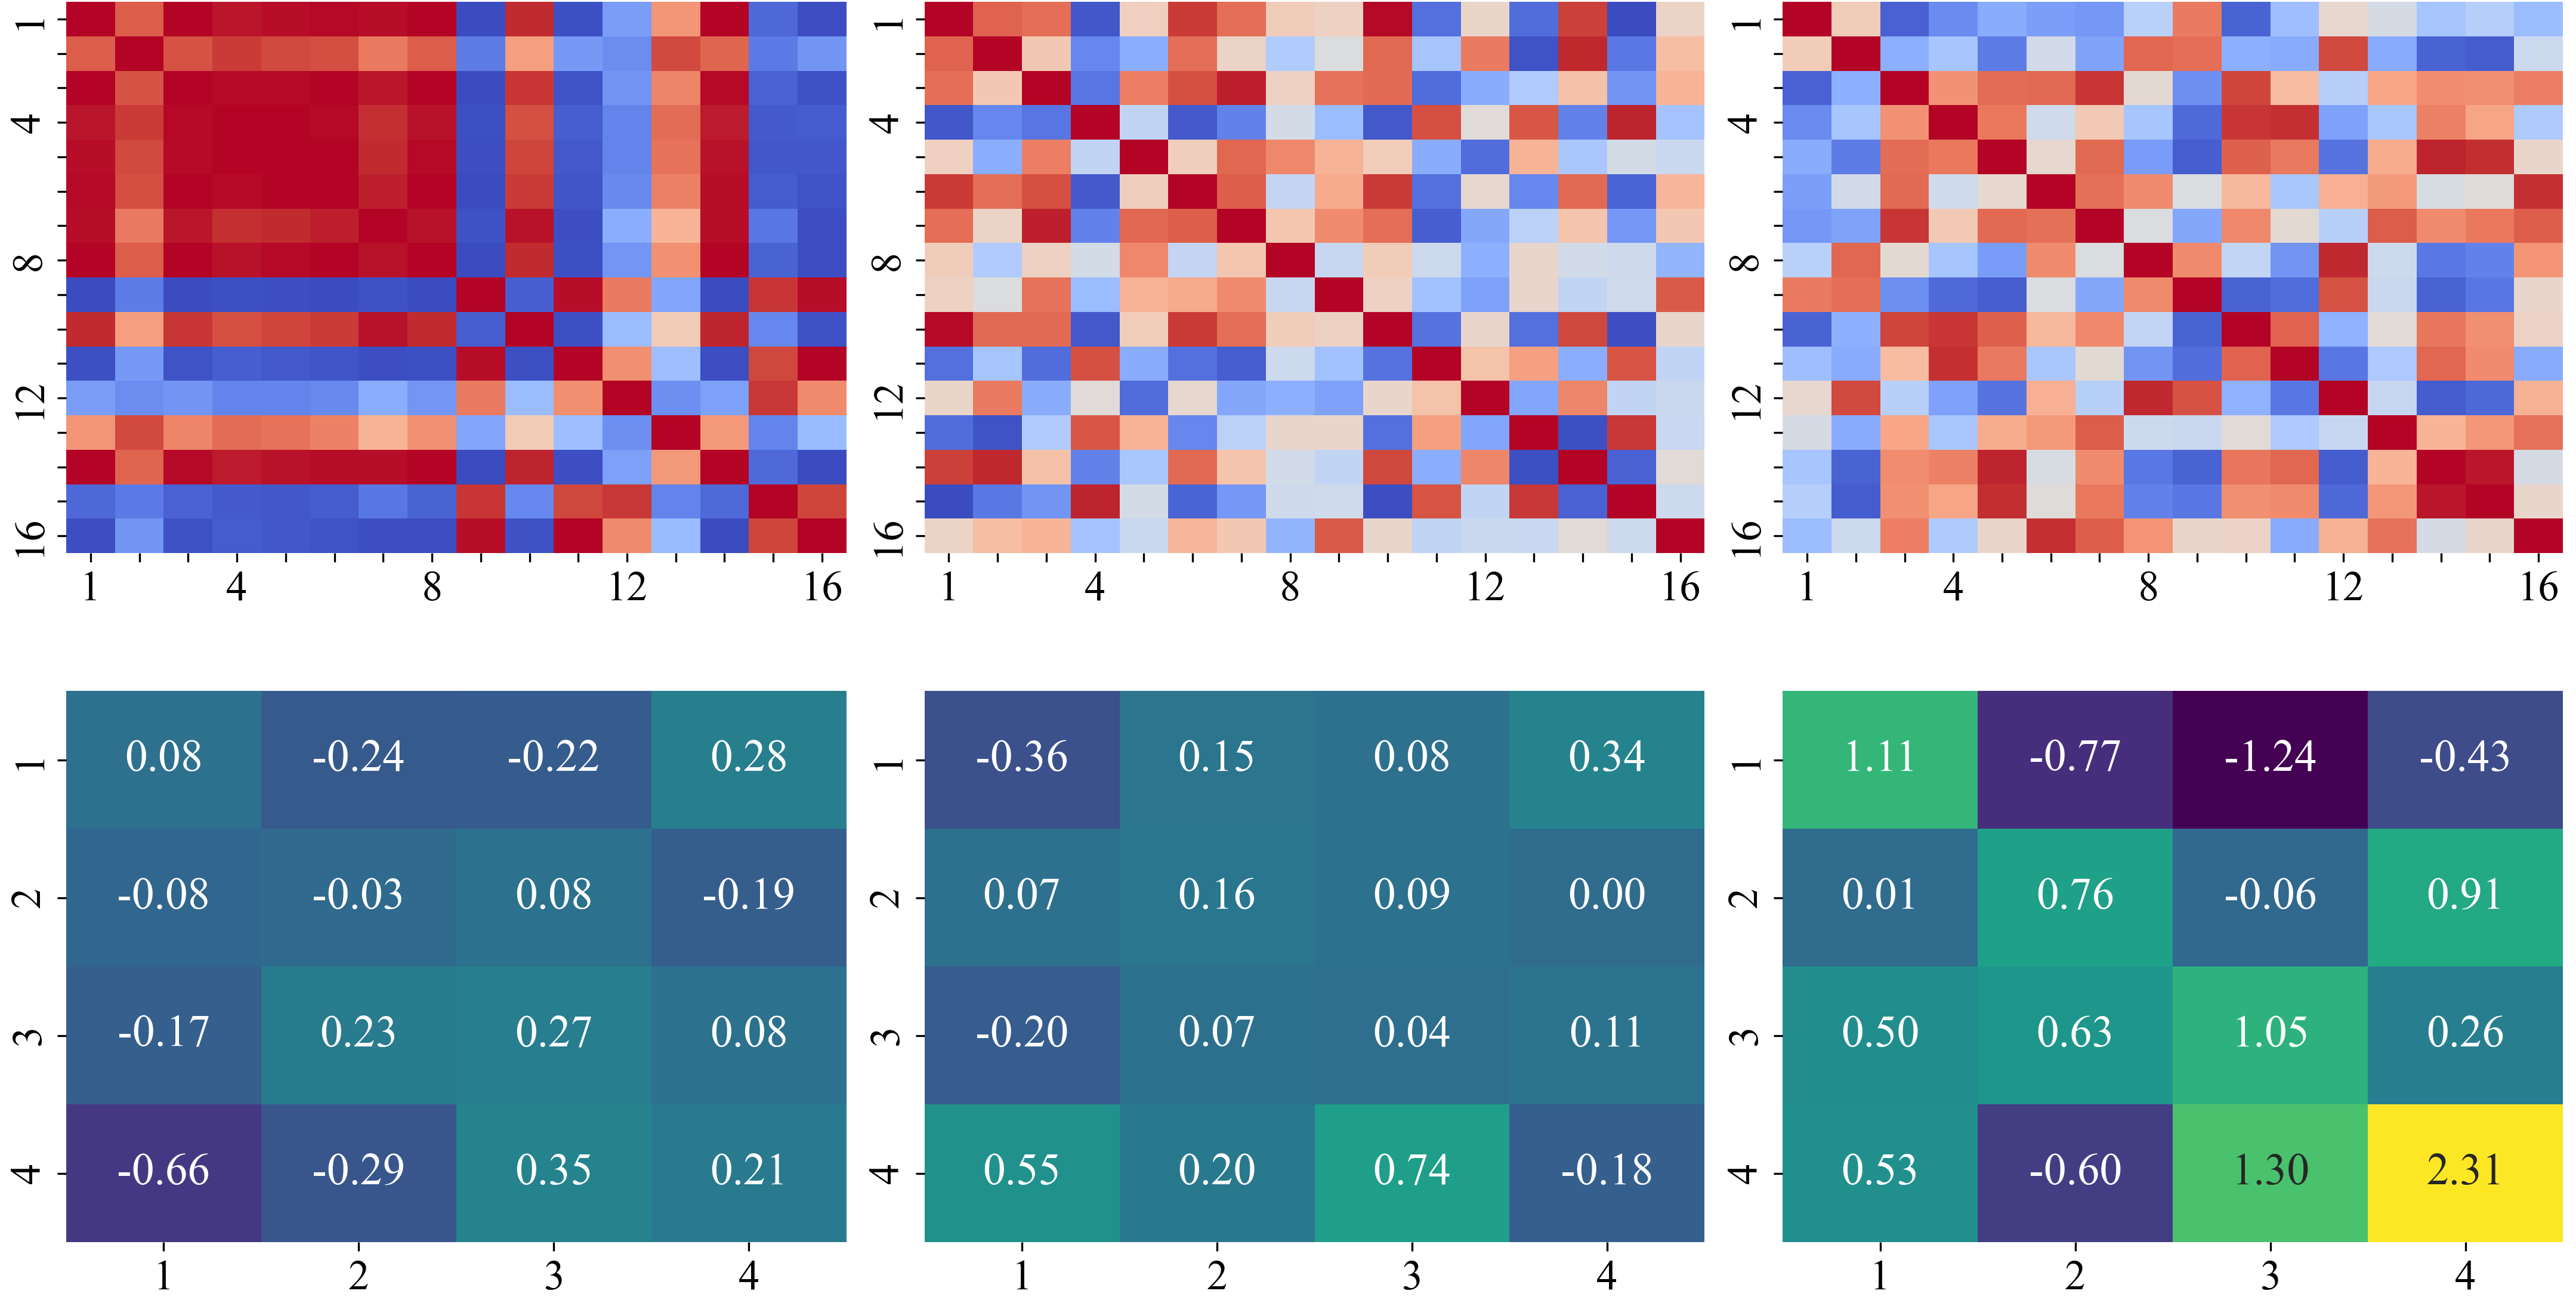} 
\caption{Feature evolution across fusion stages on BTH.} %Top: channel-wise correlation matrices show progressive decorrelation and structure emergence. Bottom: local activation maps illustrate increasing sparsity and semantic focus.}
\label{fusionfinBTH}
\end{figure}

\bigskip

\bibliographystyle{aaai}
\bibliography{ref}

\end{document}
