# Supplementary material for: Learning Intrinsic Water-Quality Dynamics with Rainfall for Data-Driven Forecasting
Source: arXiv:2508.08279 source file (2026-09-10)
Supplement: Supplementary file 2 [file Appendix.tex]

%File: formatting-instruction.tex
\documentclass[letterpaper]{article}
\usepackage{aaai}
\usepackage{amsfonts}
\usepackage{times}
\usepackage{graphicx}
\usepackage{helvet}
\usepackage{courier}
\usepackage{bibentry}
\usepackage{amsmath}
\usepackage{booktabs} 
\usepackage{multirow}
\usepackage{comment}
\usepackage{subfigure}
\usepackage{algorithm}
\usepackage{algorithmic}
\frenchspacing
\setlength{\pdfpagewidth}{8.5in}
\setlength{\pdfpageheight}{11in}
\pdfinfo{
/Title (XXX) %Multidimensional
/Author (Put All Your Authors Here, Separated by Commas)}
\setcounter{secnumdepth}{0}  
 \begin{document}
% The file aaai.sty is the style file for AAAI Press 
% proceedings, working notes, and technical reports.
%
\nocopyright
\title{Supplementary Material for Spatially Distributed Long-Term Time Series Prediction via Multimodal Multi-Scale Sequence Decomposition}
% \author{AAAI Press\\
% Association for the Advancement of Artificial Intelligence\\
% 2275 East Bayshore Road, Suite 160\\
% Palo Alto, California 94303\\
% }
\author{Anonymous submission}
\maketitle

This document provides more analysis, implementation details and
additional experimental results for comparative studies.

\section{Data Analysis}
\subsection{Cross-site Periodic Coupling Analysis} %换成一天一画 线细一点，两个图差异大一点
This section gives a detailed analysis on observed water quality data. We first compute periodograms at one-day resolution over the range of 0 to 30 days for two monitoring stations. It is shown in Fig. \ref{period} that each spectrum is displayed as a power versus period bar chart and overlaid with a LOESS \cite{loess} trend line. Station A exhibits two dominant peaks at one day and around thirty days, indicating highly pure diurnal and monthly oscillations. Station B also shows a strong one-day peak but displays additional, lower-amplitude peaks throughout the 10 to 20 day range, revealing substantial mid-term periodic variability. These pronounced differences in peak magnitude and spectral complexity provide clear evidence of heterogeneous cross-site coupling. Station A’s spectrum peaks sharply at one day and again around thirty days, yielding a clean diurnal and monthly signature with minimal intermediate bumps. Station B also shows a clear one-day rhythm but differs markedly in the ten–twenty-day band, where it displays a series of lower-amplitude peaks that are absent or much weaker in Station A’s profile. This contrast in mid-term periodic content underscores the heterogeneous nature of cross-site coupling and indicates that Station B incorporates more multi-day variability, whereas Station A remains dominated by pure daily and monthly cycles.

We further extract the full time series from both stations, applying two fourth-order Butterworth band-pass filters: one isolating the 0.8–1.2 cycles/day band (daily cycle) and the other isolating the 1/20–1/10 cycles/day band (10–20 day mid-term cycle). Each filtered signal is transformed via the Hilbert analytic signal to compute its instantaneous amplitude envelope. Finally, we plot both envelopes on a common time-index axis at high resolution, using distinct line widths and the colors to differentiate stations. In the daily-cycle envelope plot, two curves overlap perfectly, indicating that the two stations share the same diurnal frequency and exhibit similar phase behavior. In contrast, the 10–20 day envelope reveals pronounced differences. This contrast demonstrates that while daily oscillations are regionally homogeneous, the multiday component varies significantly between sites, providing compelling evidence that cross-site periodic coupling is characterized by strong diurnal synchrony alongside heterogeneous mid-term variability.

\begin{figure}[ht!]
\centering
\includegraphics[width=0.99\columnwidth]{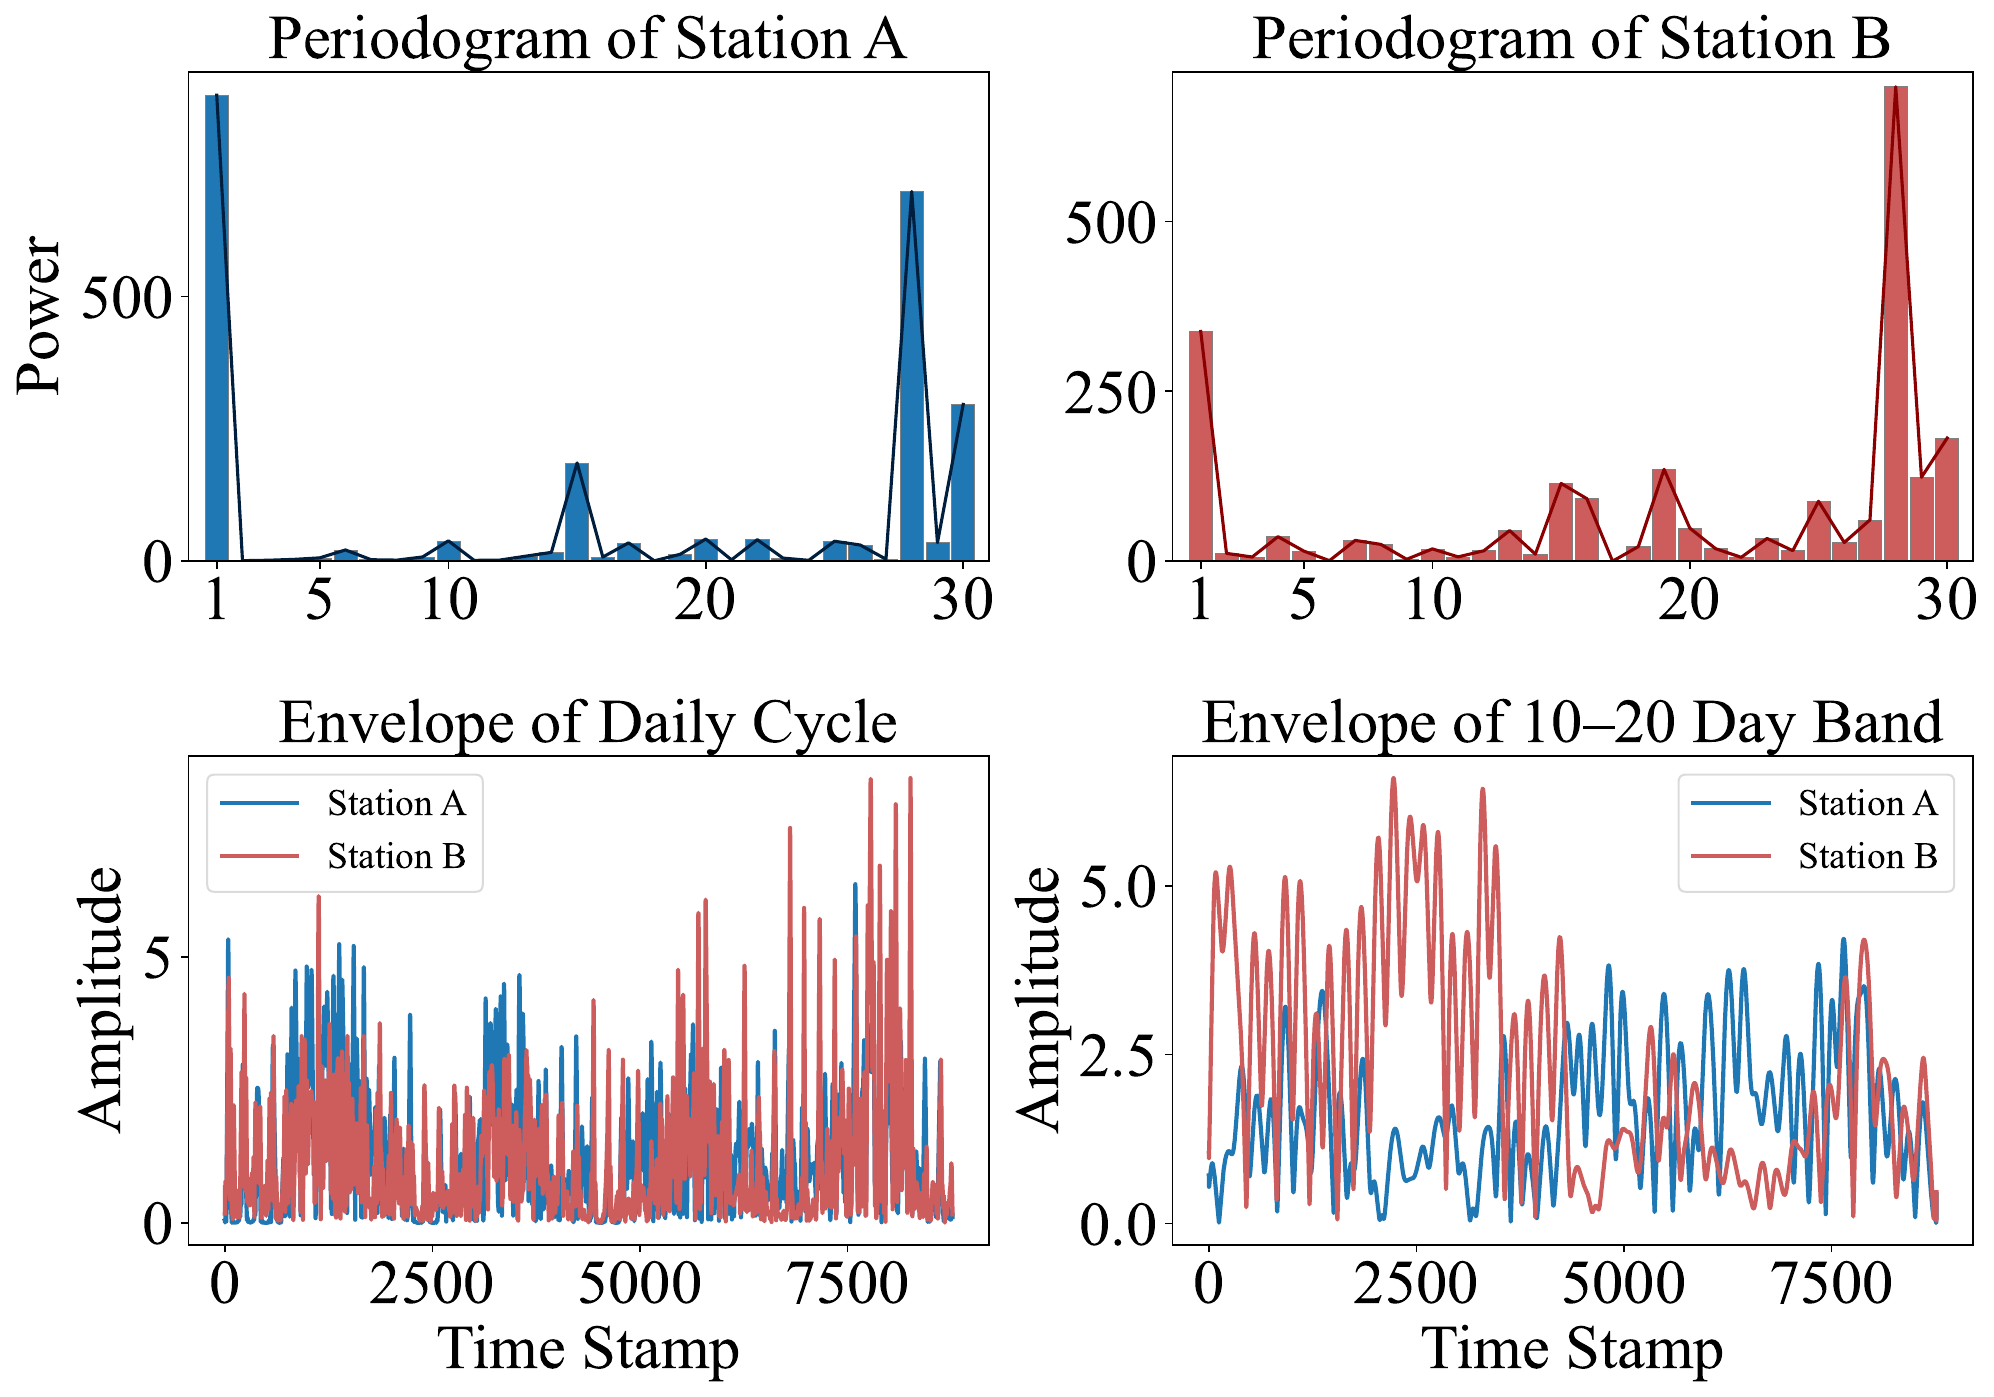} % Reduce the figure size so that it is slightly narrower than the column. Don't use precise values for figure width.This setup will avoid overfull boxes.
\caption{Two-site periodicity analysis.}
\label{period}
\end{figure}

\subsection{Stationary and Fluctuation Analysis}
\label{111111}
Fig. \ref{station} characterizes long-range dependence and time-varying volatility with environmental factors. First, autocorrelation function (ACF) plots are generated for lags 1-25 with 95\% confidence bounds, allowing quantification of memory effects: a rapid decay implies predominantly short-range dependence, whereas a slow decay reveals significant long-term trend or periodic components. Second, a fixed 48-point rolling window is applied to compute the local standard deviation at each time step, and the distribution of these rolling standard deviations is presented as a histogram. Points that exceed $\pm 3$ rolling standard deviations from the local mean are counted as anomalies. This dual-axis layout simultaneously conveys the baseline fluctuation distribution and the frequency of extreme deviations across different volatility regimes.

\begin{figure}[ht!]
\centering
\includegraphics[width=0.99\columnwidth]{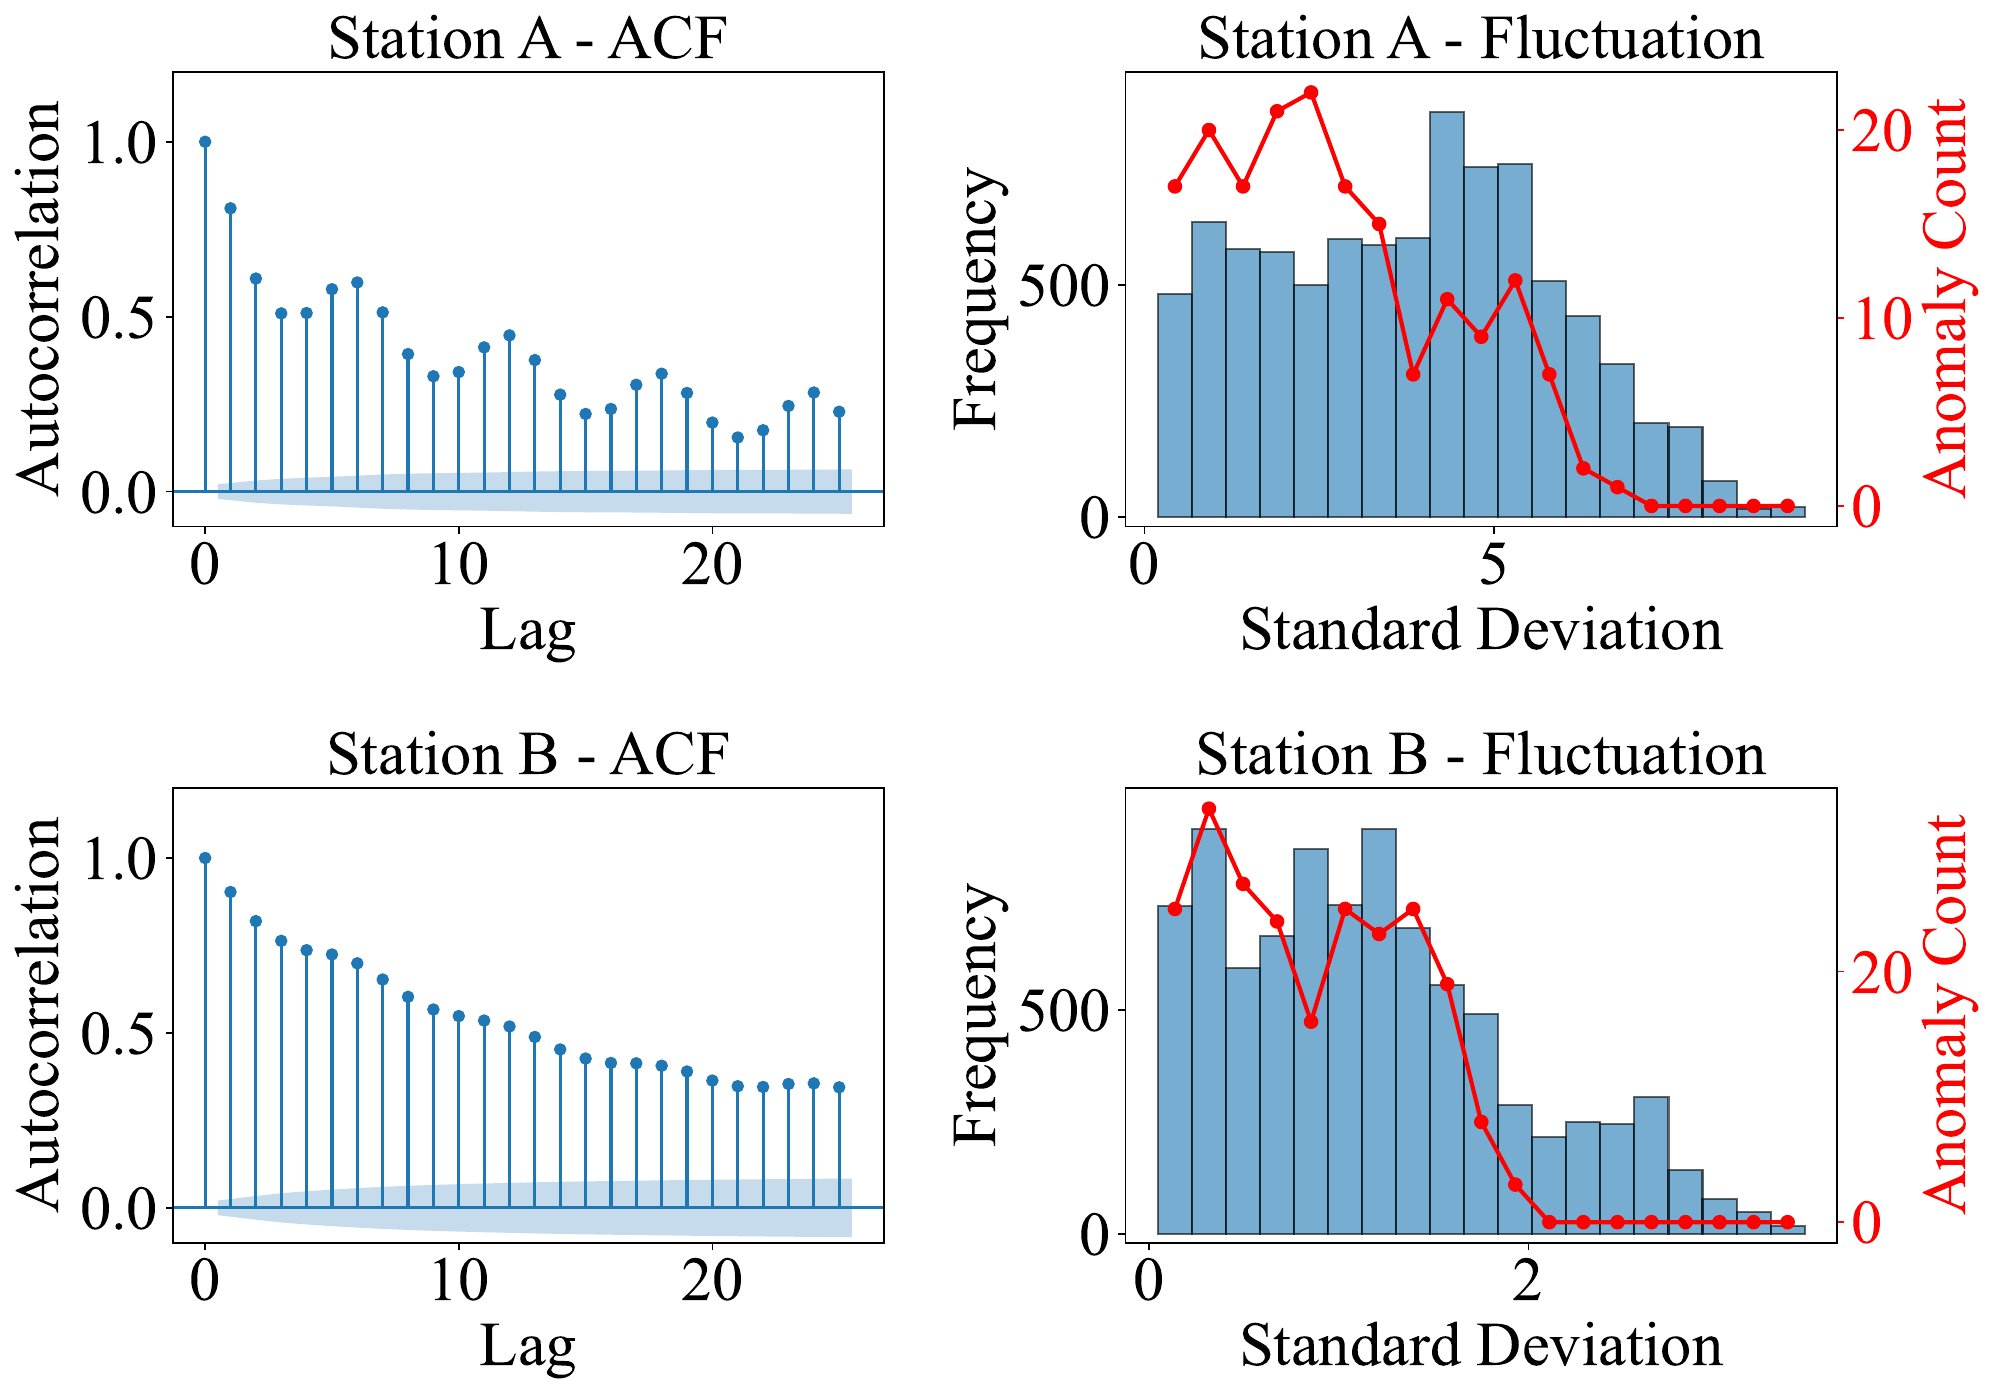} 
\caption{Two-site stationary analysis.}
\label{station}
\end{figure}

Station A’s ACF declines from approximately one at lag one to around 0.5 by lag five and remains near 0.2–0.3 through lag 25, indicating moderate mid-term dependence but relatively mild long-term drift. Its rolling standard deviation is concentrated in moderate volatility bins, with anomaly counts peaking in the standard deviation range of approximately 1-3, showing that fluctuations occur primarily during episodes of elevated local volatility. In contrast, Station B exhibits a markedly slower ACF decay, retaining positive correlation above 0.3 even at lag 25, signifying pronounced long-memory effects. Its rolling standard deviation distribution is broader with a heavy right tail, and anomalies appear both at low and mid volatility levels, reflecting both pronounced trend- or cycle-driven disturbances.

\section{Implementation Details}

\subsection{Embedding Construction}
To obtain temporally enriched representations from both modalities, we employ a unified embedding strategy consisting of value, positional, and periodic components.

For the water quality sequence at resolution level $l$, each time step $t$ contains an input $\mathbf{x}_t^{(l)} {\in} \mathbb{R}^{M}$. This is projected into a latent space using a multi-layer perceptron:
\begin{equation}
\mathbf{e}_{t}^{\text{val}} = \mathrm{MLP}(\mathbf{x}_t^{(l)}) \in \mathbb{R}^d.
\end{equation}
The MLP contains $L$ linear layers with ReLU activation and dropout, and the final layer projects to dimension $d$, transforming low-dimensional inputs into expressive representations. To encode temporal position, we add fixed sinusoidal positional embeddings:
\begin{equation}
\mathbf{e}_{t}^{\text{pos}} = \mathrm{PE}[t] \in \mathbb{R}^d,
\end{equation}
where $\mathrm{PE}[t]$ is the $t$-th row of a deterministic positional encoding matrix. We further incorporate learnable periodic embeddings based on discrete time attributes:
\begin{equation}
\mathbf{e}_{t}^{\text{per}} = \mathrm{TE}_\text{h}(h_t) + \mathrm{TE}_\text{w}(w_t) + \mathrm{TE}_\text{m}(m_t) \in \mathbb{R}^d,
\end{equation}
where $h_t$, $w_t$, and $m_t$ represent the hour of day, weekday, and month of time step $t$, respectively, and each $\mathrm{TE}_*$ is a trainable embedding lookup table. The final temporal embedding sequence is the element-wise sum:
\begin{equation}
F_{\text{temp}}^{(l)} = [\mathbf{e}_t^{\text{val}} + \mathbf{e}_t^{\text{pos}} + \mathbf{e}_t^{\text{per}}]_{t=1}^{T_l} \in \mathbb{R}^{T_l \times d}.
\end{equation}

For the image stream, the input at level $l$ is denoted by $\tilde{F}_{\text{img}}^{(l)} = [\tilde{\mathbf{f}}_1^{(l)}, \dots, \tilde{\mathbf{f}}_{T_l}^{(l)}] \in \mathbb{R}^{T_l \times d}$, where each $\tilde{\mathbf{f}}_t^{(l)}$ is the flattened and projected feature of the $t$-th downsampled image. To model temporal dependencies between frames, we apply a graph attention network for value embedding:
\begin{equation}
\overline{\mathbf{e}}_{t}^{\text{val}} = \mathrm{GAT}(\tilde{F}_{\text{img}}^{(l)})\in \mathbb{R}^d.
\end{equation}
Positional and periodic embeddings are added in the same way as sensor data:
\begin{equation}
F_{\text{img}}^{(l)} = [\overline{\mathbf{e}}_t^{\text{val}} + \overline{\mathbf{e}}_t^{\text{pos}} + \overline{\mathbf{e}}_t^{\text{per}}]_{t=1}^{T_l} \in \mathbb{R}^{T_l \times d}.
\end{equation}

This embedding process enables the model to simultaneously encode modality-specific content, temporal order, and periodicity, ensuring aligned and informative inputs for downstream fusion and modeling.

\subsection{Construction of \texttt{XFMNet}}
Algorithm 1 shows the working process of the \texttt{XFMNet}.

\begin{algorithm}[!ht]
\renewcommand\arraystretch{{2}}
\caption{{Training process of \texttt{XFMNet}}}
\label{train}
\small
{\bf Input:} Sensor time series ($X$), Remote sensing-based precipitation imagery sequence ($I$)\\
{\bf Output:} Prediction result $\hat{Y}$ 
\begin{algorithmic}[1]%{\Statex}
\FOR{each epoch}
\STATE \textit{Preprocessing and Multiscale Aligned Sampling}
\STATE Downsampling $X$ by fixed-stride 1D pooling to obtain $X^{(l)}$.
\STATE Embedding $X^{(l)}$ to obtain $F_{\text{temp}}^{(l)}$
\STATE Extracting features from $I$ by EfficientNet, obtaining $F_{\text{raw}}$.
\STATE Downsampling and projecting $F_{\text{raw}}$ to obtain $\tilde{F}_{\text{img}}^{(l)}$.
\STATE Embedding $\tilde{F}_{\text{img}}^{(l)}$ to obtain $F_{\text{img}}^{(l)}$
\STATE Concatenating $F_{\text{img}}^{(l)}$ and $F_{\text{temp}}^{(l)}$ and fusing by a 2D convolution to obtain $F^{(l)}_{con}$.
\STATE \textit{Sequence Decomposition and Multimodal Fusion}
\STATE Decomposing $F_{\mathrm{mod}}^{(l)} {\in}[F_{\mathrm{temp}}^{(l)}, F_{\mathrm{img}}^{(l)}, F^{(l)}_{con}]$ by \texttt{LocTrend} into seasonal part ${S_{\text{mod}}^{(l)}}$ and trend part ${R_{\text{mod}}^{(l)}}$.
\STATE Enhancing ${S_{\text{mod}}^{(l)}}$ in bottom-up direction by stacked linear layers and a multi-kernel convolutional block.
\STATE Enhancing ${R_{\text{mod}}^{(l)}}$ in top-down direction by transposed convolution block and stacked linear layers.
\STATE Taking seasonal part as an example, performing the first fusion by bidirectional interaction to obtain $A_{t\leftarrow i}^{(l)}$ and $A_{i\leftarrow t}^{(l)}$.
\STATE Performing the second fusion by interpolated fusion to obtain $\hat{S}_{\mathrm{temp}}^{(l)}$ and $\hat{S}_{\mathrm{img}}^{(l)}$.
\STATE Performing the third fusion by gated fusion to obtain $S_{\mathrm{f}}^{(l)}$.
\STATE Performing the fourth fusion by adding the early fusion $S_{\mathrm{con}}^{(l)}$ to obtain $\bar{S}^{(l)}$.
\STATE Performing the fifth fusion by adaptively integrating seasonal part $\bar{S}^{(l)}$ and trend part $\bar{R}^{(l)}$ to obtain $Z^{(l)}$.
\STATE Passing a shared feed-forward block to obtain $\hat{Z}^{(l)}$.
\STATE Performing recursive fusion to obtain $\hat{Z}^{(l,n)}$
\STATE \textit{Long-term Cross-site Prediction}
\STATE Performing scale-specific regression to obtain $Y_{\text{reg}}^{(l)}$
\STATE Projecting and averaging all scales to obtain the final prediction $\hat{Y}$.
\ENDFOR
\end{algorithmic}
\end{algorithm}

\subsection{Parameter Sensitivity} %表格
The predictive performance of \texttt{XFMNet} depends on several essential hyperparameters, including the number of recursive fusion iterations ($n$), the depth of downsampling levels ($l$), the embedding size ($d$), the dimensionality of the feedforward network ($d_f$), and the order of multi-scale information enhancement. These settings are selected through systematic experimentation to achieve optimal results. Table~\ref{tab:recursive_fusion} presents the performance under different numbers of recursive fusion iterations ($n$). Compared to $n=1$, introducing an additional fusion step ($n=2$) consistently reduces both MSE and MAE across all datasets, demonstrating that moderate recursive refinement effectively mitigates the information loss from one-shot fusion. However, further increasing $n$ beyond 2 results in clear performance degradation, because repeated fusion introduces redundant representations and excessive aggregation of similar signals, ultimately diminishing generalization. Based on these observations, $n=2$ is selected as the optimal configuration, striking the best balance between information retention and model simplicity.

\begin{table*}[ht]
\centering
\caption{Effect of recursive fusion iterations ($n$) on forecasting accuracy.} %Optimal performance is observed at $n=2$.}
\begin{tabular}{c|cc|cc|cc|cc|cc}
\toprule
\multirow{2}{*}{Dataset} & \multicolumn{2}{|c|}{$n=1$} & \multicolumn{2}{c|}{$n=2$} & \multicolumn{2}{c|}{$n=3$} & \multicolumn{2}{c|}{$n=4$} & \multicolumn{2}{c}{$n=5$} \\
\cmidrule(lr){2-3}\cmidrule(lr){4-5}\cmidrule(lr){6-7}\cmidrule(lr){8-9}\cmidrule(lr){10-11}
& MSE & MAE & MSE & MAE & MSE & MAE & MSE & MAE & MSE & MAE \\
\midrule
BJ & 0.877 & 0.726 & 0.867 & 0.721 & 0.879 & 0.726 & 0.893 & 0.734 & 0.881 & 0.728 \\
BTH     & 0.781 & 0.611 & 0.726 & 0.585 & 0.726 & 0.585 & 0.728 & 0.586 & 0.726 & 0.585 \\
Ala & 1.148 & 0.660 & 0.854 & 0.578 & 1.415 & 0.716 & 2.256 & 0.823 & 1.092 & 0.626 \\
\bottomrule
\end{tabular}
\label{tab:recursive_fusion}
\end{table*}

Table~\ref{tab:downsampling_levels} shows the forecasting performance under different numbers of downsampling levels ($l$). The results reveal that introducing a moderate degree of multiscale downsampling substantially improves predictive accuracy compared to no downsampling ($l=0$). Specifically, setting $l=3$ consistently achieves the lowest MSE and MAE on all datasets, highlighting its effectiveness in capturing salient temporal patterns while reducing redundancy. However, further increasing $l$ to 4 degrades performance, because excessive resolution reduction discards fine-grained temporal signals critical for modeling localized dynamics. These results suggest that a balanced downsampling configuration is essential for maximizing the benefits of multiscale feature extraction.

\begin{table*}[t]
\centering
\caption{Forecasting performance with varying numbers of downsampling levels ($l$).}
\begin{tabular}{c|cc|cc|cc|cc|cc}
\toprule
\multirow{2}{*}{Dataset} & \multicolumn{2}{c|}{$l=0$} & \multicolumn{2}{c|}{$l=1$} & \multicolumn{2}{c|}{$l=2$} & \multicolumn{2}{c|}{$l=3$} & \multicolumn{2}{c}{$l=4$} \\
\cmidrule(lr){2-3} \cmidrule(lr){4-5} \cmidrule(lr){6-7} \cmidrule(lr){8-9} \cmidrule(lr){10-11}
& MSE & MAE & MSE & MAE & MSE & MAE & MSE & MAE & MSE & MAE \\
\midrule
BJ & 0.872 & 0.724 & 0.913 & 0.742 & 0.908 & 0.740 & 0.867 & 0.721 & 0.881 & 0.727 \\
BTH     & 0.743 & 0.594 & 0.743 & 0.594 & 0.735 & 0.590 & 0.726 & 0.585 & 0.735 & 0.589 \\
Ala & 1.428 & 0.734 & 0.880 & 0.582 & 1.208 & 0.674 & 0.854 & 0.578 & 1.624 & 0.772 \\
\bottomrule
\end{tabular}
\label{tab:downsampling_levels}
\end{table*}

Table~\ref{tab:embedding_dimension} shows the impact of varying the embedding dimension $d$ on predictive performance. As $d$ increases from 8 to 16, all datasets consistently exhibit improved MSE and MAE, highlighting that richer embeddings help capture more informative temporal and spatial patterns. However, further increasing $d$ beyond 16 does not lead to consistent improvements. For example, while BTH benefits slightly when $d=32$, the Alabama dataset shows clear performance degradation, likely due to overfitting and increased model variance in smaller datasets. Overall, $d=16$ provides the most stable and competitive results across different scenarios, striking a balance between expressiveness and generalization.

\begin{table*}[htbp]
\centering
\caption{Effect of embedding dimension $d$ on forecasting performance.}
\renewcommand{\arraystretch}{1.1}
\begin{tabular}{c|cc|cc|cc|cc|cc}
\toprule
\multirow{2}{*}{Dataset} & 
\multicolumn{2}{|c|}{$d=8$} &
\multicolumn{2}{c|}{$d=16$} &
\multicolumn{2}{c|}{$d=24$} &
\multicolumn{2}{c|}{$d=32$} &
\multicolumn{2}{c}{$d=40$} \\
\cmidrule(lr){2-3}
\cmidrule(lr){4-5}
\cmidrule(lr){6-7}
\cmidrule(lr){8-9}
\cmidrule(lr){10-11}
& MSE & MAE & MSE & MAE & MSE & MAE & MSE & MAE & MSE & MAE \\
\midrule
BJ & 0.915 & 0.740 & 0.867 & 0.721 & 0.906 & 0.737 & 0.889 & 0.731 & 0.876 & 0.725 \\
BTH     & 0.735 & 0.593 & 0.726 & 0.585 & 0.720 & 0.583 & 0.709 & 0.581 & 0.717 & 0.583 \\
Ala & 0.895 & 0.591 & 0.854 & 0.578 & 1.396 & 0.623 & 1.433 & 0.736 & 0.875 & 0.587 \\
\bottomrule
\end{tabular}
\label{tab:embedding_dimension}
\end{table*}

We further examine the impact of varying the hidden dimension $d_f$ in the feedforward layers (Table~\ref{tab:ffd_dim}). The results reveal that moderate hidden sizes (e.g., $d_f=8$ or $d_f=16$) deliver more consistent performance across datasets. In particular, increasing $d_f$ beyond 24 tends to degrade MSE and MAE on Alabama, likely due to over-parameterization and limited data coverage in this region, which lead to overfitting. On Beijing and BTH, the results remain relatively stable across different hidden dimensions, suggesting that these datasets are less sensitive to the capacity of the feedforward layers. Consequently, we set $d_f=16$ to maintain a trade-off between representation capacity and robust generalization.

\begin{table*}[t]
\centering
\caption{Impact of hidden dimension $d_f$ in feedforward layers on MSE and MAE across datasets.}
\begin{tabular}{c|cc|cc|cc|cc|cc}
\toprule
\multirow{2}{*}{Dataset} & \multicolumn{2}{c|}{$d_f=8$} & \multicolumn{2}{c|}{$d_f=16$} & \multicolumn{2}{c|}{$d_f=24$} & \multicolumn{2}{c|}{$d_f=32$} & \multicolumn{2}{c}{$d_f=40$} \\
\cmidrule(lr){2-3}
\cmidrule(lr){4-5}
\cmidrule(lr){6-7}
\cmidrule(lr){8-9}
\cmidrule(lr){10-11}
 & MSE & MAE & MSE & MAE & MSE & MAE & MSE & MAE & MSE & MAE \\
\midrule
Beijing & 0.867 & 0.720 & 0.860 & 0.716 & 0.900 & 0.732 & 0.867 & 0.721 & 0.860 & 0.717 \\
BTH     & 0.707 & 0.579 & 0.725 & 0.585 & 0.719 & 0.583 & 0.726 & 0.585 & 0.712 & 0.582 \\
Alabama & 0.823 & 0.560 & 1.016 & 0.614 & 1.545 & 0.747 & 0.854 & 0.578 & 1.398 & 0.713 \\
\bottomrule
\end{tabular}
\label{tab:ffd_dim}
\end{table*}

%We set the sliding-window length $w$ to control the granularity of local temporal segments in \texttt{LocTrend}. It is shown in Table \ref{window} that a larger window size could smooth over fine-grained dynamics, while a smaller window may introduce noise in trend estimation. We find that $w = 27$ offers stable performance across datasets with different temporal characteristics. Notably, since \texttt{LocTrend} employs fixed kernel projections without parameter learning, this setting also ensures fast execution during both training and inference.

We set the sliding-window length $w$ to control the granularity of local temporal segments in \texttt{LocTrend}. As illustrated in Table~\ref{window}, the choice of $w$ balances sensitivity to short-term fluctuations and the ability to capture longer-range trends. A small window size tends to increase the influence of high-frequency variations and may introduce noise in the extracted trend components. Conversely, a huge window can over-smooth the sequence, potentially masking abrupt changes or fine-grained dynamics. We find that a moderate setting of $w = 27$ consistently yields robust performance across datasets exhibiting diverse temporal characteristics, including periodicity, abrupt transitions, and non-stationary behaviors. Furthermore, since \texttt{LocTrend} operates with fixed kernel projections and avoids costly parameter learning or matrix decomposition, this configuration ensures both computational efficiency and ease of deployment during training and inference.

\begin{table*}[htbp]
\centering
\caption{Performance of \texttt{XFMNet} under Different window size $w$}
\label{window}
\begin{tabular}{c|cc|cc|cc|cc|cc}
\toprule
\multirow{2}{*}{Dataset} & 
\multicolumn{2}{c|}{$w=9$} & 
\multicolumn{2}{c|}{$w=18$} & 
\multicolumn{2}{c|}{$w=27$} & 
\multicolumn{2}{c|}{$w=36$} & 
\multicolumn{2}{c}{$w=45$} \\
\cmidrule(r){2-3} \cmidrule(r){4-5} \cmidrule(r){6-7} \cmidrule(r){8-9} \cmidrule(r){10-11}
 & MSE & MAE & MSE & MAE & MSE & MAE & MSE & MAE & MSE & MAE \\
\midrule
BJ  & 0.868 & 0.721 & 0.867 & 0.721 & 0.867 & 0.721 & 0.867 & 0.721 & 0.867 & 0.721 \\
BTH      & 0.725 & 0.585 & 0.727 & 0.585 & 0.727 & 0.585 & 0.727 & 0.585 & 0.727 & 0.586 \\
Ala  & 0.995 & 0.628 & 0.958 & 0.620 & 0.929 & 0.609 & 0.973 & 0.621 & 0.946 & 0.613 \\
\bottomrule
\end{tabular}
\end{table*}

To further amplify decomposed components and facilitate cross-resolution representation alignment, we introduce a hierarchical dual-path enhancement mechanism. Table \ref{tab:trend-season-order} show that for the seasonal component, a bottom-up refinement achieves better performance. Given that high-frequency seasonal variations are typically rooted in local fluctuations, the model progressively aggregates fine-grained representations into coarser ones. Conversely, for the trend component, the top-down enhancement strategy achieves better performance. This design is motivated by the observation that trend dynamics often manifest over long horizons, and global structure should guide the shaping of local trends. Coarse-resolution trend signals are gradually upsampled to reconstruct higher-resolution features. Overall, this bidirectional refinement paradigm provides a principled way to separately optimize seasonality and trend components, while also aligning multi-resolution features. It strengthens both local sensitivity and global awareness, forming a key part of our architecture’s effectiveness in complex temporal environments.

\begin{table*}[htbp]
\centering
\caption{Performance under different season-trend enhancement orders.}
\label{tab:trend-season-order}
\begin{tabular}{c|cc|cc|cc|cc}
\toprule
\multirow{2}{*}{Dataset} & \multicolumn{2}{c|}{season↓-trend↑} & \multicolumn{2}{c|}{season↑-trend↑} & \multicolumn{2}{c|}{season↑-trend↓} & \multicolumn{2}{c}{season↓-trend↓} \\
\cmidrule(r){2-3} \cmidrule(r){4-5} \cmidrule(r){6-7} \cmidrule(r){8-9}
& MSE & MAE & MSE & MAE & MSE & MAE & MSE & MAE \\
\midrule
BJ & 0.867 & 0.721 & 0.868 & 0.721 & 0.867 & 0.721 & 0.864 & 0.720 \\
BTH     & 0.727 & 0.585 & 0.727 & 0.586 & 0.726 & 0.585 & 0.726 & 0.585 \\
Ala & 1.063 & 0.640 & 1.254 & 0.675 & 0.854 & 0.578 & 0.969 & 0.621 \\
\bottomrule
\end{tabular}
\end{table*}

\section{Dataset Description}
The details of the three real-world water quality datasets are provided in Table \ref{sum}. The BJ and BTH datasets cover the period from January 2019 to December 2022, with measurements recorded every four hours. The BJ dataset contains dissolved oxygen (DO) data from six monitoring stations distributed across the Chaobai River basin in the Beijing area, covering approximately 120 km. The BTH data set includes total nitrogen (TN) measurements from nine stations located throughout the broader region of three cities, within the Beiyan Canal, covering a spatial range of about 300 km. The Ala dataset comprises hourly DO observations from five stations in Alabama, collected between January 2021 and December 2022. These stations are situated within the Cahaba River watershed and span approximately 190 km. All datasets are supplemented with remote sensing-based precipitation imagery, temporally aligned with the water quality sampling frequency (four-hourly for BJ and BTH; hourly for Ala) and featuring a spatial resolution of 0.1 {$\times$} 0.1°. An example of remote sensing-based precipitation imagery is shown in Fig. \ref{rain}. It captures the spatio-temporal environmental dynamics that influence water quality. We release a publicly available multimodal water quality prediction dataset BJ to support further research in multimodal environmental forecasting. The sample data is presented in Table \ref{tab:data-sample}. %还有遥感图

\begin{table}[!ht]
\centering
\caption{Dataset Description}
\label{sum}
\begin{tabular}{cccc}
\hline
\multirow{2}{*}{Parameter} & \multicolumn{3}{c}{Datasets}  \\ \cline{2-4}
& BTH & BJ & Ala \\ \hline
Number of station   & 9  & 6       & 5       \\ \hline
% Time Span        & \multicolumn{2}{c|}{Jan. 1, 2019–Dec. 31, 2022}  & Jan. 1, 2021–Dec. 31, 2022 \\ \hline
Sampling frequency        & 4 hours & 4 hours & 1 hour \\ \hline
Data length      & 8,766   & 8,766   & 17,520   \\ \hline
Water quality indicator  & TN     & DO     & DO      \\ \hline
\end{tabular}
\end{table}

\begin{figure}[!ht]
\centering
\includegraphics[width=0.6\columnwidth]{figure/rainfall.jpg} 
\caption{Remote sensing-based precipitation imagery.}
\label{rain}
\end{figure}

%样例数据
\begin{table*}[htbp]
\centering
\caption{Example of DO Index in BJ Dataset with Station Coordinates}
\label{tab:data-sample}
\renewcommand{\arraystretch}{1.2}
\begin{tabular}{c|cccccc}
\toprule
\textbf{Station} & \textbf{Dahongqiao} & \textbf{Shawo} & \textbf{Xinbaliqiao} & \textbf{Wangjiabai} & \textbf{Wucun} & \textbf{Huairoushuiku} \\
\midrule
\textbf{Latitude}  & 40.010°N & 39.850°N & 39.920°N & 39.970°N & 39.880°N & 40.350°N \\
\textbf{Longitude} & 116.320°E & 116.240°E & 116.500°E & 116.700°E & 116.600°E & 116.630°E \\
\midrule
2019/1/1 0:00  & 11.17 Mg/L & 11.06 Mg/L & 6.39 Mg/L & 6.04 Mg/L & 10.71 Mg/L & 13.92 Mg/L\\
2019/1/1 4:00  & 11.13 Mg/L& 11.08 Mg/L& 5.68 Mg/L & 5.80 Mg/L & 10.38 Mg/L & 13.98 Mg/L\\
2019/1/1 8:00  & 11.09 Mg/L & 10.95 Mg/L & 5.91 Mg/L & 5.92 Mg/L & 10.00 Mg/L & 13.97 Mg/L \\
2019/1/1 12:00 & 11.05 Mg/L & 10.92 Mg/L& 10.11 Mg/L& 5.78 Mg/L & 9.96 Mg/L & 13.94 Mg/L\\
2019/1/1 16:00 & 11.01 Mg/L& 11.48 Mg/L& 11.99 Mg/L & 5.84 Mg/L & 10.27 Mg/L & 13.96 Mg/L\\
2019/1/1 20:00 & 10.97 Mg/L & 11.58 Mg/L & 8.45 Mg/L & 5.87 Mg/L & 10.63 Mg/L & 13.89 Mg/L \\
2019/1/2 0:00  & 10.93 Mg/L & 9.20 Mg/L  & 5.82 Mg/L & 13.16 Mg/L& 14.23 Mg/L& 14.80 Mg/L\\
2019/1/2 4:00  & 10.89 Mg/L & 9.28 Mg/L & 4.75 Mg/L & 13.08 Mg/L & 13.39 Mg/L & 14.47 Mg/L\\
2019/1/2 8:00  & 10.86 Mg/L & 9.40 Mg/L & 4.70 Mg/L & 12.62 Mg/L & 13.21 Mg/L & 14.64 Mg/L\\
2019/1/2 12:00 & 10.82 Mg/L & 10.22 Mg/L& 10.00 Mg/L& 13.27 Mg/L& 13.55 Mg/L& 14.66 Mg/L\\
\bottomrule
\end{tabular}
\end{table*}

\section{Compared Models and Evaluation Metrics}
We compare our method with several state-of-the-art time series forecasting models. TimeKAN \cite{TimeKAN} introduces a KAN-based architecture that decomposes time series into multiple frequency bands and learns multi-order representations for each. FilterTS \cite{FilterTS} employs learnable frequency-domain filters to extract salient patterns and suppress high-frequency noise. TimePFN \cite{TimePFN} leverages synthetic data priors and permutation-invariant transformers to achieve robust forecasting in few-shot and zero-shot settings. MSGNet \cite{MSGNet} models multi-scale inter-series dependencies via frequency decomposition and adaptive graph convolution. TimeMixer \cite{TimeMixer} proposes a fully MLP-based framework that integrates seasonal and trend components across multiple resolutions through parallel decomposition and multi-predictor fusion. iTransformer \cite{iTransformer} inverts the attention mechanism over variate tokens to better capture multivariate dependencies. TimesNet \cite{TimesNet} converts 1D time series into 2D period-based tensors and applies 2D convolutions to model intra- and inter-period variations. FEDformer \cite{FEDformer} combines seasonal-trend decomposition with frequency-domain modeling for efficient long-term forecasting.

MSE \cite{MSE} emphasizes large deviations and is more sensitive to abrupt fluctuations, while MAE \cite{MAE} reflects overall average error with greater robustness to outliers. Lower MSE and MAE values indicate higher forecasting accuracy and better model performance. They are calculated as:
\begin{equation}
\text{MAE}{=}\frac{1}{a} \sum_{j=1}^a\left|\hat{h}_j{-}h_j\right|
\end{equation}
\begin{equation}
\text{MSE}{=}\frac{1}{a} \sum_{j=1}^a\left|\hat{h}_j{-}h_j\right|^2
\end{equation}
where $a$ denotes the number of samples. $h_j$ and $\hat{h}_j$ denote the ground truth and predicted values of data point $j$.

\section{Full Results}
\subsection{Comparitive Results} %可以画图

Table~\ref{tab:main_results} reports the long-term forecasting performance of all baseline models and \texttt{XFMNet} across three representative real-world datasets, each evaluated under a range of prediction horizons. The corresponding trend comparisons of MSE and MAE metrics across different time steps are visualized in Figs.~\ref{BJ}–\ref{Ala}. These results demonstrate the superior modeling capacity of \texttt{XFMNet} in capturing complex spatiotemporal dynamics and maintaining stable predictive performance across diverse conditions. Compared to existing methods, \texttt{XFMNet} consistently ranks first or second in both error metrics, revealing its strong generalization capability and robustness under varying forecasting challenges.

The BJ dataset, primarily composed of water quality records from urban monitoring stations, exhibits relatively smooth temporal patterns with localized fluctuations driven by rainfall. This dataset serves as a relatively regular benchmark. As shown in both Table~\ref{tab:main_results} and Fig.~\ref{BJ}, \texttt{XFMNet} outperforms all competing models across all horizons, with particularly significant gains in MSE. Since MSE is more sensitive to large deviations, this suggests that \texttt{XFMNet} is especially effective in detecting sharp changes or localized anomalies. The model's ability to leverage visual cues offers an advantage in anticipating such events. MAE results, which reflect general accuracy, also remain consistently favorable, indicating reliable modeling of baseline trends and normal variation ranges.

The BTH dataset introduces increased modeling complexity. It covers a broad spatial region encompassing three metropolitan areas, with a dense network of monitoring sites affected by both natural hydrological processes and anthropogenic factors. The spatial heterogeneity leads to frequent inter-site correlations, phase shifts across locations, and a higher degree of non-stationarity. These characteristics typically challenge traditional models that treat series independently or rely solely on self-attention. However, \texttt{XFMNet} still demonstrates strong performance on this dataset, achieving the lowest or near-lowest MAE and lowest MSE under every time horizon, as shown in Fig.~\ref{BTH}. This suggests that its recursive cross-modal fusion enables better extraction of inter-series dependencies and dynamic relationships, particularly through its alignment mechanism that adapts at each step. Notably, its margin of superiority widens at longer horizons, indicating resilience against error accumulation during recursive inference.

The Ala dataset, representing a natural watershed system, features substantial seasonal variation driven by precipitation events, runoff cycles, and land-cover transitions. Unlike urban datasets, Ala exhibits strong periodicity and abrupt changes due to exogenous drivers. As reflected in Table~\ref{tab:main_results} and Fig.~\ref{Ala}, most baselines suffer performance degradation on this dataset, especially under long-horizon settings, due to limited ability to model such exogenous and nonlinear behaviors. In contrast, \texttt{XFMNet} maintains a consistently low error across all forecasting steps, with the lowest MSE and MAE throughout. Fig.~\ref{ladar} provides a compact visual summary of these performance comparisons across all datasets and prediction lengths. It clearly shows that \texttt{XFMNet} excels in short-term prediction (96–192 steps) and maintains reliable long-range forecasting ability beyond 480 steps, a regime where most baselines deteriorate significantly. This consistent advantage underscores the benefits of step-wise multimodal alignment and fine-grained feature interaction, particularly in modeling multi-source environmental data where spatial, temporal, and contextual information are deeply intertwined.

In summary, these comprehensive results validate the effectiveness of \texttt{XFMNet}'s core design: its ability to inject visual context at each step, progressively align modalities, and recursively refine cross-modal representations empowers it to handle diverse forecasting challenges. Whether under urban, regional, or basin-scale conditions, the model adapts well to both stationary and non-stationary dynamics, offering a promising solution for fine-grained spatiotemporal prediction tasks.

%BJ
\begin{figure}[htbp]
    \centering
    \subfigure[MSE]{%
        \includegraphics[width=0.99\columnwidth]{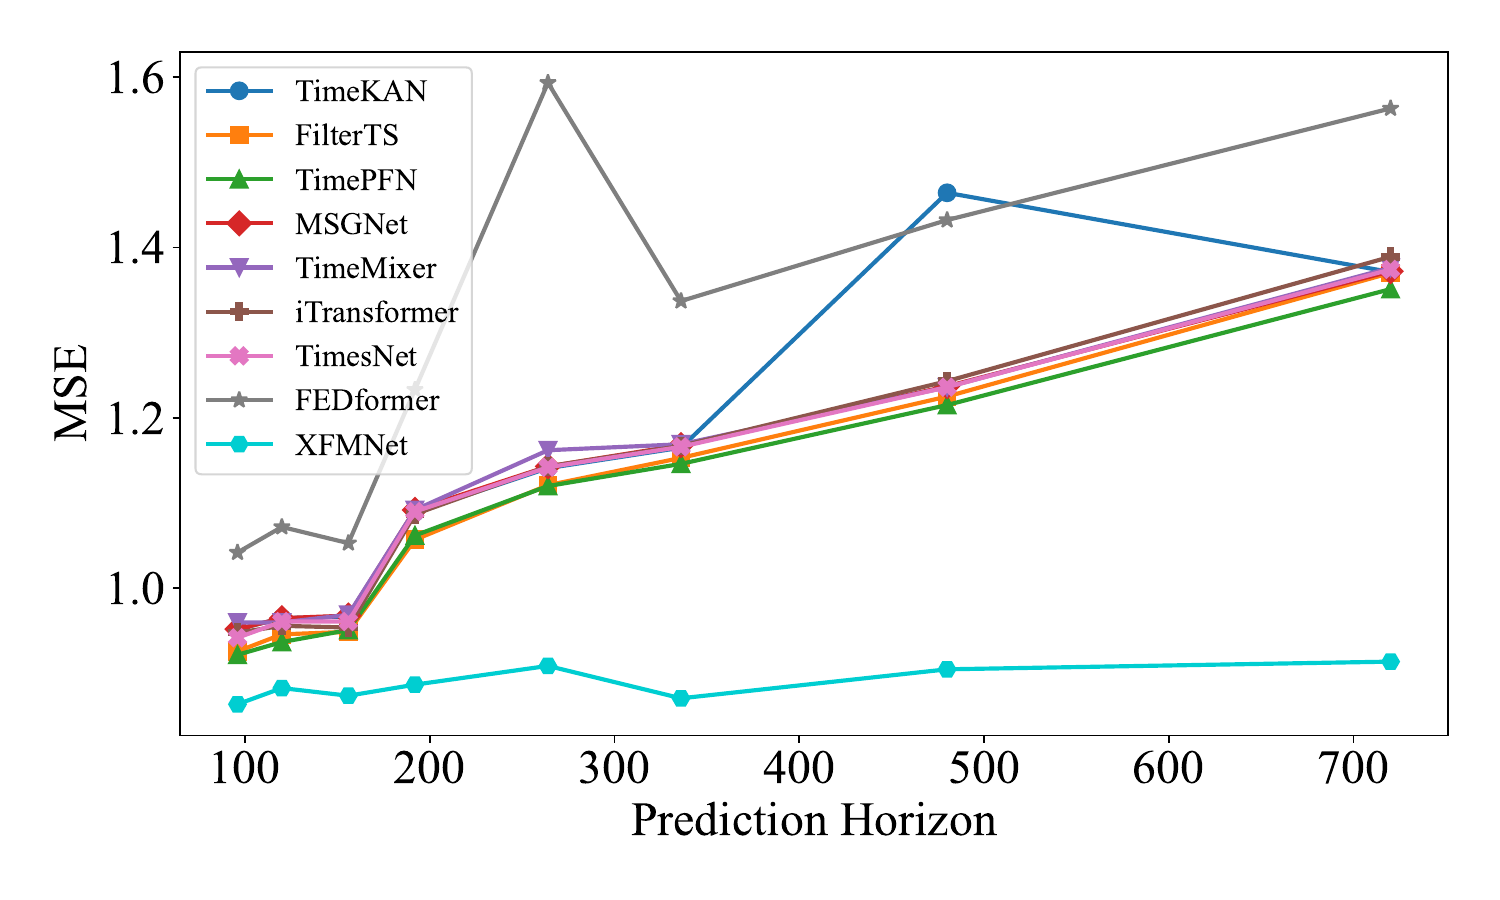}%
        \label{BJ1}
    }
    \quad
    \subfigure[MAE]{%
        \includegraphics[width=0.99\columnwidth]{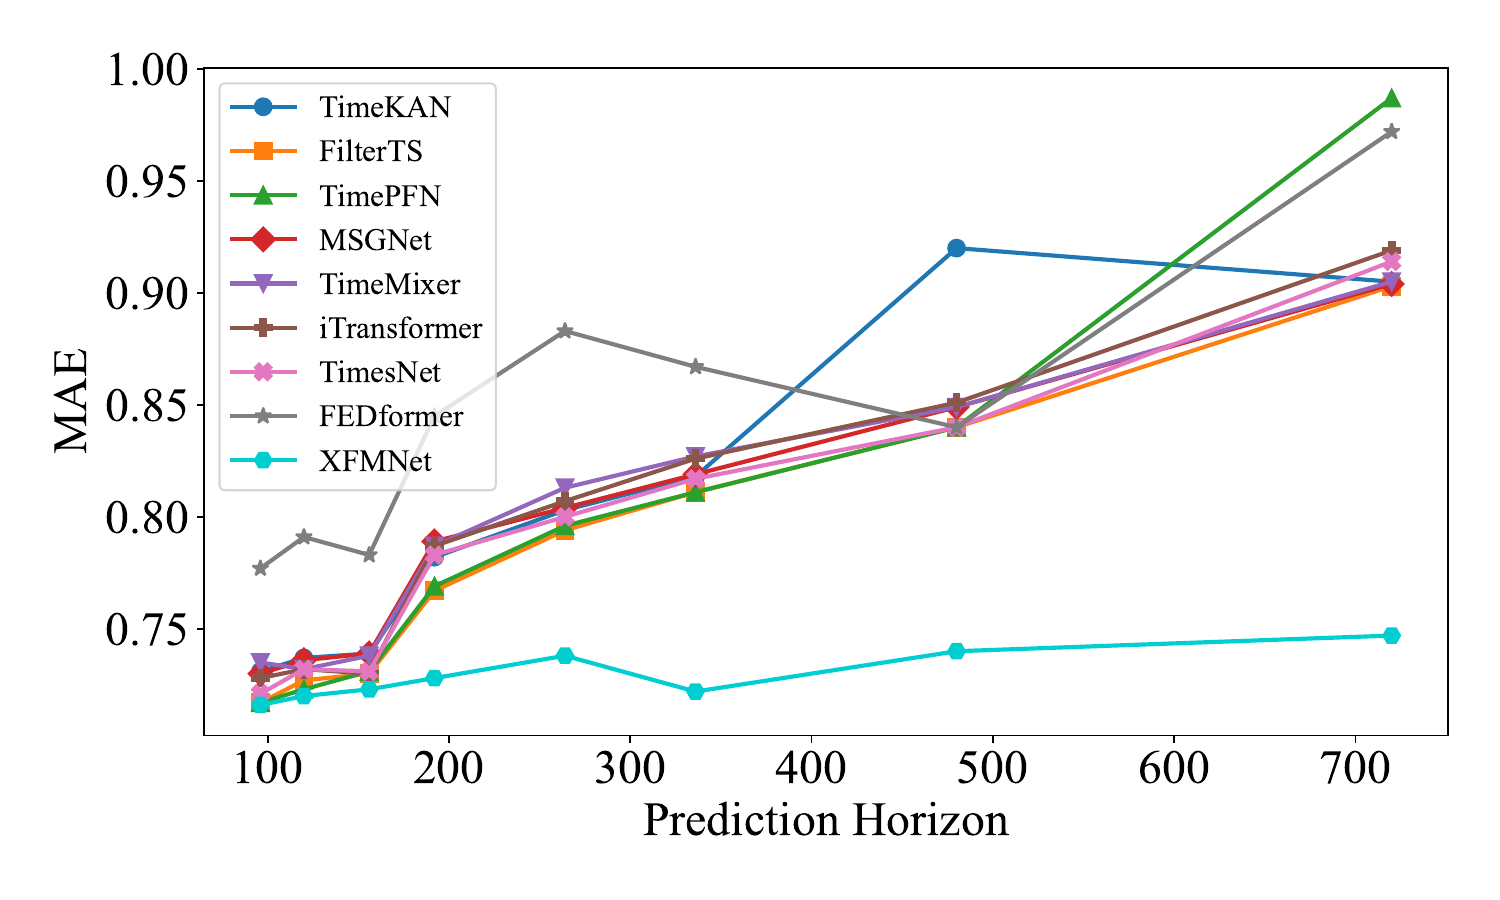}%
        \label{BJ2}
    }
    \caption{Performance comparison across different prediction horizons on the BJ dataset.}
    \label{BJ}
\end{figure}

%BTH
\begin{figure}[htbp]
    \centering
    \subfigure[MSE]{%
        \includegraphics[width=0.99\columnwidth]{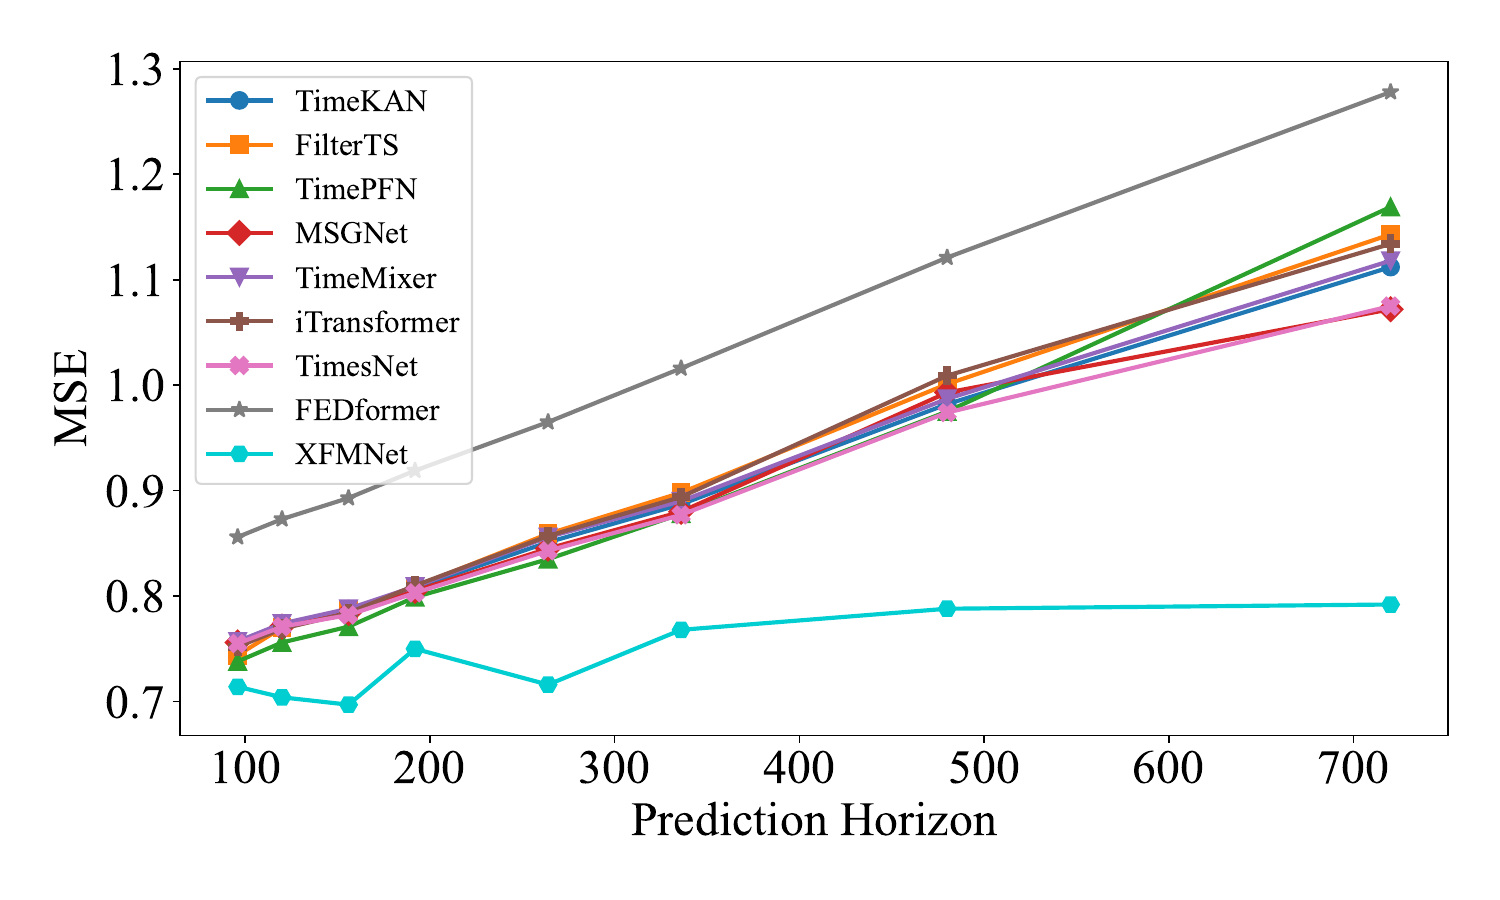}%
        \label{BTH1}
    }
    \quad
    \subfigure[MAE]{%
        \includegraphics[width=0.99\columnwidth]{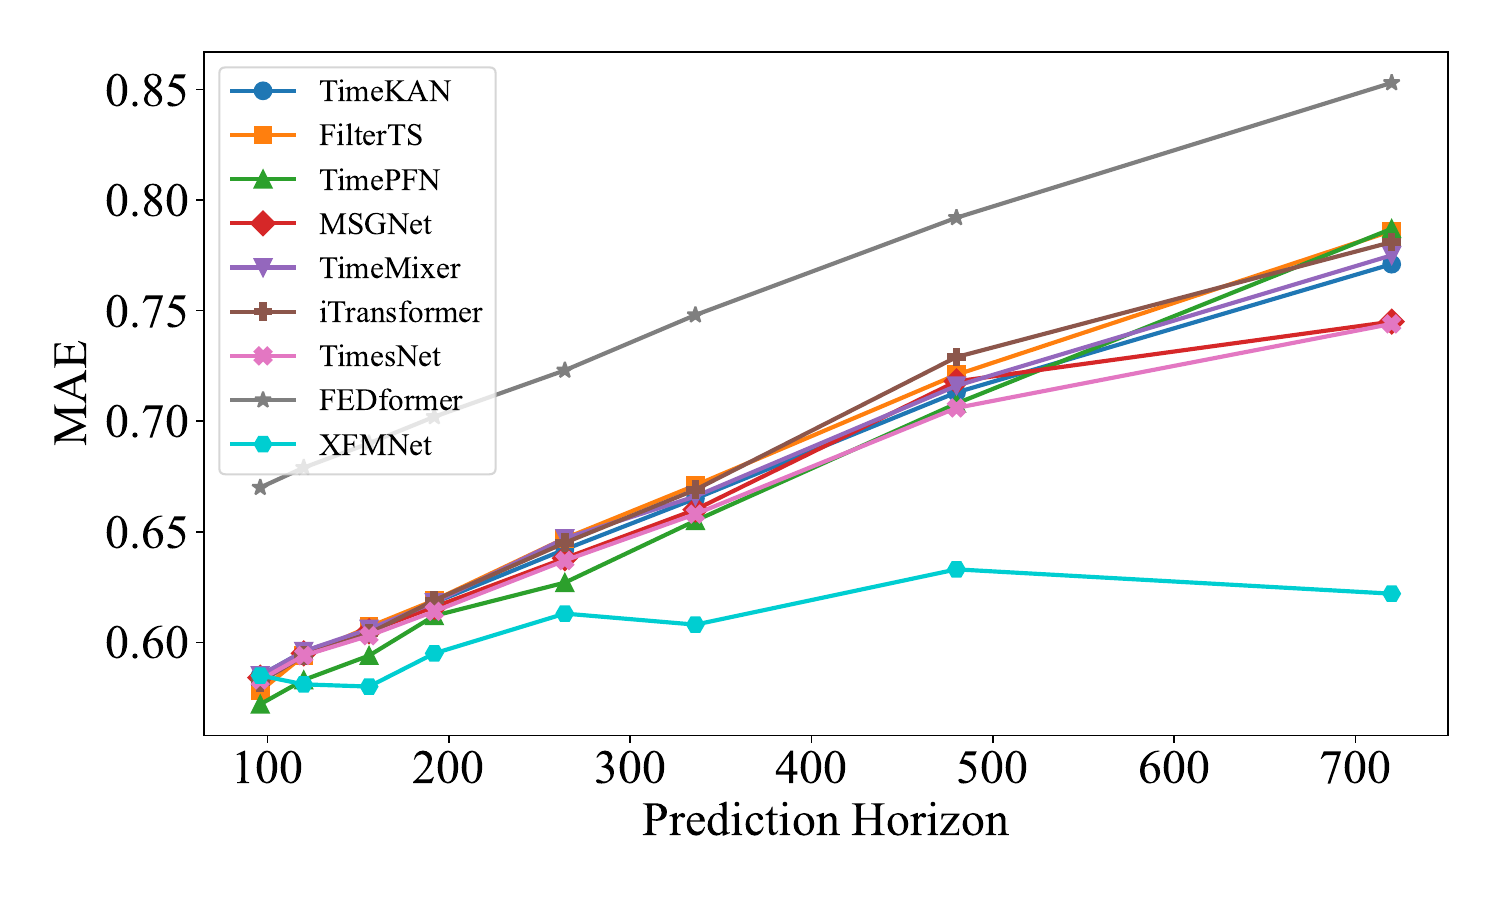}%
        \label{BTH2}
    }
    \caption{Performance comparison across different prediction horizons on the BTH dataset.}
    \label{BTH}
\end{figure}

%Ala
\begin{figure}[htbp]
    \centering
    \subfigure[MSE]{%
        \includegraphics[width=0.99\columnwidth]{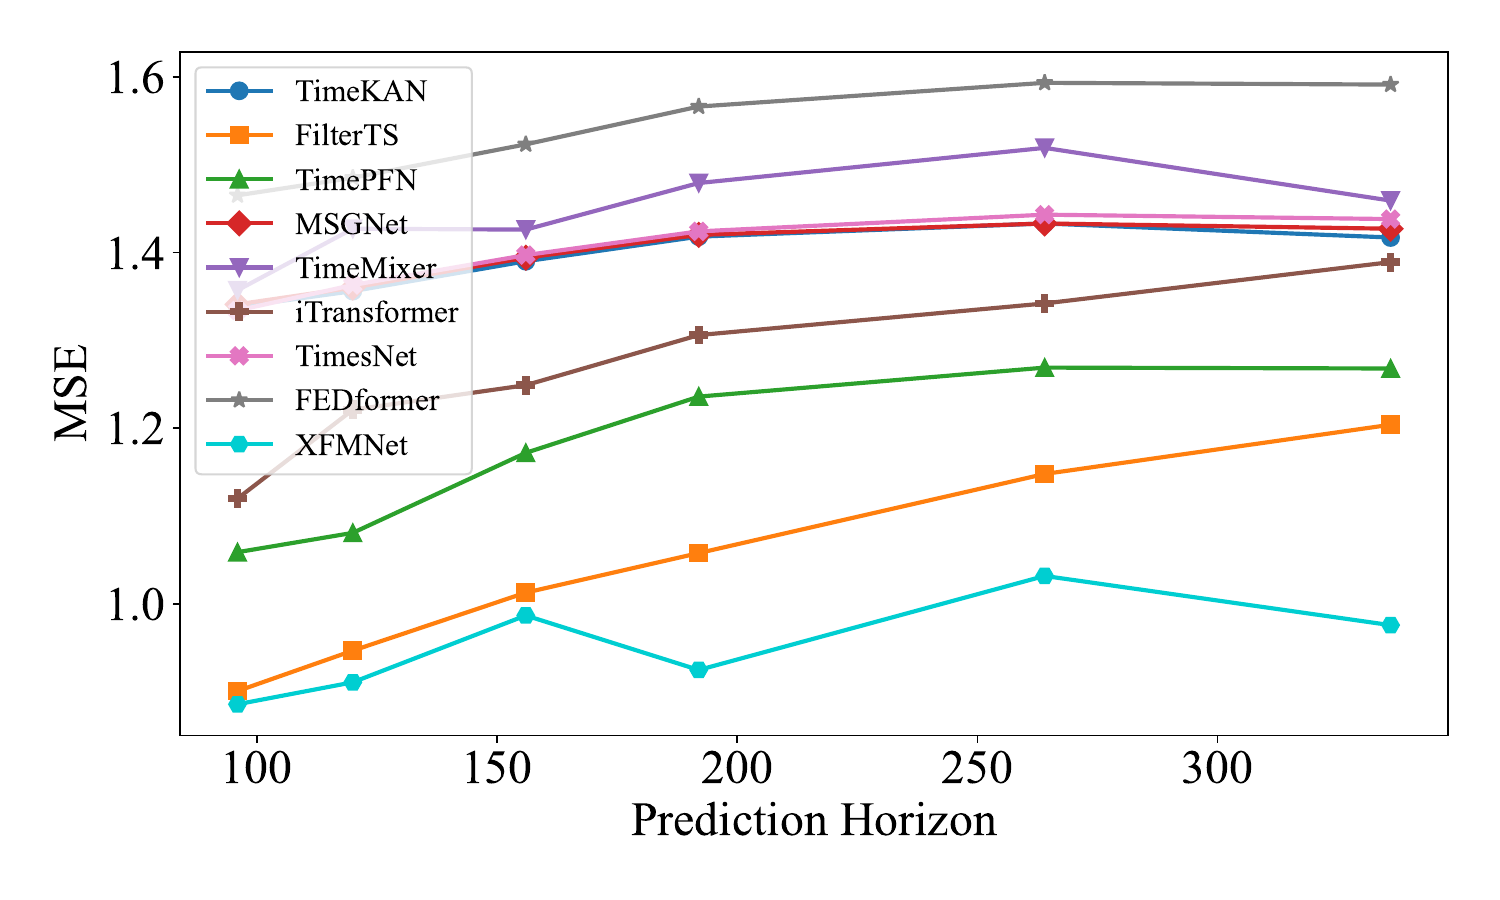}%
        \label{Ala1}
    }
    \quad
    \subfigure[MAE]{%
        \includegraphics[width=0.99\columnwidth]{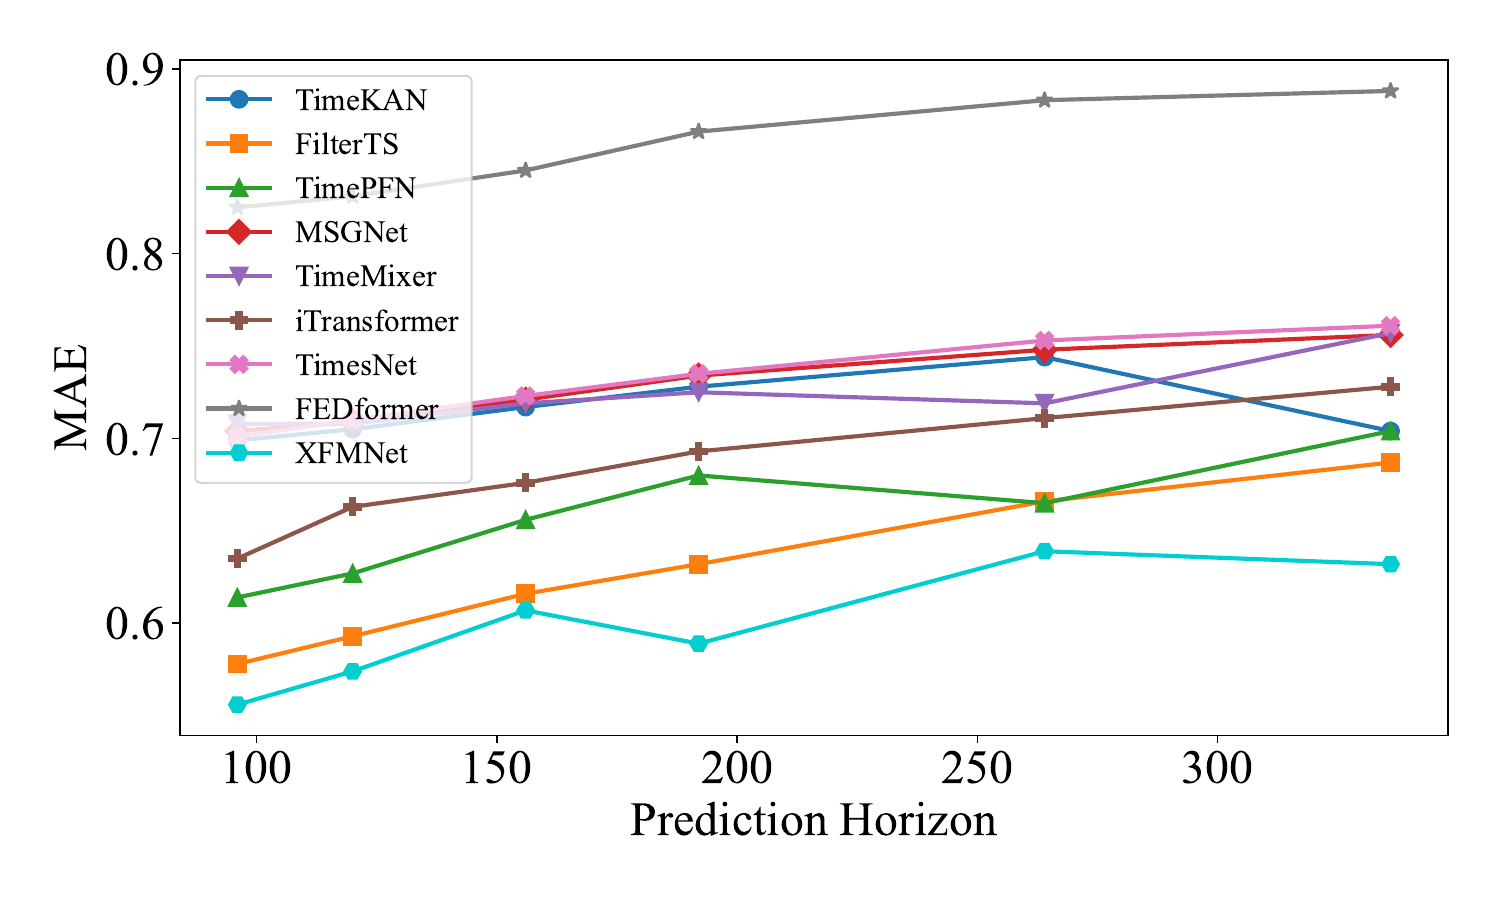}%
        \label{Ala2}
    }
    \caption{Performance comparison across different prediction horizons on the Ala dataset.}
    \label{Ala}
\end{figure}

\begin{figure}[!ht]
\centering  %图片全局居中
\subfigure[MSE]{
\label{pennu}
\includegraphics[width=0.5\columnwidth]{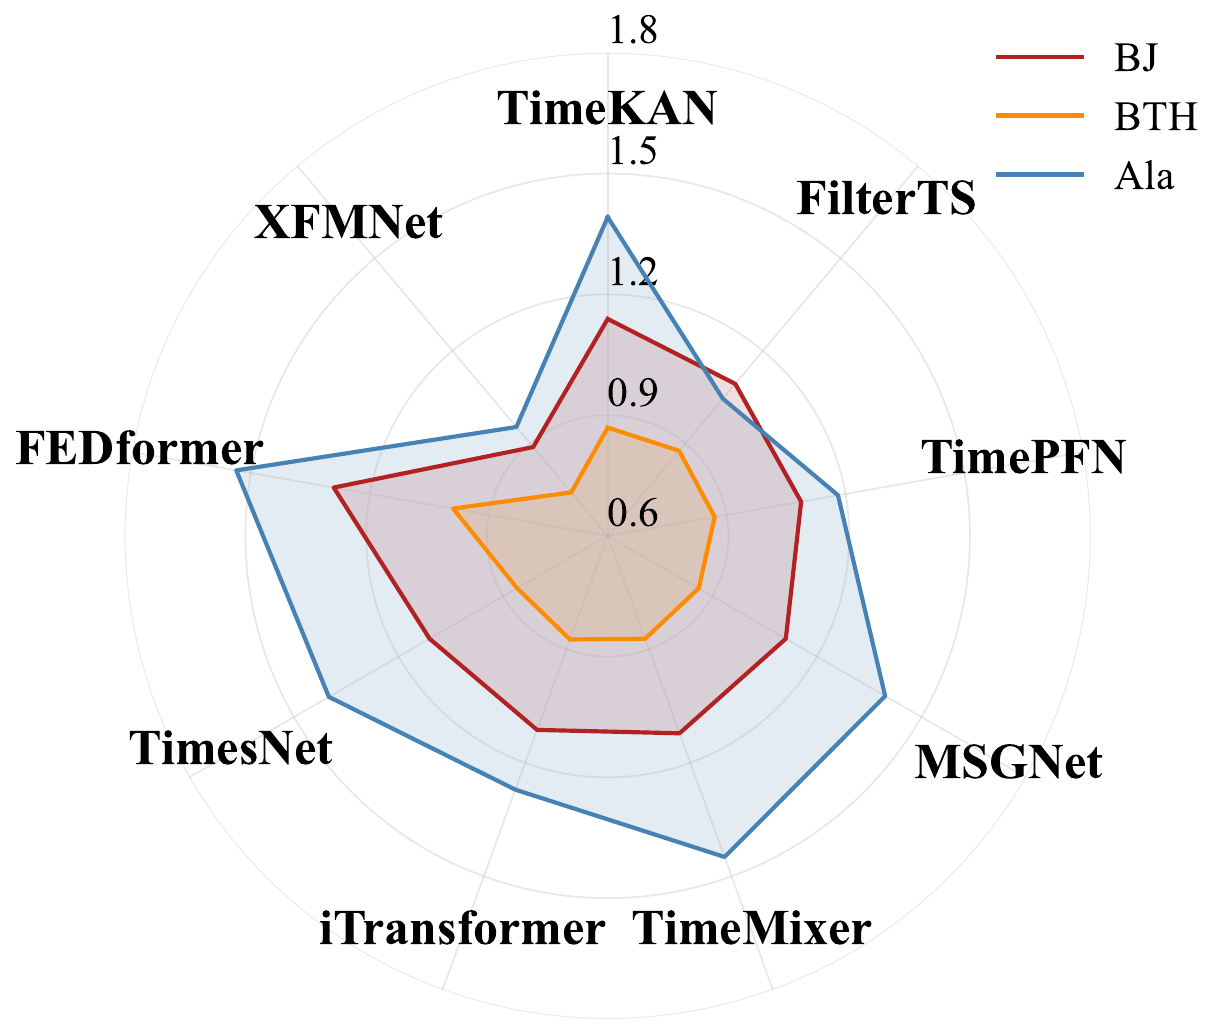}}\subfigure[MAE]{
\label{pendis}
\includegraphics[width=0.5\columnwidth]{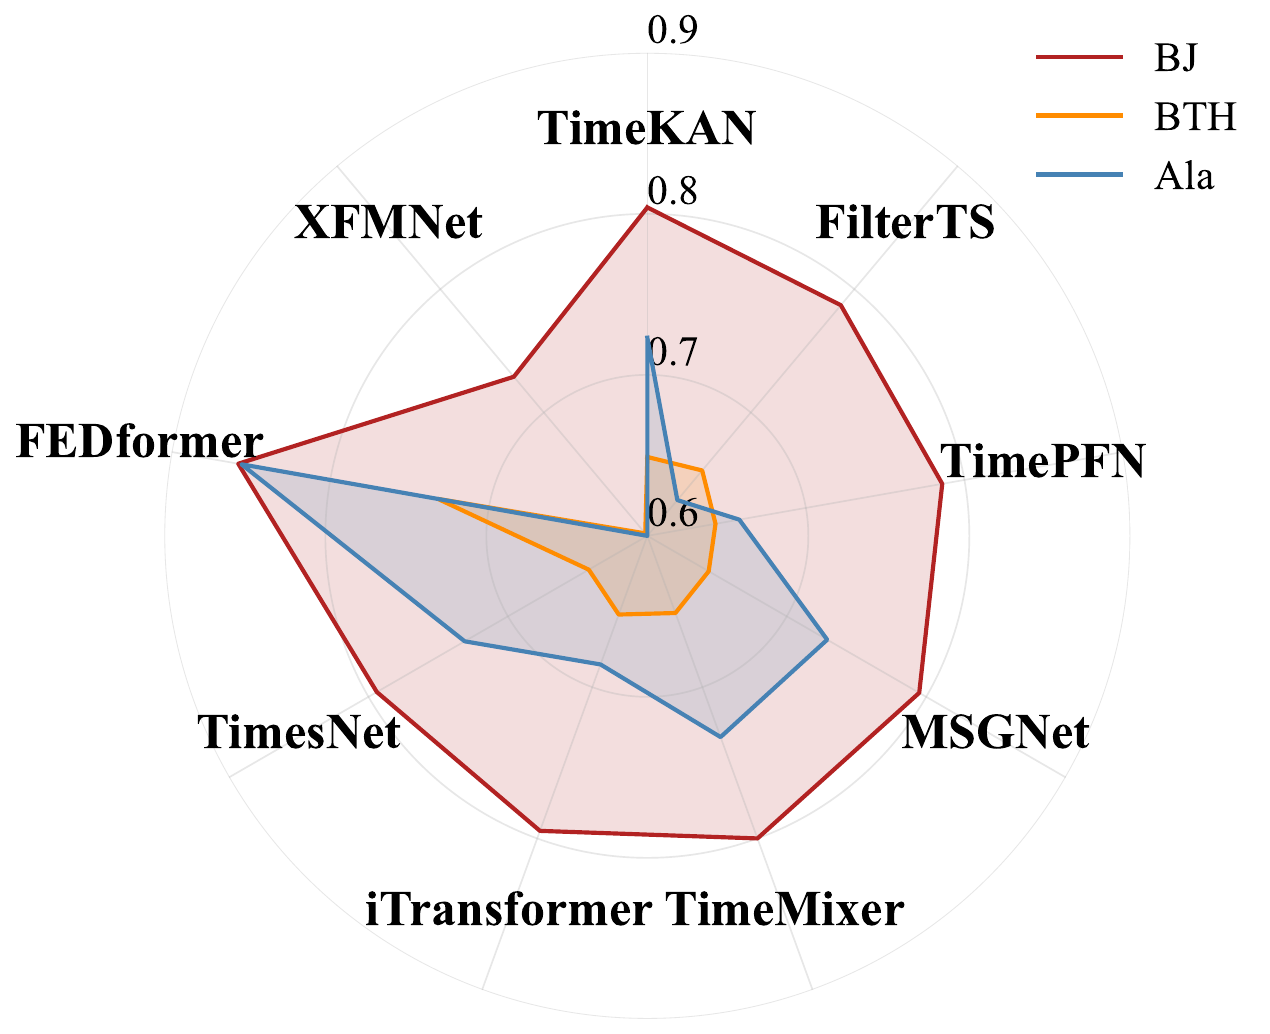}}
\caption{Radar chart of average MSE and MAE across three datasets under forecasting horizons starting from 96.}
\label{ladar}
\end{figure}

\begin{table*}[t!]
\centering
\small
\setlength{\tabcolsep}{2.6pt}
\renewcommand{\arraystretch}{1.3}
\caption{Long-term prediction results on three real-world datasets under varying prediction horizons. We highlight the best and the second-best results in \textbf{bold} and \underline{underline}, respectively.}
\begin{tabular}{c@{\hskip 10pt}c
@{\hskip 6pt}|c@{\hskip 2.5pt}c
@{\hskip 6pt}|c@{\hskip 2.5pt}c
@{\hskip 6pt}|c@{\hskip 2.5pt}c
@{\hskip 6pt}|c@{\hskip 2.5pt}c
@{\hskip 6pt}|c@{\hskip 2.5pt}c
@{\hskip 6pt}|c@{\hskip 2.5pt}c
@{\hskip 6pt}|c@{\hskip 2.5pt}c
@{\hskip 6pt}|c@{\hskip 2.5pt}c
@{\hskip 6pt}|c@{\hskip 2.5pt}c}
\toprule
%\multirow{3.5}{*}{Data} & \multirow{3.5}{*}{Horizon} 
%\multirow{3}{*}{Metric}
\multicolumn{2}{c|}{\multirow{2}{*}{Model}} & \multicolumn{2}{c}{TimeKAN} & \multicolumn{2}{c}{FilterTS} & \multicolumn{2}{c}{TimePFN} 
& \multicolumn{2}{c}{MSGNet} & \multicolumn{2}{c}{TimeMixer} &  \multicolumn{2}{c}{iTransformer} & \multicolumn{2}{c}{TimesNet} & \multicolumn{2}{c}{FEDformer} & \multicolumn{2}{c}{XFMNet} \\
& & \multicolumn{2}{c}{(2025)} & \multicolumn{2}{c}{(2025)} & \multicolumn{2}{c}{(2025)} & \multicolumn{2}{c}{(2024)} & \multicolumn{2}{c}{(2024)} & \multicolumn{2}{c}{(2024)} & \multicolumn{2}{c}{(2023)} & \multicolumn{2}{c}{(2022)} & \multicolumn{2}{c}{(ours)}\\
\cmidrule(lr){1-2} \cmidrule(lr){3-4} \cmidrule(lr){5-6} \cmidrule(lr){7-8} \cmidrule(lr){9-10} \cmidrule(lr){11-12} \cmidrule(lr){13-14} \cmidrule(lr){15-16} \cmidrule(lr){17-18}  \cmidrule(lr){19-20} 
\multicolumn{2}{c|}{Metric} & MSE & MAE & MSE & MAE & MSE & MAE & MSE & MAE & MSE & MAE & MSE & MAE & MSE & MAE & MSE & MAE & MSE & MAE\\
\midrule
\multirow{9}{*}{\rotatebox{90}{BJ}} 
& 96  & 0.952 & 0.731 & 0.926 & \underline{0.717} & \underline{0.922} & \underline{0.717} & 0.952 & 0.730 & 0.960 & 0.735 & 0.948 & 0.728 & 0.951 & 0.730 & 1.042 & 0.777 & \textbf{0.864} & \textbf{0.716} \\
& 120 & 0.965 & 0.737 & 0.946 & 0.727 & \underline{0.937} & \underline{0.723} & 0.965 & 0.736 & 0.968 & 0.738 & 0.956 & 0.732 & 0.969 & 0.737 & 1.072 & 0.791 & \textbf{0.883} & \textbf{0.720} \\
& 156 & 0.967 & 0.739 & \underline{0.949} & \underline{0.730} & 0.951 & 0.731 & 0.963 & 0.737 & 0.969 & 0.738 & 0.954 & 0.732 & 0.961 & 0.735 & 1.053 & 0.783 & \textbf{0.874} & \textbf{0.723} \\
& 192 & 1.089 & 0.782 & \underline{1.057} & \underline{0.767} & 1.064 & 0.772 & 1.091 & 0.782 & 1.092 & 0.783 & 1.089 & 0.780 & 1.090 & 0.781 & 1.233 & 0.845 & \textbf{0.887} & \textbf{0.728} \\
& 264 & 1.141 & 0.803 & \underline{1.121} & \underline{0.794} & \underline{1.121} & 0.796 & 1.143 & 0.804 & 1.162 & 0.813 & 1.148 & 0.804 & 1.142 & 0.802 & 1.593 & 0.883 & \textbf{0.909} & \textbf{0.738} \\
& 336 & 1.165 & 0.818 & 1.153 & 0.812 & \underline{1.146} & \underline{0.811} & 1.168 & 0.819 & 1.214 & 0.837 & 1.176 & 0.822 & 1.166 & 0.817 & 1.337 & 0.887 & \textbf{0.871} & \textbf{0.722} \\
& 480 & 1.464 & 0.920 & 1.225 & 0.844 & \underline{1.215} & \underline{0.840} & 1.237 & 0.849 & 1.237 & 0.850 & 1.243 & 0.850 & 1.236 & 0.847 & 1.432 & 0.924 & \textbf{0.905} & \textbf{0.740} \\
& 720 & 1.371 & 0.905 & 1.370 & 0.903 & \underline{1.351} & \underline{0.897} & 1.372 & 0.904 & 1.376 & 0.905 & 1.389 & 0.909 & 1.374 & 0.904 & 1.563 & 0.972 & \textbf{0.914} & \textbf{0.747} \\
& Avg & 1.139 & 0.804 & 1.093 & 0.787 &  \underline{1.088} &  \underline{0.786} & 1.111 & 0.795 & 1.122 & 0.800 & 1.113 & 0.795 & 1.111 & 0.794 & 1.291 & 0.858 & \textbf{0.888} & \textbf{0.729}\\
\midrule
\multirow{9}{*}{\rotatebox{90}{BTH}} 
& 96  & 0.757 & 0.585 & 0.744 & \underline{0.578} & \underline{0.738} & \textbf{0.572} & 0.756 & 0.584 & 0.757 & 0.585 & 0.752 & 0.582 & 0.755 & 0.583 & 0.856 & 0.670 & \textbf{0.714} & 0.585 \\
& 120 & 0.773 & 0.596 & 0.770 & 0.594 & \underline{0.756} & \underline{0.583} & 0.771 & 0.595 & 0.774 & 0.596 & 0.769 & 0.594 & 0.771 & 0.594 & 0.873 & 0.679 & \textbf{0.704} & \textbf{0.581} \\
& 156 & 0.785 & 0.605 & 0.787 & 0.607 & \underline{0.771} & \underline{0.594} & 0.784 & 0.605 & 0.788 & 0.606 & 0.784 & 0.604 & 0.782 & 0.603 & 0.893 & 0.690 & \textbf{0.697} & \textbf{0.580} \\
& 192 & 0.808 & 0.618 & 0.809 & 0.619 & \underline{0.799} & \underline{0.612} & 0.805 & 0.616 & 0.809 & 0.618 & 0.810 & 0.619 & 0.803 & 0.614 & 0.919 & 0.702 & \textbf{0.750} & \textbf{0.595} \\
& 264 & 0.851 & 0.642 & 0.859 & 0.647 & \underline{0.835} & \underline{0.627} & 0.845 & 0.638 & 0.856 & 0.647 & 0.857 & 0.645 & 0.843 & 0.637 & 0.965 & 0.723 & \textbf{0.716} & \textbf{0.613} \\
& 336 & 0.887 & 0.665 & 0.898 & 0.671 & 0.878 & \underline{0.655} & 0.880 & 0.660 & 0.890 & 0.666 & 0.894 & 0.669 & \underline{0.877} & 0.658 & 1.016 & 0.748 & \textbf{0.768} & \textbf{0.608} \\
& 480 & 0.982 & 0.713 & 1.001 & 0.721 & 1.015 & 0.713 & 0.975 & 0.708 & 0.987 & 0.716 & 0.993 & 0.718 & \underline{0.974} & \underline{0.706} & 1.121 & 0.792 & \textbf{0.788} & \textbf{0.633} \\
& 720 & 1.112 & 0.771 & 1.143 & 0.786 & 1.169 & 0.787 & \underline{1.072} & 0.745 & 1.118 & 0.775 & 1.134 & 0.781 & 1.075 & \underline{0.744} & 1.278 & 0.853 & \textbf{0.792} & \textbf{0.622} \\
& Avg & 0.869 & 0.649 & 0.876 & 0.653 & 0.870 & 0.643 & 0.861 & 0.644 & 0.872 & 0.651 & 0.874 & 0.652 & \underline{0.860} & \underline{0.642} & 0.990 & 0.732 & \textbf{0.741} & \textbf{0.602}\\
\midrule

\multirow{9}{*}{\rotatebox{90}{Ala}} 
& 96 & 1.338 & 0.699 & \underline{0.901} & \underline{0.578} & 1.059 & 0.614 & 1.341 & 0.704 & 1.357 & 0.708 & 1.120 & 0.635 & 1.334 & 0.701 & 1.465 & 0.825 & \textbf{0.886} & \textbf{0.556} \\
& 120 & 1.356 & 0.705 & \underline{0.947} & \underline{0.593} & 1.081 & 0.627 & 1.360 & 0.709 & 1.427 & 0.708 & 1.221 & 0.663 & 1.363 & 0.710 & 1.485 & 0.831 & \textbf{0.911} & \textbf{0.574} \\
& 156 & 1.390 & 0.717 & \underline{1.013} & \underline{0.616} & 1.172 & 0.656 & 1.394 & 0.721 & 1.436 & 0.719 & 1.249 & 0.676 & 1.397 & 0.723 & 1.523 & 0.845 & \textbf{0.987} & \textbf{0.607} \\
& 192 & 1.418 & 0.728 & \underline{1.058} & \underline{0.632} & 1.236 & 0.680 & 1.421 & 0.734 & 1.479 & 0.725 & 1.306 & 0.693 & 1.424 & 0.735 & 1.566 & 0.866 & \textbf{0.925} & \textbf{0.589} \\
& 264 & 1.433 & 0.744 & \underline{1.148} & 0.666 & 1.269 & \underline{0.665} & 1.433 & 0.748 & 1.519 & 0.778 & 1.342 & 0.712 & 1.443 & 0.753 & 1.593 & 0.883 & \textbf{1.032} & \textbf{0.639} \\
& 336 & 1.417 & 0.747 & \underline{1.204} & \underline{0.687} & 1.268 & 0.704 & 1.427 & 0.756 & 1.475 & 0.757 & 1.389 & 0.728 & 1.438 & 0.761 & 1.591 & 0.888 & \textbf{0.976} & \textbf{0.632} \\
& Avg & 1.392 & 0.723 & \underline{1.045} & \underline{0.629} & 1.181 & 0.658 & 1.396 & 0.729 & 1.449 & 0.733 & 1.271 & 0.685 & 1.400 & 0.731 & 1.537 & 0.856 & \textbf{0.953} & \textbf{0.600}\\

\bottomrule
\end{tabular}
\label{tab:main_results}
\end{table*}

In addition, we compare \texttt{XFMnet} with other multimodal fusion strategies and large multimodal model. The results are shown in Table \ref{multimodallarge} and Figs. \ref{} to \ref{}. It is shown that

\begin{table*}[t!]
\centering
\small
\setlength{\tabcolsep}{2.6pt}
\renewcommand{\arraystretch}{1.3}
\caption{Comparison of different fusion strategies and multimodal models. We highlight the best and the second-best results in \textbf{bold} and \underline{underline}, respectively.}
\begin{tabular}{c@{\hskip 10pt}c
@{\hskip 6pt}|c@{\hskip 2.5pt}c
@{\hskip 6pt}|c@{\hskip 2.5pt}c
@{\hskip 6pt}|c@{\hskip 2.5pt}c
@{\hskip 6pt}|c@{\hskip 2.5pt}c
@{\hskip 6pt}|c@{\hskip 2.5pt}c
@{\hskip 6pt}|c@{\hskip 2.5pt}c
@{\hskip 6pt}|c@{\hskip 2.5pt}c
@{\hskip 6pt}|c@{\hskip 2.5pt}c
@{\hskip 6pt}|c@{\hskip 2.5pt}c}
\toprule
%\multirow{3.5}{*}{Data} & \multirow{3.5}{*}{Horizon} 
%\multirow{3}{*}{Metric}
\multicolumn{2}{c|}{\multirow{2}{*}{Model}} & \multicolumn{2}{c}{TimeKAN} & \multicolumn{2}{c}{FilterTS} & \multicolumn{2}{c}{TimePFN} 
& \multicolumn{2}{c}{MSGNet} & \multicolumn{2}{c}{TimeMixer} &  \multicolumn{2}{c}{iTransformer} & \multicolumn{2}{c}{TimesNet} & \multicolumn{2}{c}{FEDformer} & \multicolumn{2}{c}{XFMNet} \\
& & \multicolumn{2}{c}{(2025)} & \multicolumn{2}{c}{(2025)} & \multicolumn{2}{c}{(2025)} & \multicolumn{2}{c}{(2024)} & \multicolumn{2}{c}{(2024)} & \multicolumn{2}{c}{(2024)} & \multicolumn{2}{c}{(2023)} & \multicolumn{2}{c}{(2022)} & \multicolumn{2}{c}{(ours)}\\
\cmidrule(lr){1-2} \cmidrule(lr){3-4} \cmidrule(lr){5-6} \cmidrule(lr){7-8} \cmidrule(lr){9-10} \cmidrule(lr){11-12} \cmidrule(lr){13-14} \cmidrule(lr){15-16} \cmidrule(lr){17-18}  \cmidrule(lr){19-20} 
\multicolumn{2}{c|}{Metric} & MSE & MAE & MSE & MAE & MSE & MAE & MSE & MAE & MSE & MAE & MSE & MAE & MSE & MAE & MSE & MAE & MSE & MAE\\
\midrule
\multirow{9}{*}{\rotatebox{90}{BJ}} 
& 96  & 0.952 & 0.731 & 0.926 & \underline{0.717} & \underline{0.922} & \underline{0.717} & 0.952 & 0.730 & 0.960 & 0.735 & 0.948 & 0.728 & 0.951 & 0.730 & 1.042 & 0.777 & \textbf{0.864} & \textbf{0.716} \\
& 120 & 0.965 & 0.737 & 0.946 & 0.727 & \underline{0.937} & \underline{0.723} & 0.965 & 0.736 & 0.968 & 0.738 & 0.956 & 0.732 & 0.969 & 0.737 & 1.072 & 0.791 & \textbf{0.883} & \textbf{0.720} \\
& 156 & 0.967 & 0.739 & \underline{0.949} & \underline{0.730} & 0.951 & 0.731 & 0.963 & 0.737 & 0.969 & 0.738 & 0.954 & 0.732 & 0.961 & 0.735 & 1.053 & 0.783 & \textbf{0.874} & \textbf{0.723} \\
& 192 & 1.089 & 0.782 & \underline{1.057} & \underline{0.767} & 1.064 & 0.772 & 1.091 & 0.782 & 1.092 & 0.783 & 1.089 & 0.780 & 1.090 & 0.781 & 1.233 & 0.845 & \textbf{0.887} & \textbf{0.728} \\
& 264 & 1.141 & 0.803 & \underline{1.121} & \underline{0.794} & \underline{1.121} & 0.796 & 1.143 & 0.804 & 1.162 & 0.813 & 1.148 & 0.804 & 1.142 & 0.802 & 1.593 & 0.883 & \textbf{0.909} & \textbf{0.738} \\
& 336 & 1.165 & 0.818 & 1.153 & 0.812 & \underline{1.146} & \underline{0.811} & 1.168 & 0.819 & 1.214 & 0.837 & 1.176 & 0.822 & 1.166 & 0.817 & 1.337 & 0.887 & \textbf{0.871} & \textbf{0.722} \\
& 480 & 1.464 & 0.920 & 1.225 & 0.844 & \underline{1.215} & \underline{0.840} & 1.237 & 0.849 & 1.237 & 0.850 & 1.243 & 0.850 & 1.236 & 0.847 & 1.432 & 0.924 & \textbf{0.905} & \textbf{0.740} \\
& 720 & 1.371 & 0.905 & 1.370 & 0.903 & \underline{1.351} & \underline{0.897} & 1.372 & 0.904 & 1.376 & 0.905 & 1.389 & 0.909 & 1.374 & 0.904 & 1.563 & 0.972 & \textbf{0.914} & \textbf{0.747} \\
& Avg & 1.139 & 0.804 & 1.093 & 0.787 &  \underline{1.088} &  \underline{0.786} & 1.111 & 0.795 & 1.122 & 0.800 & 1.113 & 0.795 & 1.111 & 0.794 & 1.291 & 0.858 & \textbf{0.888} & \textbf{0.729}\\
\midrule
\multirow{9}{*}{\rotatebox{90}{BTH}} 
& 96  & 0.757 & 0.585 & 0.744 & \underline{0.578} & \underline{0.738} & \textbf{0.572} & 0.756 & 0.584 & 0.757 & 0.585 & 0.752 & 0.582 & 0.755 & 0.583 & 0.856 & 0.670 & \textbf{0.714} & 0.585 \\
& 120 & 0.773 & 0.596 & 0.770 & 0.594 & \underline{0.756} & \underline{0.583} & 0.771 & 0.595 & 0.774 & 0.596 & 0.769 & 0.594 & 0.771 & 0.594 & 0.873 & 0.679 & \textbf{0.704} & \textbf{0.581} \\
& 156 & 0.785 & 0.605 & 0.787 & 0.607 & \underline{0.771} & \underline{0.594} & 0.784 & 0.605 & 0.788 & 0.606 & 0.784 & 0.604 & 0.782 & 0.603 & 0.893 & 0.690 & \textbf{0.697} & \textbf{0.580} \\
& 192 & 0.808 & 0.618 & 0.809 & 0.619 & \underline{0.799} & \underline{0.612} & 0.805 & 0.616 & 0.809 & 0.618 & 0.810 & 0.619 & 0.803 & 0.614 & 0.919 & 0.702 & \textbf{0.750} & \textbf{0.595} \\
& 264 & 0.851 & 0.642 & 0.859 & 0.647 & \underline{0.835} & \underline{0.627} & 0.845 & 0.638 & 0.856 & 0.647 & 0.857 & 0.645 & 0.843 & 0.637 & 0.965 & 0.723 & \textbf{0.716} & \textbf{0.613} \\
& 336 & 0.887 & 0.665 & 0.898 & 0.671 & 0.878 & \underline{0.655} & 0.880 & 0.660 & 0.890 & 0.666 & 0.894 & 0.669 & \underline{0.877} & 0.658 & 1.016 & 0.748 & \textbf{0.768} & \textbf{0.608} \\
& 480 & 0.982 & 0.713 & 1.001 & 0.721 & 1.015 & 0.713 & 0.975 & 0.708 & 0.987 & 0.716 & 0.993 & 0.718 & \underline{0.974} & \underline{0.706} & 1.121 & 0.792 & \textbf{0.788} & \textbf{0.633} \\
& 720 & 1.112 & 0.771 & 1.143 & 0.786 & 1.169 & 0.787 & \underline{1.072} & 0.745 & 1.118 & 0.775 & 1.134 & 0.781 & 1.075 & \underline{0.744} & 1.278 & 0.853 & \textbf{0.792} & \textbf{0.622} \\
& Avg & 0.869 & 0.649 & 0.876 & 0.653 & 0.870 & 0.643 & 0.861 & 0.644 & 0.872 & 0.651 & 0.874 & 0.652 & \underline{0.860} & \underline{0.642} & 0.990 & 0.732 & \textbf{0.741} & \textbf{0.602}\\
\midrule

\multirow{9}{*}{\rotatebox{90}{Ala}} 
& 96 & 1.338 & 0.699 & \underline{0.901} & \underline{0.578} & 1.059 & 0.614 & 1.341 & 0.704 & 1.357 & 0.708 & 1.120 & 0.635 & 1.334 & 0.701 & 1.465 & 0.825 & \textbf{0.886} & \textbf{0.556} \\
& 120 & 1.356 & 0.705 & \underline{0.947} & \underline{0.593} & 1.081 & 0.627 & 1.360 & 0.709 & 1.427 & 0.708 & 1.221 & 0.663 & 1.363 & 0.710 & 1.485 & 0.831 & \textbf{0.911} & \textbf{0.574} \\
& 156 & 1.390 & 0.717 & \underline{1.013} & \underline{0.616} & 1.172 & 0.656 & 1.394 & 0.721 & 1.436 & 0.719 & 1.249 & 0.676 & 1.397 & 0.723 & 1.523 & 0.845 & \textbf{0.987} & \textbf{0.607} \\
& 192 & 1.418 & 0.728 & \underline{1.058} & \underline{0.632} & 1.236 & 0.680 & 1.421 & 0.734 & 1.479 & 0.725 & 1.306 & 0.693 & 1.424 & 0.735 & 1.566 & 0.866 & \textbf{0.925} & \textbf{0.589} \\
& 264 & 1.433 & 0.744 & \underline{1.148} & 0.666 & 1.269 & \underline{0.665} & 1.433 & 0.748 & 1.519 & 0.778 & 1.342 & 0.712 & 1.443 & 0.753 & 1.593 & 0.883 & \textbf{1.032} & \textbf{0.639} \\
& 336 & 1.417 & 0.747 & \underline{1.204} & \underline{0.687} & 1.268 & 0.704 & 1.427 & 0.756 & 1.475 & 0.757 & 1.389 & 0.728 & 1.438 & 0.761 & 1.591 & 0.888 & \textbf{0.976} & \textbf{0.632} \\
& Avg & 1.392 & 0.723 & \underline{1.045} & \underline{0.629} & 1.181 & 0.658 & 1.396 & 0.729 & 1.449 & 0.733 & 1.271 & 0.685 & 1.400 & 0.731 & 1.537 & 0.856 & \textbf{0.953} & \textbf{0.600}\\

\bottomrule
\end{tabular}
\label{multimodallarge}
\end{table*}

\subsection{Computational Cost}
Table \ref{computing} shows the computational cost of all compared models.

\begin{table*}[t!]
\centering
\small
\setlength{\tabcolsep}{2.6pt}
\renewcommand{\arraystretch}{1.3}
\caption{Comparison of model parameters (Par) and memory consumption (MC) on each dataset.}
\begin{tabular}{c|cc|cc|cc|cc|cc|cc|cc|cc|cc}
\toprule
\multicolumn{1}{c|}{Datasets} 
& \multicolumn{2}{c}{TimeKAN} 
& \multicolumn{2}{c}{FilterTS} 
& \multicolumn{2}{c}{TimePFN} 
& \multicolumn{2}{c}{MSGNet} 
& \multicolumn{2}{c}{TimeMixer} 
& \multicolumn{2}{c}{iTransformer} 
& \multicolumn{2}{c}{TimesNet} 
& \multicolumn{2}{c}{FEDformer} 
& \multicolumn{2}{c}{XFMNet} \\
\cmidrule(lr){2-3}
\cmidrule(lr){4-5}
\cmidrule(lr){6-7}
\cmidrule(lr){8-9}
\cmidrule(lr){10-11}
\cmidrule(lr){12-13}
\cmidrule(lr){14-15}
\cmidrule(lr){16-17}
\cmidrule(lr){18-19}
Metrics & Par & MC & Par & MC & Par & MC & Par & MC & Par & MC & Par & MC & Par & MC & Par & MC & Par & MC \\
\midrule
BJ  & xxx & xxx & xxx & xxx & xxx & xxx & xxx & xxx & xxx & xxx & xxx & xxx & xxx & xxx & xxx & xxx & xxx & xxx \\
BTH & xxx & xxx & xxx & xxx & xxx & xxx & xxx & xxx & xxx & xxx & xxx & xxx & xxx & xxx & xxx & xxx & xxx & xxx \\
Ala & xxx & xxx & xxx & xxx & xxx & xxx & xxx & xxx & xxx & xxx & xxx & xxx & xxx & xxx & xxx & xxx & xxx & xxx \\
\bottomrule
\end{tabular}
\label{computing}
\end{table*}

\subsection{Effectiveness of \texttt{XGateFusion}} %与别的方法比较 三个数据集都画融合图
Fig.~\ref{aba_mae} presents the mean MAE results of multiple model variants. Removing the recursive fusion module (w/o-RF) leads to noticeable performance drops, particularly on the Ala and BTH datasets, where complex non-stationary dynamics are more prominent. This highlights the importance of iterative refinement in capturing evolving spatiotemporal signals. More critically, replacing \texttt{XGateFusion} with a simple MLP (re-XGF-MLP) results in the most substantial degradation across all datasets. These results underscore the necessity of a learnable, modality-aware fusion strategy for effective cross-modal integration. %Replacing the LocTrend decomposition with a moving average filter (re-LT-MA) leads to moderate degradation, indicating that fine-grained trend-seasonal disentanglement also supports accurate modeling. 
The second worst performance is observed when both \texttt{XGateFusion} and LocTrend are replaced (re-MLP-MA), confirming the synergy between adaptive fusion and signal decomposition. The worst performance is entirely removing \texttt{XGateFusion}, demonstrating its importance in integrating visual cues.

To further understand how \texttt{XGateFusion} facilitates effective cross-modal integration, we visualize the internal feature evolution at three representative fusion stages on the BTH and Ala datasets, as shown in Fig. \ref{fusionfinBTH} and Fig. \ref{fusionfinAla}. Specifically, we track: (1) the output of cross-attention ($A_{\mathrm{t} \leftrightarrow \mathrm{i}}$), (2) the gated fusion result ($S_{\mathrm{f}}^{(l)}$), and (3) the final recursive representation ($\hat{Z}^{(l,n)}$). The top rows of each figure show the channel-wise Pearson correlation matrices. On both datasets, $A_{\mathrm{t} \leftrightarrow \mathrm{i}}$ displays strong redundancy and modality-specific entanglement, as evidenced by dense off-diagonal patterns. In $S_{\mathrm{f}}^{(l)}$, the correlation becomes sparser and more structured, suggesting that the gating mechanism begins to disentangle irrelevant cross-modal noise and emphasize salient cues. Finally, in $\hat{Z}^{(l,n)}$, the correlations exhibit well-organized blocks, indicating the emergence of hierarchically structured, modality-enhanced representations. The bottom rows present the corresponding local activation heatmaps. Initially, the activations are scattered and relatively diffuse in $A_{\mathrm{t} \leftrightarrow \mathrm{i}}$, lacking semantic focus. Through further fusion, $S_{\mathrm{f}}^{(l)}$ exhibits localized emphasis with clearer spatial relevance. At the final stage, $\hat{Z}^{(l,n)}$ shows sharply defined activations that correspond to critical spatial–temporal features. These observations suggest that \texttt{XGateFusion} facilitates channel-wise decorrelation and spatial localization with semantic filtering, which are essential for robust forecasting.

In summary, these results confirm that \texttt{XGateFusion} plays a central role in guiding effective and adaptive cross-modal integration. Its design supports progressive signal disentanglement, semantic enhancement, and recursive refinement, which together contribute to the superior performance observed in the main experiments.

\begin{figure}[!ht]
\centering
\includegraphics[width=0.97\columnwidth]{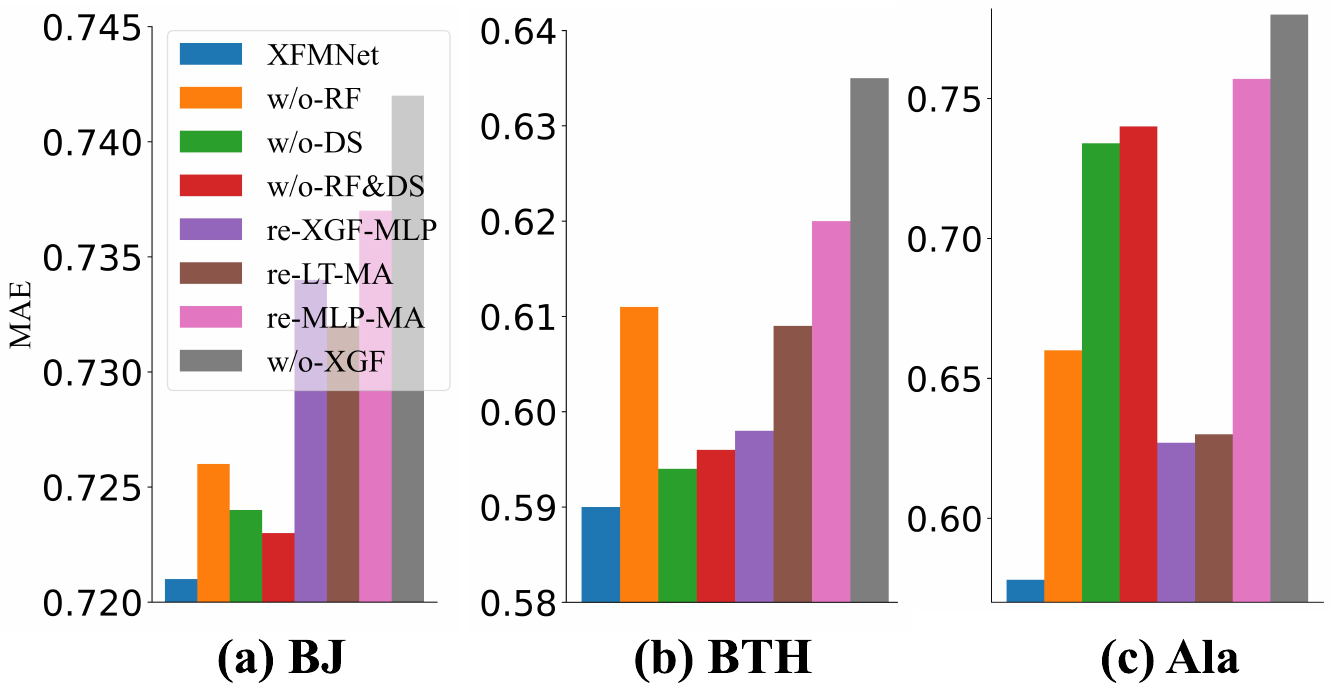} 
\caption{Ablation study on three datasets. Each bar represents the mean MAE obtained by different model variants.}
\label{aba_mae}
\end{figure}

\begin{figure}[!ht]
\centering
\includegraphics[width=0.99\columnwidth]{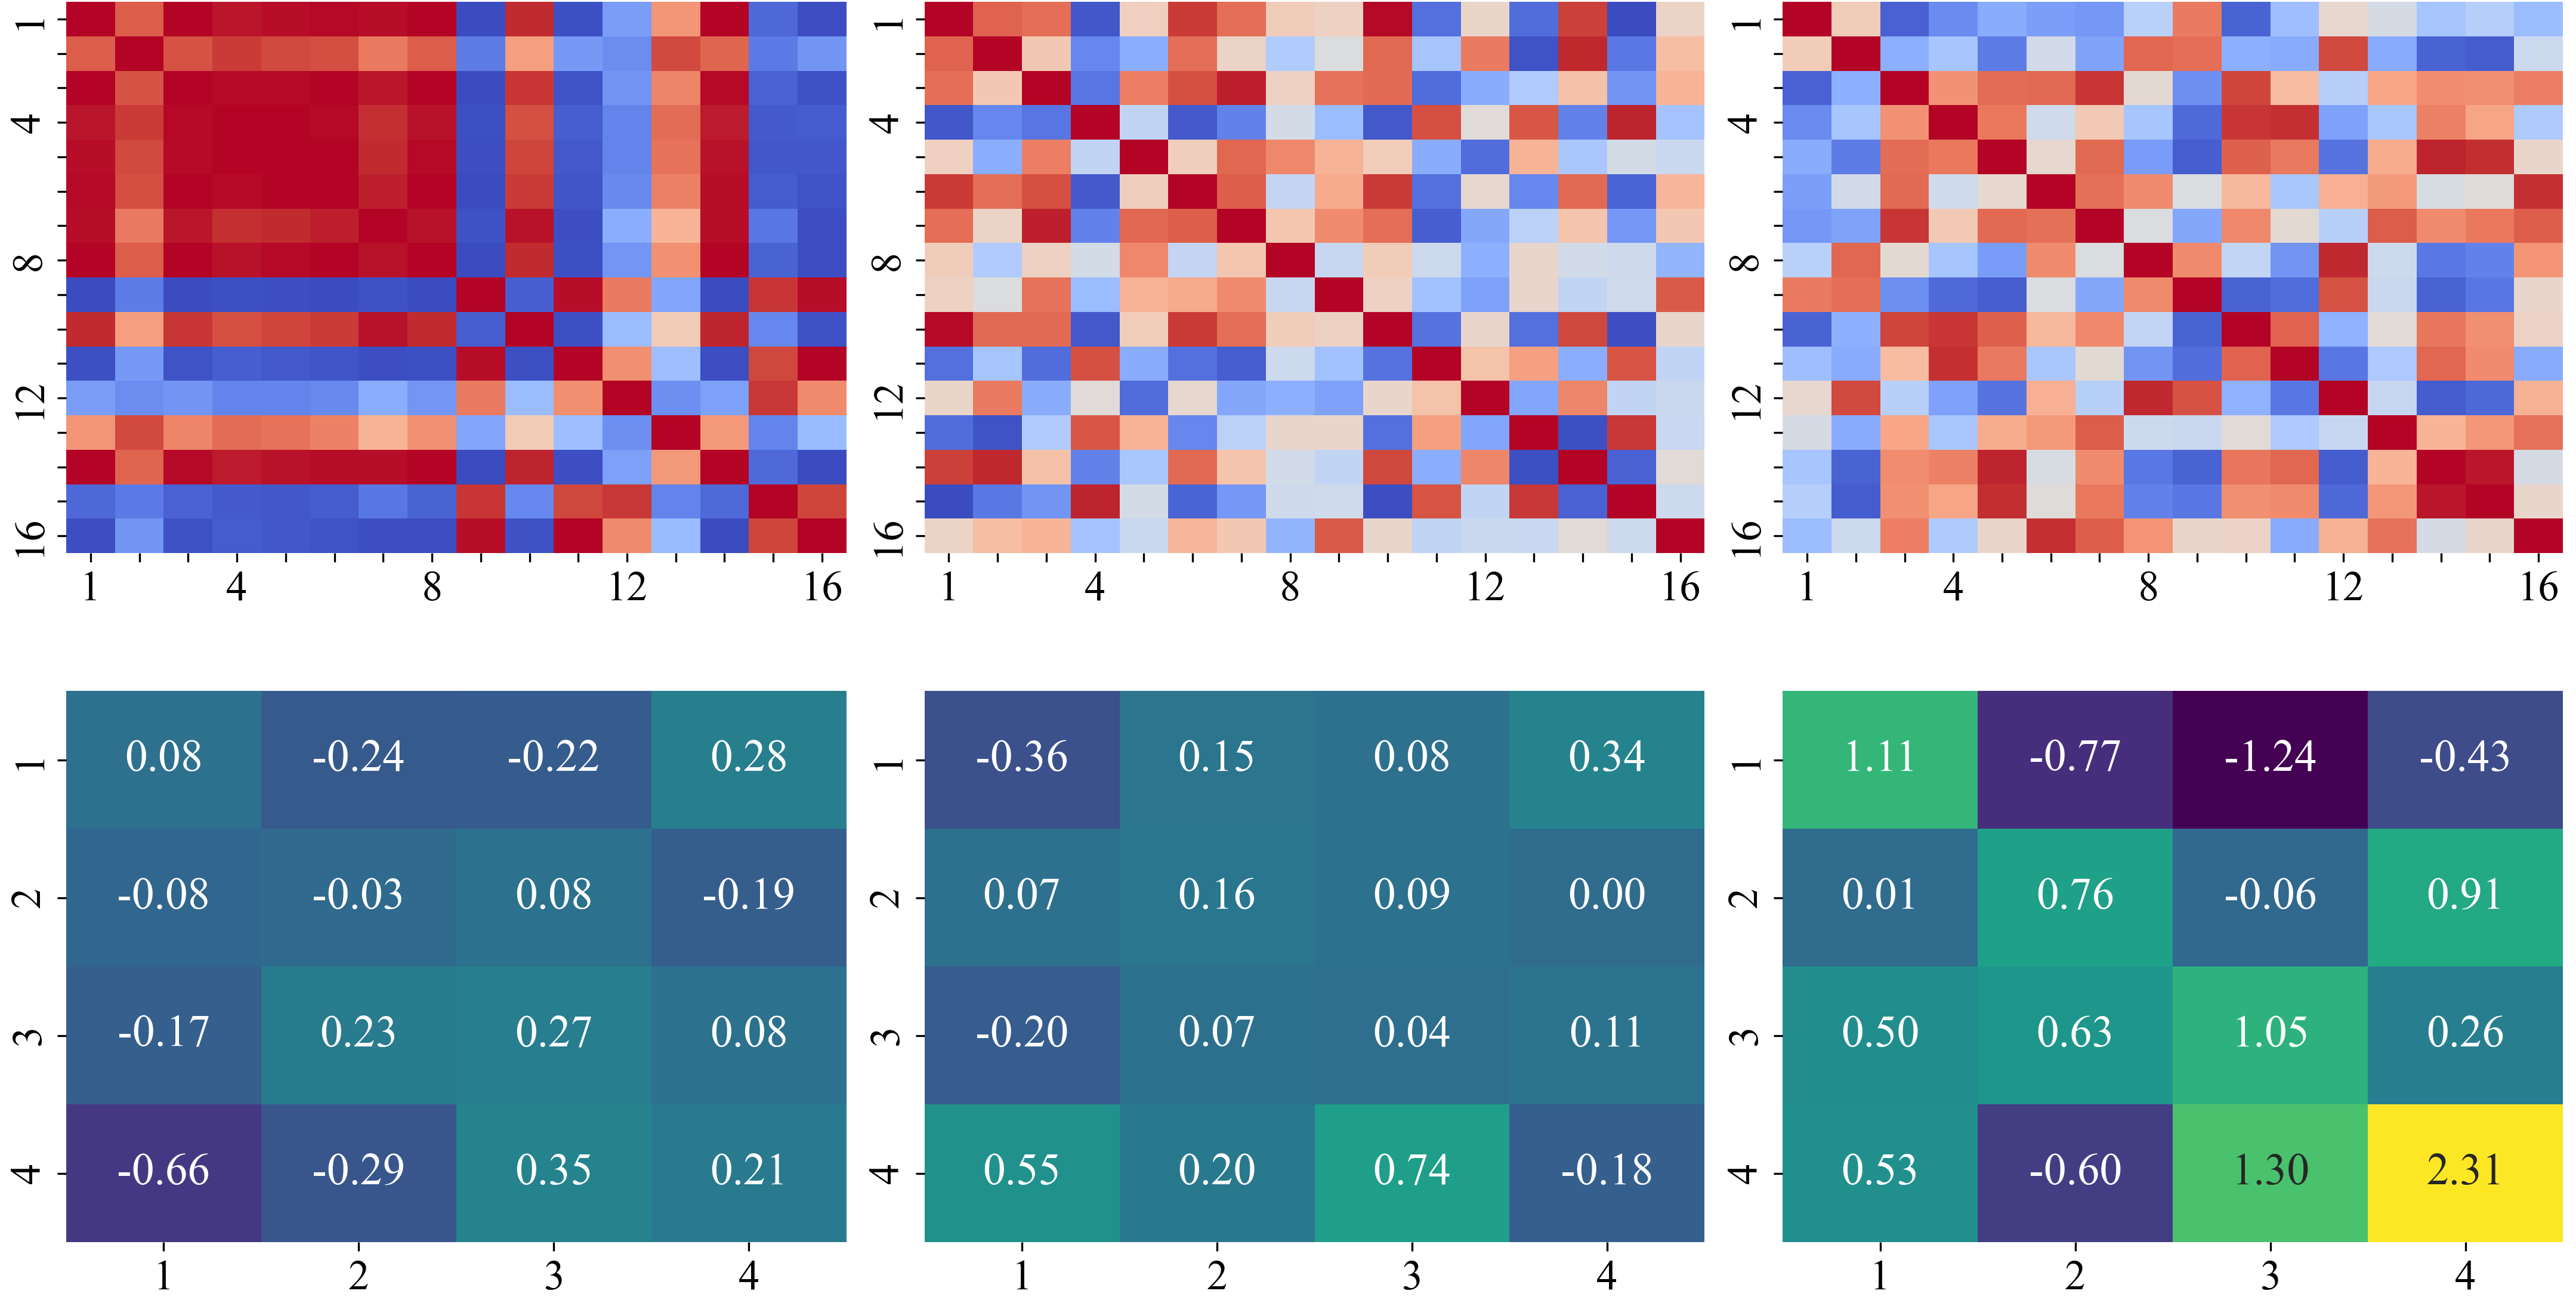} 
\vspace{-5pt}
\caption{Feature evolution across fusion stages on BTH.} %Top: channel-wise correlation matrices show progressive decorrelation and structure emergence. Bottom: local activation maps illustrate increasing sparsity and semantic focus.}
\label{fusionfinBTH}
\end{figure}

\begin{figure}[!ht]
\centering
\includegraphics[width=0.99\columnwidth]{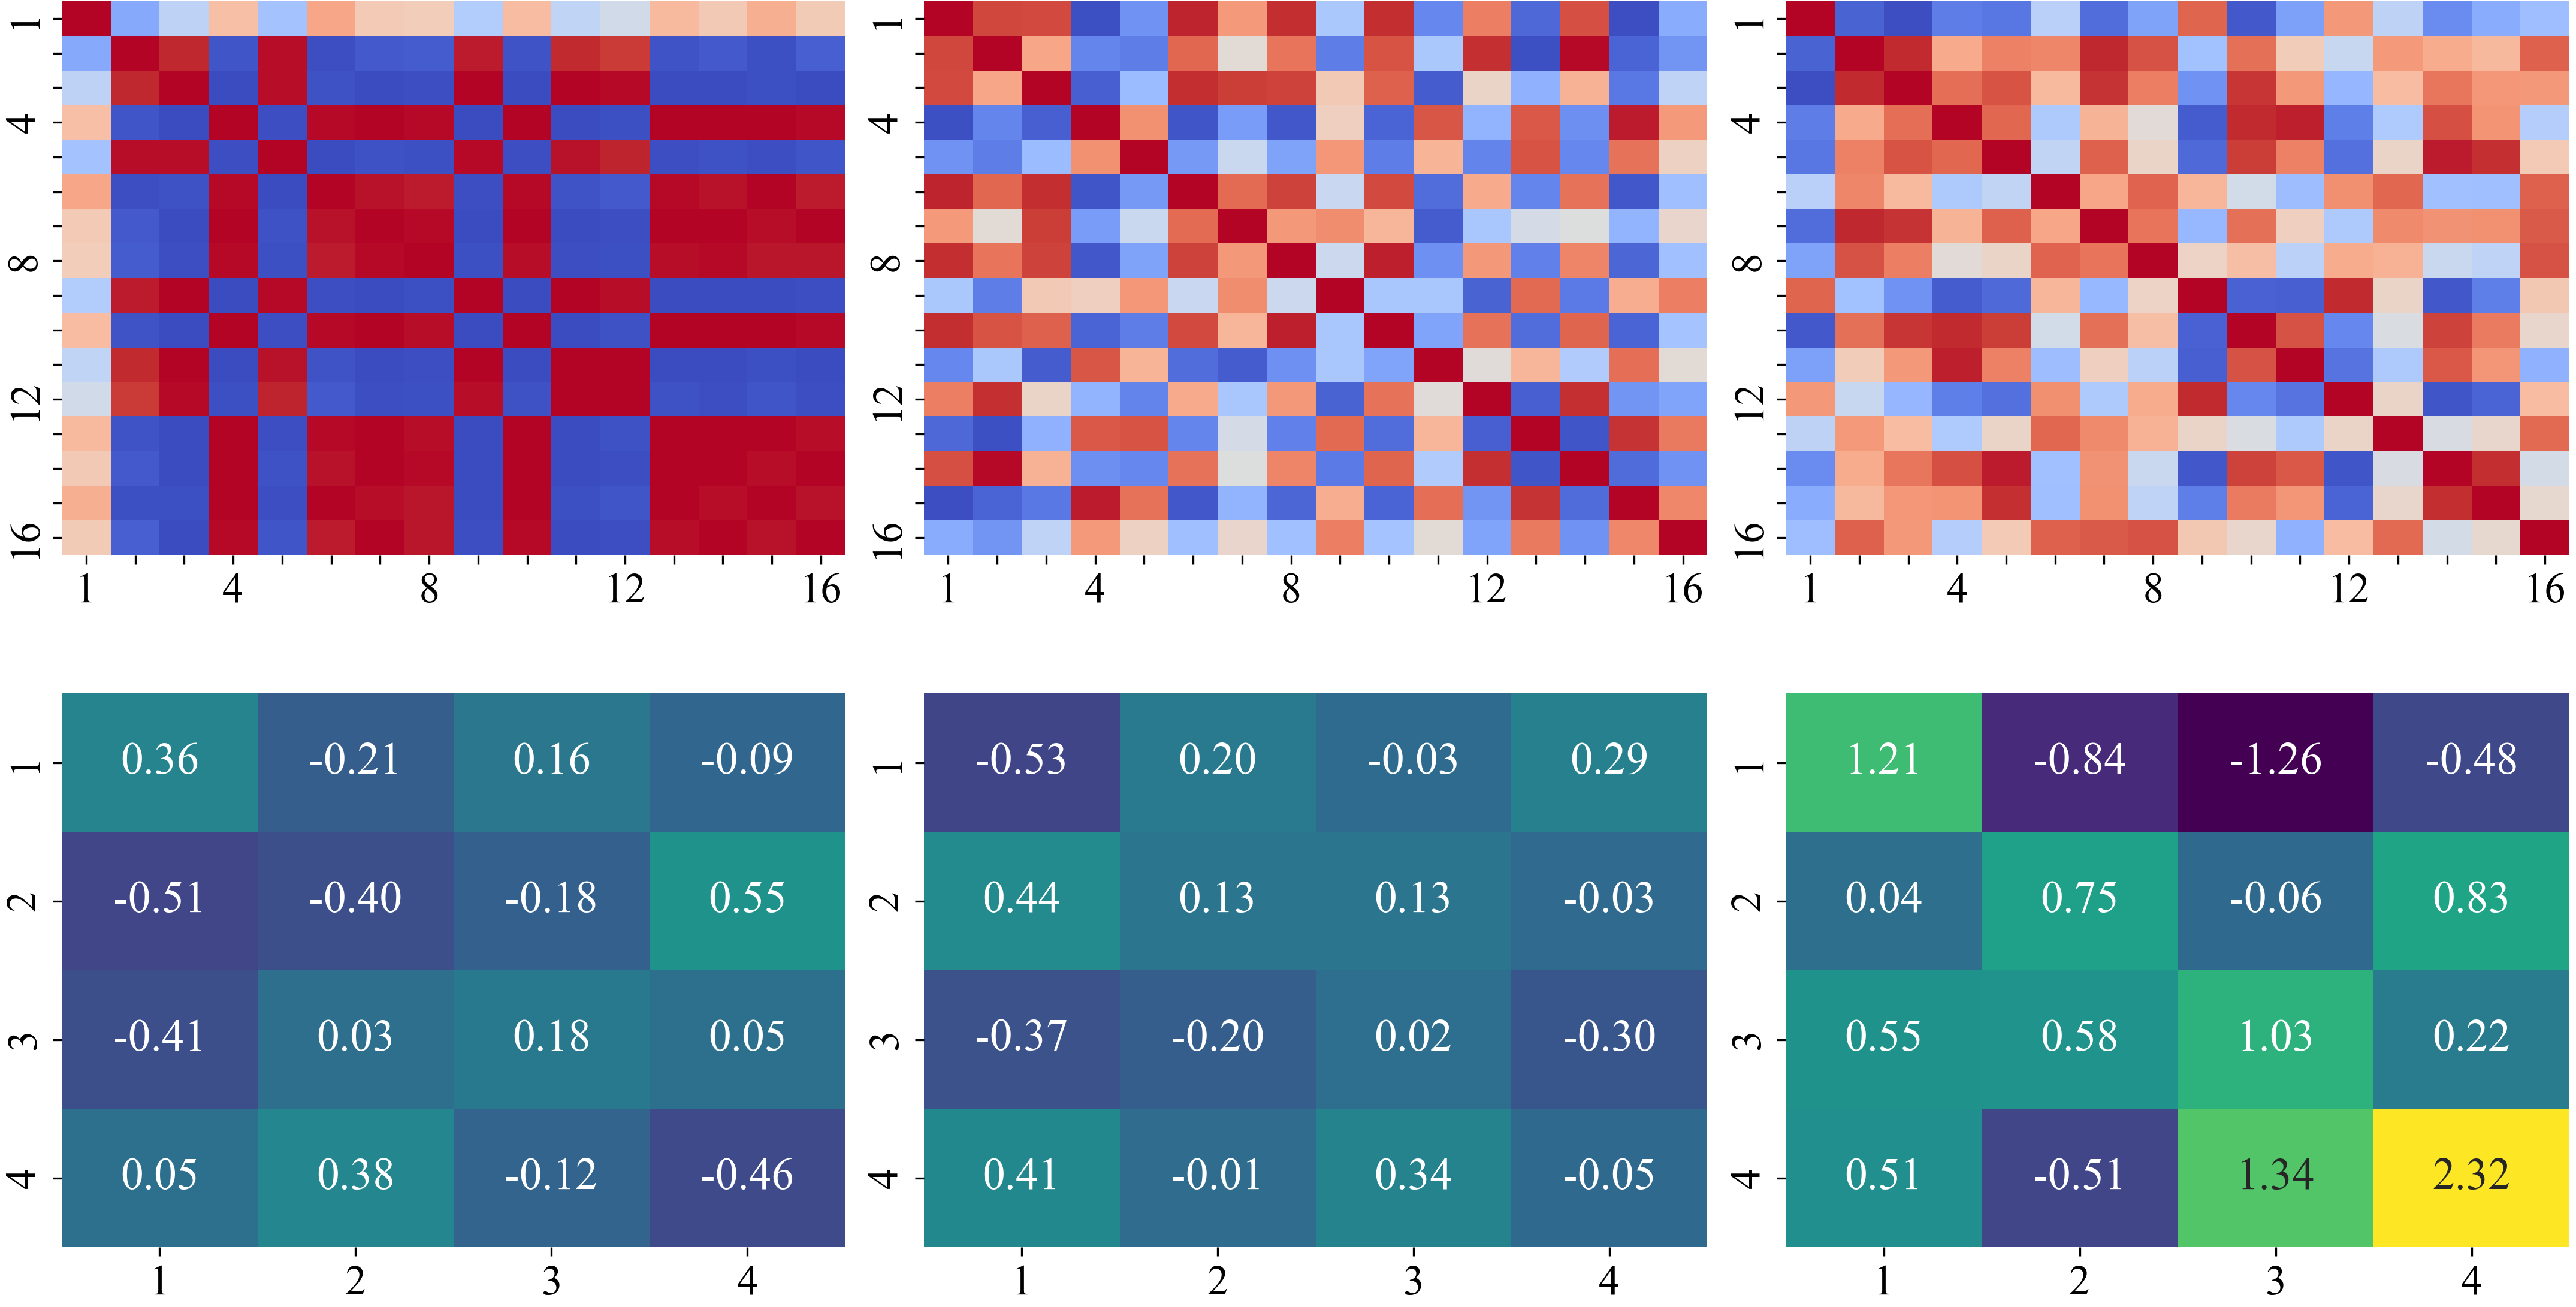} 
\vspace{-5pt}
\caption{Feature evolution across fusion stages on Ala.} %Top: channel-wise correlation matrices show progressive decorrelation and structure emergence. Bottom: local activation maps illustrate increasing sparsity and semantic focus.}
\label{fusionfinAla}
\end{figure}

\begin{comment}
%多模态比较放这里
\begin{table*}
\centering
\caption{Comparison of fusion results of MBT, LMF, TFN, and CMLIP}
\label{Comp_fusion}
\tabcolsep=0.28cm
\setlength{\tabcolsep}{2pt}\begin{tabular}{cccccccccc}
\midrule[0.5pt]
\multirow{2}{*}{Models} & \multicolumn{3}{c}{128 Steps}  & \multicolumn{3}{c}{256 Steps}    & \multicolumn{3}{c}{384 Steps}    \\ \cmidrule(r){2-4}  \cmidrule(r){5-7} \cmidrule(r){8-10}  
 &{MSE}   & MAE  &Prediction Time   & MSE   &{MAE}  &Prediction Time   &{MSE}   & MAE  &Prediction Time   \\ \midrule[0.5pt]
MBT     &0.472$\pm$0.008  &0.491$\pm$0.011 &60.223$\pm$2.781  &0.682$\pm$0.016  &0.628$\pm$0.025  &61.452$\pm$1.340  &0.786$\pm$0.029  &0.679$\pm$0.040  &59.145$\pm$2.768 \\  
LMF     &0.468$\pm$0.013  &0.487$\pm$0.022 &73.259$\pm$2.655  &0.670$\pm$0.035  &0.627$\pm$0.036  &70.447$\pm$3.121  &0.832$\pm$0.047  &0.707$\pm$0.041  &71.878$\pm$2.546                         \\  
TFN     &0.509$\pm$0.010  &0.522$\pm$0.003 &75.354$\pm$1.139  &0.667$\pm$0.029  &0.614$\pm$0.025  &72.877$\pm$1.348  &0.831$\pm$0.033  &0.678$\pm$0.025  &74.583$\pm$1.054                            \\   
\textbf{CMLIP}  &\textbf{0.442$\pm3.51\times10^{-7}$}  &\textbf{0.472$\pm1.49\times10^{-7}$} &\textbf{57.567}$\pm$2.718 & {\textbf{0.645}$\pm$0.045}  & \textbf{0.605}$\pm$0.019 &\textbf{54.661}$\pm$2.820 & {\textbf{0.742}$\pm$0.025}   &\textbf{0.650}$\pm$0.008      &\textbf{43.457}$\pm$0.127                             \\   \midrule[0.5pt]
\end{tabular}
\end{table*}
\end{comment}

\bigskip

\bibliographystyle{aaai}
\bibliography{ref}

\end{document}
